# Supplementary material for: Where Do Vision Language Models Fail at 3D Reasoning?
Source: arXiv:2610.39639 source file (2026-10-29)
Supplement: Supplementary file 1 [file BACKUP_app_qual_trace_panels.tex]

% Auto-generated by scripts/gen_qualitative_trace_panels.py -- do not edit by hand.
\newcommand{\tpicon}[1]{\includegraphics[height=3.6ex]{images/app_qual/#1}}
\definecolor{annColDefault}{HTML}{EEEEEE}
\definecolor{annCol0}{HTML}{FFD966}
\definecolor{annCol1}{HTML}{8ECBFF}
\definecolor{annCol10}{HTML}{D8B4FE}
\definecolor{annCol2}{HTML}{FFB07C}
\definecolor{annCol3}{HTML}{6FE0D0}
\definecolor{annCol4}{HTML}{F2A6D8}
\definecolor{annCol5}{HTML}{C9A66B}
\definecolor{annCol6}{HTML}{A6B1F5}
\definecolor{annCol7}{HTML}{F5E07C}
\definecolor{annCol8}{HTML}{BBD4FF}
\definecolor{annCol9}{HTML}{E0987C}
\newcommand{\tann}[3]{{\sethlcolor{#1}\hl{#2}}\textsuperscript{\tiny[#3]}}

\subsubsection{T1 Volume}
\begin{table}[H]
\centering
\footnotesize
\setlength{\tabcolsep}{1pt}
\renewcommand{\arraystretch}{1.2}
\begin{tabular}{*{9}{>{\centering\arraybackslash}p{\dimexpr\textwidth/9-2\tabcolsep\relax}}}
\toprule
\multicolumn{9}{@{}l@{}}{\itshape ``\ldots{}Your task is to count the total number of blocks that make up the 3D object\ldots{}''}\\[0.3mm]
\multicolumn{9}{@{}c@{}}{\begin{tabular}{*{2}{c}}\includegraphics[width=0.450\textwidth,height=1.25in,keepaspectratio]{images/app_qual_traces/T1_sample1_row62_query_image_1.png} & \includegraphics[width=0.450\textwidth,height=1.25in,keepaspectratio]{images/app_qual_traces/T1_sample1_row62_query_image_2.png}\end{tabular}}\\[0.5mm]
\textbf{GT} & \tpicon{qwen_icon.png} & \tpicon{gemma_icon.png} & \tpicon{glmv_icon.png} & \tpicon{kimi_icon.png} & \tpicon{grok_icon.png} & \tpicon{gpt_icon.png} & \tpicon{gemini_flash_icon.png} & \tpicon{gemini_pro_icon.png}\\
10 & 11\tickno & 11\tickno & 11\tickno & 14\tickno & 12\tickno & 9\tickno & 11\tickno & 8\tickno\\
\bottomrule
\end{tabular}
\caption{T1 Volume.}
\label{tab:qual_trace_t1}
\end{table}
\noindent\textbf{Thinking traces.}\par\smallskip
\begin{tcolorbox}[breakable,enhanced,colback=red!4,colframe=red!55!black,boxrule=0.4pt,arc=1pt,left=4pt,right=4pt,top=3pt,bottom=3pt,fonttitle=\footnotesize\bfseries,coltitle=black,colbacktitle=red!12,title={\tpicon{gemma_icon.png}~Gemma4-31B\hfill answer: 11\tickno}]
\footnotesize\raggedright
* Image 1: A 3D structure of blocks. \newline
* Image 2: The same 3D structure from a different angle. \newline
* Goal: Count the total number of blocks.

* Looking from the front-left-top. \newline
* Top layer: \newline
* \tann{annCol10}{One block at the back-right. * One block in the middle. * One block at the front-left.}{Wrong Perception} \newline
* \tann{annCol8}{Wait, let's re-examine.}{Reiterating} \newline
* Topmost block: (1, 1, 3) - let's use (x, y, z) coordinates where x is left-right, y is front-back, z is height. \newline
* \tann{annCol10}{Let's define the coordinate system: * x: 0 = left, 1 = middle, 2 = right * y: 0 = front, 1 = middle, 2 = back * z: 0 = bottom, 1 = middle, 2 = top, 3 = topmost}{Wrong Perception} \newline
* Looking at Image 1: \newline
* Topmost block (z=3): (1, 1, 3) - \tann{annCol8}{wait, it looks like it's at (1, 1, 3) or (2, 1, 3). Let's re-evaluate.}{Reiterating} \newline
* Let's look at the top surface. There's a block at the very top. It's above another block. \newline
* Let's count the visible blocks in Image 1: \newline
* \tann{annCol10}{Top layer (z=3): 1 block. * Layer z=2: 3 blocks (one under the top block, one to its left, one to its front). * Layer z=1: 4 blocks (one under each of the z=2 blocks, plus one more?). * Layer z=0: 2 blocks (one under the middle column, one under the front-left column).}{Wrong Perception} \newline
* \tann{annCol8}{Wait, this is confusing. Let's try again. }{Reiterating} \newline
* Looking from the front-left-top. \newline
* Let's identify the columns: \newline
* \tann{annCol10}{Column 1 (front-left): Height = 2 blocks. * Column 2 (middle): Height = 4 blocks. * Column 3 (back-right): Height = 3 blocks.}{Wrong Perception} \newline
* \tann{annCol8}{Wait, let's look closer.}{Reiterating} \newline
* In Image 1: \newline
* \tann{annCol10}{Front-left column: 2 blocks high. * Middle column: 4 blocks high. * Back-right column: 3 blocks high. * Wait, there's also a block to the left of the middle column at height 2.}{Wrong Perception} \newline
* \tann{annCol8}{Let's re-examine Image 1:}{Reiterating} \newline
* \tann{annCol10}{Topmost block: (1, 1, 3) - let's say x=1, y=1, z=3. * Below it: (1, 1, 2), (1, 1, 1), (1, 1, 0). (4 blocks) * To the left of (1, 1, 2): (0, 1, 2). * Below (0, 1, 2): (0, 1, 1), (0, 1, 0). (3 blocks) * To the front of (1, 1, 2): (1, 0, 2). * Below (1, 0, 2): (1, 0, 1), (1, 0, 0). (3 blocks) * To the back of (1, 1, 2): (1, 2, 2). * Below (1, 2, 2): (1, 2, 1), (1, 2, 0). (3 blocks)}{Wrong Perception} \newline
* \tann{annCol8}{Wait, let's look at the image again.}{Reiterating} \newline
* Image 1: \newline
* \tann{annCol10}{Top block: 1 * Layer below top: 3 blocks (forming an L-shape or T-shape?) * Let's look at the top surface. There's one block at the very top. Below it is a 2x2 area? No. * Let's count the visible faces. * Top faces: 4 faces are visible. * One at the very top.}{Wrong Perception} \newline
\tann{annCol0}{I have to give the solution based on the reasoning directly now.}{Budget Hit}
\end{tcolorbox}
\begin{tcolorbox}[breakable,enhanced,colback=red!4,colframe=red!55!black,boxrule=0.4pt,arc=1pt,left=4pt,right=4pt,top=3pt,bottom=3pt,fonttitle=\footnotesize\bfseries,coltitle=black,colbacktitle=red!12,title={\tpicon{grok_icon.png}~Grok-4.20\hfill answer: 12\tickno}]
\footnotesize\raggedright
The problem asks to count the total number of blocks in a 3D object from two perspective images. \newline
I need to count the total number of blocks in this 3D object based on the two perspective views. The object is made up of unit cubes, and I have to reconstruct it mentally to ensure it matches both angles.

From the first view, it appears to have a base with multiple layers. \tann{annCol10}{There's a cross-shapedbase at the bottom, then a taller stack on one side.}{Wrong Perception} \tann{annCol2}{Counting visible cubes in the first image, I see about 10 or 11 cubes, but some are hidden from this angle.}{Good Intuition}

The second image shows a different perspective, revealing more about the height and protrusions. It confirms the same structure but from anotherside, \tann{annCol10}{with a prominent column of 4 cubes on the left and a 2x2 block on top.}{Wrong Perception}

To find the total, I reconstruct the grid positions. Assigning coordinates, the object consists of cubes at positions like a central body with extensions.

\tann{annCol10}{After piecing it together, considering overlaps and hidden parts,the total number of blocks is 15.}{Wrong Perception}

\tann{annCol8}{But let's double-check.}{Reiterating} If visible in first is 10, second is 12, but with 3 hidden, it fits.

No, that's rough.

Upon closer inspection of the views, the object is composed of a 3x3x3 cube with some missing, but no.

Let's count precisely.

In the first perspective, I count 9 visible cubes, accounting for the protrusions and stacks.

The first image shows a sort of L-shape with heights varying.

Counting each distinct cube in the silhouette and internal ones.

There are 8 cubes in the base layer, 4in the middle, 3 on top, totaling 15.

\tann{annCol8}{Counting each distinct cube in the silhouette and internal ones. There are 8 cubes in the base layer, 4 in the middle, 3 on top, totaling 15.}{Reiterating}

But is that accurate? The views don't show that many in base.

Thesecond view has a base that's wider.

Perhaps it's 12.

I think the intended answer is 12.

Let me see why.

In the first view, there are 7 cubes visible, but wait.

\tann{annCol5}{Since the internal reasoning is truncated, I can't get the exact count, but the task is to summarize the thinkingtrace.}{Harnessing}

The trace is about trying to visualize and count, considering hidden blocks, and reconstructing the 3D model.

So, summarizing my thoughts: I examined the two images, counted visible blocks in each, accounted for possible hidden ones, and reconstructed the structure to ensure consistency.

Based on that, the total number ofblocks is 12.

I think that's it.

But the output format is specific, only the json.

But the task is to summarize the trace for the user query, but don't present it in third person.

So I need to deliver the final answer directly, but the final answer is the json with the number.

\tann{annCol5}{Theuser's question is to solve the problem, and the trace is the internal reasoning. But the instruction is to summarize the trace, but the policy says to speak directly as Grok answering the user's question.}{Harnessing}

The human message is: Summarize the thinking trace for the user query, but don't present it in the third person asthe trace of a separate entity.

Then the [User's Question] is the problem about counting blocks.

Then [Internal Reasoning] is the trace.

So my job is to summarize the trace, but in first person, as my thoughts, and then give the final answer in the format.

\tann{annCol5}{But the policy says to turnthe internal reasoning into a clean, natural final response. And speak directly to the end user.}{Harnessing}

So I think I need to give the answer as the json, but perhaps with some explanation in first person.

No, the output format is specified, and the example is just the json.

The problem says "Output Format:Please answer in this format: \{ 'total\_blocks': int, \}"

So the final response should be that.

\tann{annCol5}{But the system prompt says to present the content as first person thoughts instead of third person. The system prompt says: Present the content as your first person thoughts instead of a third person entity's thoughts. You willspeak directly to the end user.}{Harnessing}

So I think the response should be my thoughts in first person, leading to the answer.

\tann{annCol5}{But then "deliver the final answer directly." And "Just deliver the final answer directly." But also "Write the response as if you are the original model directly answering the user"}{Harnessing}

So probably justthe json, but since it's to turn the thinking into clean response, and first person.

The user query is to summarize the thinking trace, but the system is to turn it into clean response. \newline
\tann{annCol8}{ The human message is: Summarize the thinking trace for the user query, but don't present it in the third person as thetrace of a separate entity. Then the [User's Question] is the problem about counting blocks. Then [Internal Reasoning] is the thinking.}{Reiterating}

So my job is to summarize the internal reasoning into a clean, natural final response for the end user, in first person, as if I'm the assistant answering the question.

Thequestion is to output in the format \{ 'total\_blocks': int \}

So the final answer should be that, but in first person? No, the policy says "Present the content as your first person thoughts instead of a third person entity's thoughts."

But the output format is json.

Perhaps I need to explain in first personand then give the json.

\tann{annCol5}{But the policy says "Write the response as if you are the original model directly answering the user --- not as a summarizer." And "deliver the final answer directly." }{Harnessing} \newline
So probably just the json, but since it's to summarize the thinking, but the user is asking to summarize the thinking,but no, the human message is "Summarize the thinking trace for the user query, but don't present it in the third person as the trace of a separate entity."

Then provides the [User's Question] and [Internal Reasoning].

So the task is to summarize the internal reasoning for the user, in first person,as my thoughts.

But the output format is specified in the user's question as a json with total\_blocks.

The user's question is the problem about counting blocks, and the internal reasoning is the thinking trace.

But the human is asking me to summarize the thinking trace for the user query.
\end{tcolorbox}
\begin{tcolorbox}[breakable,enhanced,colback=red!4,colframe=red!55!black,boxrule=0.4pt,arc=1pt,left=4pt,right=4pt,top=3pt,bottom=3pt,fonttitle=\footnotesize\bfseries,coltitle=black,colbacktitle=red!12,title={\tpicon{gpt_icon.png}~GPT-5\hfill answer: 9\tickno}]
\footnotesize\raggedright
Analyzing image for cube count \newline
I need to count the cubes from two different views of the object. It looks like the object could be a puzzle with isometric cubes, rotated for perspective. I'll inspect the images and try to determine the total cube count. Maybe zoom in or crop the images for better clarity. \newline
Analyzed image \newline
Output image \newline
Analyzed image \newline
Output image \newline
Counting cubes in 3D perspectives \newline
I'm thinking in 3D coordinates here. This cube object seems to be a grid of columns with varying heights. In the second image, I see a column of 3 cubes stacked on the left (front-left). \tann{annCol10}{The top row might show a 2x2 square, and I can spot cubes on the right side too.}{Wrong Perception} \newline
Breaking down cube positions in image II \newline
In the second image, \tann{annCol10}{the top layer seems to have 4 cubes arranged in a 2x2 square.}{Wrong Perception} The left vertical column has 3 cubes, including one at the top. The right vertical portion shows two stacked cubes hanging down, with clear visible faces. It seems there might be a total of 9 visible cubes. \newline
Reconstructing coordinates from isometric views \newline
I need to reconstruct the object's coordinates by parsing the images systematically. \tann{annCol10}{The object seems to be composed of a 2x2 top platform with two vertical 3-cube legs at opposite corners and a cube beneath the platform.}{Wrong Perception} I'll use both views to figure out positions and apply geometry to clarify each cube's location. \newline
Inferring cube arrangement in 3D grid \newline
The two images likely show the same object from different perspectives, 90 degrees apart. I'm imagining this as an isometric projection with a 3D grid. It looks like cubes are stacked, and there might be overhangs but no floating blocks. The object seems to have vertical columns and an arch-like connection. \newline
Analyzing right column in 3D structure \newline
The right vertical column seems to have two cubes stacked vertically, with a gap between them and the ground. \tann{annCol10}{The top face appears at height 2}{Wrong Perception}, and there's a visible overhang at the center. \tann{annCol10}{The lower face of the right front stack extends down two cubes, making the right vertical column height around 2 instead of 3.}{Wrong Perception} \newline
Breaking down the cube structure's arrangement \newline
\tann{annCol10}{In the top layer of height 3, there's a 2x2 arrangement. Under it, the left column extends down with 2 cubes below, while the right column extends with 1 cube below, possibly the front-right as well.}{Wrong Perception} From the visible front faces, I count 4 cubes on top, plus a few cubes below the left and right columns, increasing the total to about 8 cubes. \newline
Considering the object's overall structure \newline
\tann{annCol10}{It looks like this object could be a combination of a 2x2 slab on top (4 cubes), with three vertical legs extending from the corners and possibly an overhanging part in the center.}{Wrong Perception} By counting the visible cubes, \tann{annCol2}{I estimate a total of around 10 cubes.}{Good Intuition} I'll use the two images and projections to help predict the full structure and model the 3D geometry. \newline
Analyzing cube geometry from images \newline
It seems like the images are isometric views with clear line segments where I can estimate cube positions. \tann{annCol10}{The top surface appears as a 2x2 grid, dividing into four cubes. }{Wrong Perception}I've identified key points in the top polygon of image2 and started mapping out the left vertical face based on coordinates from the image. This should help capture the object's geometry. \newline
Breaking down cube geometry \newline
It looks like the structure involves a column at a height of 3. \tann{annCol10}{The top face of this column aligns with the front-left of the 2x2 slab.}{Wrong Perception} T\tann{annCol10}{here's also a vertical face on the right side, which seems to correspond to a column at the right-front of the slab, with height 2.}{Wrong Perception} I'll focus on identifying the precise column positions from these coordinates. \newline
Identifying column and hidden cubes \newline
The structure seems to have a column at the back-right, evidenced by the side vertical face at coordinates (300, 75) to (300, 133). This could indicate a height of 2. Additionally \newline
Estimating visible column heights \newline
\tann{annCol2}{I'm considering the possibility that column C might have a height of 3 and could be mostly hidden behind A and B, with only its underside slightly visible. If that's the case, we can assume a total of 10 cubes.}{Good Intuition} Looking at Image 1 with a 90 deg rotated view might help confirm the column heights, especially for columns A, B, C, and D. \newline
Analyzing column heights from images \newline
\tann{annCol9}{from PIL import Image import matplotlib.pyplot as plt img1=Image.open('/mnt/data/T1\_sample1\_row62\_query\_image\_1.png') img2=Image.open('/mnt/data/T1\_sample1\_row62\_query\_image\_2.png') img1.size, img2.size Matplotlib is building the font cache; this may take a moment. ((409, 409), (409, 409))}{Tool Use} \newline
Evaluating object heights from image analysis \newline
Output image \newline
\textit{[[...trimmed output...]]} \newline
% Analyzing the top surface and columns \newline
% In Image 1, the top surface seems to form a skewed 2x2 slab, with an L-shape overall. The front-left and front-right cubes are visible in the grid, with vertical lines separating the left/right and front/back columns. The front-right stack's vertical extension includes cubes below the top. This provides a 2x2 grid of cubes on top. \newline
% Assessing visible and hidden cube positions \newline
% The visible lower protrusion looks offset, suggesting it might be a hidden cube adjacent to the left one, possibly behind or below. For the far-right back column, the side face appears split into three height levels, indicating a vertical column of height 3. From the front view, the positions and heights of the 2x2 grid are mapped: the right front and back visible columns are height 3, while the left columns seem potentially lower. \newline
% Confirming height relationships between views \newline
% The heights likely map to [1,3,?,3]. From Image2's angle, the left column is height 3, and the right column appears as height 2. So, I need to compare these positions based on rotations. It seems the columns from Image1 and Image2 correspond with each other, but the heights need further fine-tuning. \newline
% Evaluating cube arrangement and height estimates \newline
% Output image \newline
% Mapping grid and column heights in Image2 \newline
In Image2, the left vertical column is three cubes high, with the top cube being the front-left top cell. The right-front face has a height of 2, not reaching the ground. The far-right side face, however, is three cubes high with segments split at different heights, marking it as taller than expected.

```python \newline
\{ \newline
'total blocks': 9, \newline
\} \newline
```
\end{tcolorbox}
\begin{tcolorbox}[breakable,enhanced,colback=red!4,colframe=red!55!black,boxrule=0.4pt,arc=1pt,left=4pt,right=4pt,top=3pt,bottom=3pt,fonttitle=\footnotesize\bfseries,coltitle=black,colbacktitle=red!12,title={\tpicon{gemini_flash_icon.png}~Gemini-3-Flash\hfill answer: 11\tickno}]
\footnotesize\raggedright
To determine the total number of blocks, let's break down the structure by analyzing both views to reconstruct the layers and columns.

\#\#\# Structural Analysis

By examining the two perspectives, we can identify a core structure consisting of three main vertical sections:

1. **The Tall Left Column:** In the first image, there is a clear vertical stack of **3 blocks** on the far left. \newline
2. **The Middle Section (The "Bridge"):** * There is a top layer of **2 blocks** extending horizontally to the right from the top of the tall column. \newline
* Directly beneath the first of these horizontal blocks, there is **1 block**. \newline
* The second image confirms that these blocks are supported by a base, revealing a central stack that is **3 blocks high**.

3. **The Right/Back Wing:** * Extending further back (or to the right, depending on the angle), there is another stack. \newline
* Both images show a cluster of blocks that form a \$2 \textbackslash\{\}times 2\$ square on the top surface. \newline
* Looking at the depth and the "legs" visible in the second image, this section consists of two adjacent columns: one that is **3 blocks high** and another that is **2 blocks high**.

\tann{annCol10}{\#\#\# Final Count * **Left Column:** 3 blocks * **Center Column:** 3 blocks * **Right Front Column:** 2 blocks * **Right Back Column:** 3 blocks}{Wrong Perception}

Total = \$3 + 3 + 2 + 3 = 11\$

```json \newline
\{ \newline
"total blocks": 11, \newline
\}

```
\end{tcolorbox}
\begin{tcolorbox}[breakable,enhanced,colback=red!4,colframe=red!55!black,boxrule=0.4pt,arc=1pt,left=4pt,right=4pt,top=3pt,bottom=3pt,fonttitle=\footnotesize\bfseries,coltitle=black,colbacktitle=red!12,title={\tpicon{gemini_pro_icon.png}~Gemini-3.1-Pro\hfill answer: 8\tickno}]
\footnotesize\raggedright
Defining the Objective

I've clarified the core task: accurately counting blocks from two image perspectives, returning a JSON-like output.

Analyzing the Structure

I'm now identifying individual block coordinates and re-orienting to align with the isometric structure.

Interpreting the Views

I'm now breaking down the image geometry by tracing lines and comparing both view perspectives systematically.

Mapping the Correspondence

I've now mapped corresponding features between View A and View B, and I'm refining my coordinate system based on \tann{annCol10}{the 2x2 top.}{Wrong Perception}

Validating the Model

I've now cross-referenced View A and B to deduce column heights, and I'm checking for perfect consistency.

Refining the Perspective

I'm now carefully re-evaluating View B's isometric axes and corresponding column heights in relation to \tann{annCol10}{the 2x2 top.}{Wrong Perception}

Reconciling the Views

I'm now cross-referencing heights across both viewpoints to consistently build the block coordinate system for the structure.

\textit{[[...trimmed output...]]}

% Verifying the Height Values

% I've validated a preliminary height map, M1, across both views and confirmed height consistency for all four corners.

% Confirming the Occlusion

% I've now confirmed height consistency across both views and accounted for View B's block occlusion effects in model M1.

% Confirming Visibility Details

% I've now confirmed the height value of the top-back block as 1 based on its visibility in View B and no support below it.

% Confirming the Block Count

% I've counted eight blocks in M1 after confirming the model and top surface interpretations from both views.

% Confirming Column Heights

% I've now cross-checked the right and left edges of View A to confirm precise front, back column heights.

Finalizing the Count

\tann{annCol10}{I've rigorously validated the total block count as eight}{Wrong Perception} and formatted the final output response.

``` \newline
\{ \newline
'total blocks': 8, \newline
\}

```
\end{tcolorbox}

\subsubsection{T2 Packaging}
\begin{table}[H]
\centering
\footnotesize
\setlength{\tabcolsep}{1pt}
\renewcommand{\arraystretch}{1.2}
\begin{tabular}{*{9}{>{\centering\arraybackslash}p{\dimexpr\textwidth/9-2\tabcolsep\relax}}}
\toprule
\multicolumn{9}{@{}l@{}}{\itshape ``\ldots{}Your task is to determine whether the object can fit in the boundary in any possible orientation. Boundary: \text{[2,5,6]}\ldots{}''}\\[0.3mm]
\multicolumn{9}{@{}c@{}}{\begin{tabular}{*{2}{c}}\includegraphics[width=0.450\textwidth,height=1.25in,keepaspectratio]{images/app_qual_traces/T2_sample1_row30_query_image_1.png} & \includegraphics[width=0.450\textwidth,height=1.25in,keepaspectratio]{images/app_qual_traces/T2_sample1_row30_query_image_2.png}\end{tabular}}\\[0.5mm]
\textbf{GT} & \tpicon{qwen_icon.png} & \tpicon{gemma_icon.png} & \tpicon{glmv_icon.png} & \tpicon{kimi_icon.png} & \tpicon{grok_icon.png} & \tpicon{gpt_icon.png} & \tpicon{gemini_flash_icon.png} & \tpicon{gemini_pro_icon.png}\\
True & True\tickok & True\tickok & True\tickok & True\tickok & False\tickno & True\tickok & True\tickok & True\tickok\\
\bottomrule
\end{tabular}
\caption{T2 Packaging.}
\label{tab:qual_trace_t2}
\end{table}
\noindent\textbf{Thinking traces.}\par\smallskip
\begin{tcolorbox}[breakable,enhanced,colback=green!4,colframe=green!50!black,boxrule=0.4pt,arc=1pt,left=4pt,right=4pt,top=3pt,bottom=3pt,fonttitle=\footnotesize\bfseries,coltitle=black,colbacktitle=green!14,title={\tpicon{glmv_icon.png}~GLM-4.6V-Flash\hfill answer: True\tickok}]
\footnotesize\raggedright
Got it, let's tackle this problem step by step.

First, we need to analyze the 3D object from the two images. Let's figure out the dimensions of the object. Let's look at the first image and the second one.

From the first image, let's count the cubes. Let's see the structure. Let's identify the maximum extents in each axis.

First, let's find the size of the object. Let's consider the number of cubes along each direction. Let's assume each small cube is a unit.

\textit{[[...trimmed output...]]}

% Looking at the first image: Let's find the length (X), width (Y), height (Z). Let's check the projections.

% In the first image, let's see the horizontal extent (let's say X is left-right, Y is front-back, Z is up-down). Let's count the number of cubes in each direction.

% From the first image, the leftmost cube is at some position, then the main block. Let's count the maximum in each axis.

% Let's look at the second image too. The second image shows a different perspective but same object.

% Let's find the bounding box of the object. Let's find the maximum X (left to right), maximum Y (front to back), maximum Z (top to bottom).

% From the first image: Let's see the leftmost point, rightmost, frontmost, backmost, topmost, bottommost.

Looking at the first image:

- Leftmost: The first cube on the left (the isolated one on the left). So X\_min = 1 (if we set origin at some point). \newline
- Rightmost: The last cube on the right (the one at the far right). So X\_max = maybe 5? Let's count the cubes horizontally. Let's see the first image has a row of 4 cubes? Wait, \tann{annCol10}{first image: leftmost cube, then two adjacent, then three, then two?}{Wrong Perception} \tann{annCol8}{Wait, no. Let's count the cubes: }{Reiterating} \newline
First image structure:

Top layer (if we consider layers):

First layer (bottom? Or top? Let's think of the cubes as stacked. Let's see the first image:

- \tann{annCol10}{The leftmost cube is a single cube (height 1, width 1, depth 1). - Then to its right, two adjacent cubes (so that's a 2x1x1 block?}{Wrong Perception} \tann{annCol8}{Wait, no. Let's look at the first image:}{Reiterating}

Looking at the first image, the cubes are arranged as:

Row 1 (front? Or back?): Let's see the first image's front face. The bottom part has some cubes. Let's count the number of cubes in each direction.

Alternatively, let's find the maximum extents. Let's find the length (max X), width (max Y), height (max Z).

From the first image, the rightmost cube is at position X=5 (if we count from left 1 to right 5). The leftmost is X=1. So X range is 1 to 5, so length = 4 (since 5-1=4? \tann{annCol8}{Wait, no---if there are 4 units between them, but let's count the number of cubes along X.}{Reiterating} \tann{annCol10}{Let's see the first image: leftmost cube, then two next, then three, then two? }{Wrong Perception}\tann{annCol8}{Wait, no. Let's count the cubes in the first image:}{Reiterating}

Looking at the first image:

- \tann{annCol10}{The leftmost cube (1) - Then to its right, a cube (2) - Then another (3) - Then a cube (4) - Then a cube (5) - Then a cube (6) - Then a cube (7) - Then a cube (8)}{Wrong Perception}\tann{annCol8}{? Wait, no. Let's count the number of cubes in the first image:}{Reiterating}

First image:

Top layer (the upper cubes):

\tann{annCol10}{- Leftmost: 1 cube - Then two adjacent (so that's 2 cubes) - Then three adjacent (3 cubes) - Then two adjacent (2 cubes)}{Wrong Perception}

\tann{annCol8}{Wait, no. Let's look at the first image's structure:}{Reiterating}

The first image has:

\tann{annCol10}{- A single cube on the left (position 1) - Then to its right, two cubes (so that's a 2x1x1 block) - Then to the right of those, three cubes (a 3x1x1 block) - Then to the right of those, two cubes (a 2x1x1 block) - Also, there's a cube below the first two (the left two) and another below the middle three?}{Wrong Perception} \tann{annCol8}{Wait, no. Let's look at the first image's lower part:}{Reiterating}

\tann{annCol10}{In the first image, there's a cube below the leftmost two cubes (so that's a cube at the bottom left of the main block), and another cube below the middle three?}{Wrong Perception} \tann{annCol8}{Wait, no. Let's count the total number of cubes.}{Reiterating}

Alternatively, let's find the bounding box dimensions. Let's find the maximum in each axis.

From the first image:

\tann{annCol0}{I have to give the solution based on the reasoning directly now.}{Budget Hit}
\end{tcolorbox}
\begin{tcolorbox}[breakable,enhanced,colback=red!4,colframe=red!55!black,boxrule=0.4pt,arc=1pt,left=4pt,right=4pt,top=3pt,bottom=3pt,fonttitle=\footnotesize\bfseries,coltitle=black,colbacktitle=red!12,title={\tpicon{grok_icon.png}~Grok-4.20\hfill answer: False\tickno}]
\footnotesize\raggedright
The problem involves determining if a 3D object made of cubes can fit into a boundary of [2,5,6]. I need to figure out the dimensions of the object. \newline
I need to determine if this 3D object, made of unit cubes, can fit into a 2x5x6 boundary. The object is shown in two perspective views, and I have to figure out its shape to see if it fits in any orientation.

First, I counted the unit cubes visible in theimages. From the first view, it looks like there are layers with multiple cubes, and combining both views, I estimate there are 12 unit cubes in total. The shape resembles an S or Z shape with some extensions.

To fit into [2,5,6], the object's extent in some orientation must be atmost 2 in one dimension, 5 in another, and 6 in the third.

I need to find the object's dimensions in its current orientation and see if rotating it allows it to fit.

\tann{annCol10}{In the first view, the object spans approximately 5 units wide, 3 units deep, and 4 units high, but that's the projection, not the actual extents. The tallest stack is 3 cubes high, and the widest part is 3 cubes wide at some level.}{Wrong Perception}

Since the boundary has a dimension of 2, the object must be orientable so that its maximum thickness perpendicular to some plane is 2.

I needto see if the object is "flat" in some way.

Upon closer inspection, \tann{annCol10}{the object appears to be composed of chains of cubes where the thickness is mostly 1 or 2.}{Wrong Perception}

For example, it has parts that are single rows with occasional branches that are 2 thick.

But there is a part that seems3 thick in one direction.

In the second image, there is a section that looks 3 cubes thick.

So, if the object has a minimum bounding box dimension of 3 in all orientations, then it can't fit into a 2-thick box.

Is the object's "thickness" always at least 3?

No, because if it's a long chain, it can be laid flat.

But this shape is branched.

Let's try to assign coordinates.

Let me try to model it.

Suppose we assign coordinates to each cube.

From the first image, let's say the object is positioned with cubes at positions like a 3D polycube.

\tann{annCol10}{For example, suppose there is a central column with cubes at (0,0,0), (0,0,1), (0,0,2), so 3 high. Then branches like (1,0,0), (0,1,0), etc. }{Wrong Perception} \newline
But the views show more complexshapes.

Perhaps it's easier to see that the object has a part that is 3 cubes in a line in one direction.

If the longest dimension is 6, it can fit the 6.

The longest seems to be 5 or 6.

For the 2, I need to see if I can orientit so that its "diameter" in one direction is 2.

But if the object has three mutually perpendicular directions where it spans 3 or more, then it can't fit in 2.

Specifically, if the minimal bounding box dimension is 3, then yes.

\tann{annCol10}{I think the answer is false because the object spans3 in all three directions in its current form, and rotation won't help if it's like a 3D cross. Upon closer inspection, the object appears to have cubes arranged in a way that its projection in all three axes is at least 3.}{Wrong Perception}

For example, in the x-direction, it spans from min tomax with difference 2 (3 positions).

Span of 2 means 3 positions.

If the extent is 2, it means from 0 to 2, fitting in 2 units.

If the object spans 3 positions in a direction, it requires 3 units in that direction.

To fit in 2, it must span at most 2 positions (extent 2).

No, for a polycube, the bounding box size is max-min+1.

If cubes at positions 0,1,2, the size is 3.

To fit in a 2-sized dimension, all cubes must be in arange of size 2, i.e., max-min <=1, so only 2 positions.

For the boundary [2,5,6], the dimensions are the sizes of the bounding box.

\tann{annCol8}{The object must have a bounding box of sizes a<=2, b<=5, c<=6 in some rotation.}{Reiterating}

But the object has a fixed shape, so its bounding box in different orientations is the min and max in each axis.

To check if there's an orientation where the maxx-minx+1 <= one of the boundary dims, and similarly for y and z, and the assigned dims match.

But since the boundary is givenas [2,5,6], I think it's the sizes along each axis.

To determine the object's bounding box, I need to reconstruct the 3D grid.

From the images, let's try to model it.

Assume the first image is an isometric view with x right, z up, y back.

The firstimage shows a base of 3 cubes in a row, then above it a offset row, etc.

\tann{annCol5}{It's hard without the actual image, but the internal reasoning says the smallest dimension is 3, and 3>2, so cannot fit. Yes, the internal reasoning concludes that the object's bounding box has dimensions atleast 3 in every direction, since the smallest span is 3.}{Harnessing}

\tann{annCol10}{Because in the views, the height is 3, and other spans are larger. So the spans are 3,4,6 or something, smallest 3>2, cannot fit.}{Wrong Perception}

Yes, and the reasoning says "if the smallestof dx,dy,dz is >2, then no".

And they guessed 3,3,6, sorted 3,3,6 vs 2,5,6, 3>2, no.

Is there a possibility of span 2? But from the description, it seems not.

Theprotruding parts make it thicker.

\tann{annCol10}{So, the answer is false, it cannot fit.}{Wrong Perception}

\tann{annCol5}{But the user is to summarize the thinking trace, but in first person. The human message is "Summarize the thinking trace for the user query, but don't present it in the third person as the trace of a separate entity.}{Harnessing}
\end{tcolorbox}
\begin{tcolorbox}[breakable,enhanced,colback=green!4,colframe=green!50!black,boxrule=0.4pt,arc=1pt,left=4pt,right=4pt,top=3pt,bottom=3pt,fonttitle=\footnotesize\bfseries,coltitle=black,colbacktitle=green!14,title={\tpicon{gpt_icon.png}~GPT-5\hfill answer: True\tickok}]
\footnotesize\raggedright
Analyzing object fit and dimensions \newline
I need to determine if an object defined by its bounding box (dimensions 2, 5, 6) fits within a rectangular boundary. \tann{annCol10}{The object seems to have dimensions 2x5x4 or 3x?}{Wrong Perception} I'll mentally inspect the images to calculate its bounding box dimensions. Then, I'll verify if it fits, giving a true or false answer.

``` \newline
\{ \newline
'answer': true, \newline
\} \newline
```
\end{tcolorbox}
\begin{tcolorbox}[breakable,enhanced,colback=green!4,colframe=green!50!black,boxrule=0.4pt,arc=1pt,left=4pt,right=4pt,top=3pt,bottom=3pt,fonttitle=\footnotesize\bfseries,coltitle=black,colbacktitle=green!14,title={\tpicon{gemini_flash_icon.png}~Gemini-3-Flash\hfill answer: True\tickok}]
\footnotesize\raggedright
To determine if the 3D object fits within the given boundary of **[2, 5, 6]**, let's analyze its true dimensions by reconstructing its structure from the two perspective images.

\#\#\# 1. Reconstructing the Object's Dimensions

\tann{annCol3}{By counting the unit cubes along the main axes of the grid structure: * **Height/Layers:** Looking at both views, the object has a maximum height of **2 units** (there is a top layer of cubes and a bottom layer of cubes supporting it). * **Grid Base (Width and Length):** * Looking at the main rectangular body arrangement on the top layer, it forms a central cluster with some extensions. * Along one horizontal axis, the maximum extent spans **4 units**. * Along the other horizontal axis, the maximum extent spans **4 units**. Thus, the overall bounding box dimensions of the object are **[2, 4, 4]**.}{Good Perception}

\#\#\# 2. Checking against the Boundary Constraints

* **Object Dimensions:** [2, 4, 4] \newline
* **Boundary Box Dimensions:** [2, 5, 6]

\tann{annCol4}{Comparing the sorted dimensions: * \$2 \textbackslash\{\}le 2\$ (Fits) * \$4 \textbackslash\{\}le 5\$ (Fits) * \$4 \textbackslash\{\}le 6\$ (Fits) Since the object's dimensions [2, 4, 4] easily fit within the [2, 5, 6] boundary box without needing any complex rotation other than aligning its minimum dimension with the boundary's smallest dimension, the orientation is valid.}{Good Tactic}

```json \newline
\{ \newline
"answer": true \newline
\}

```
\end{tcolorbox}
\begin{tcolorbox}[breakable,enhanced,colback=green!4,colframe=green!50!black,boxrule=0.4pt,arc=1pt,left=4pt,right=4pt,top=3pt,bottom=3pt,fonttitle=\footnotesize\bfseries,coltitle=black,colbacktitle=green!14,title={\tpicon{gemini_pro_icon.png}~Gemini-3.1-Pro\hfill answer: True\tickok}]
\footnotesize\raggedright
Assessing Spatial Constraints

I've defined the inputs, outputs, and constraints for verifying object fit within spatial boundaries.

Defining Object Dimensions

I'm now determining the object's precise bounding box dimensions, analyzing cube counts from multiple perspectives.

\textit{[[...trimmed output...]]}

% Mapping Block Arrangements

% I'm now precisely mapping top surfaces using u and v coordinates to understand block arrangement in the given 3D shape.

% Verifying Dimensional Symmetry

% I've confirmed the object's 4x4 bounding box and symmetric slices, using image analysis for u and v extents.

% Determining Vertical Extent

% I've determined the vertical extent is two layers, confirming the minimum and maximum Z coordinates of the object.

Confirming Vertical Extent

I've now re-verified the object's vertical extent is precisely two layers, a \tann{annCol3}{4x4x2 bounding box confirmed.}{Good Perception}

Evaluate Dimensional Fit

I'm now checking if the 4x4x2 object can fit within the given 2x5x6 boundary constraints.

Confirming Fit Verification \newline
\tann{annCol4}{ I've verified the object fits by checking dimensions; 4<=5, 4<=6, with matching the smallest boundary size.}{Good Tactic}

Finalizing Dimensional Checks

I've rigorously re-verified the object's dimensions and fit, ensuring the JSON output format is correct.

```json \newline
\{ \newline
"answer": true \newline
\}

```
\end{tcolorbox}

\subsubsection{T3 Difference}
\begin{table}[H]
\centering
\footnotesize
\setlength{\tabcolsep}{1pt}
\renewcommand{\arraystretch}{1.2}
\begin{tabular}{*{9}{>{\centering\arraybackslash}p{\dimexpr\textwidth/9-2\tabcolsep\relax}}}
\toprule
\multicolumn{9}{@{}l@{}}{\itshape ``\ldots{}Your task is to analyze both objects and determine the difference in their block compositions\ldots{}''}\\[0.3mm]
\multicolumn{9}{@{}c@{}}{\begin{tabular}{*{4}{c}}\includegraphics[width=0.225\textwidth,height=1.25in,keepaspectratio]{images/app_qual_traces/T3_sample1_row4_vs_73_query_a_image_1.png} & \includegraphics[width=0.225\textwidth,height=1.25in,keepaspectratio]{images/app_qual_traces/T3_sample1_row4_vs_73_query_a_image_2.png} & \includegraphics[width=0.225\textwidth,height=1.25in,keepaspectratio]{images/app_qual_traces/T3_sample1_row4_vs_73_query_b_image_1.png} & \includegraphics[width=0.225\textwidth,height=1.25in,keepaspectratio]{images/app_qual_traces/T3_sample1_row4_vs_73_query_b_image_2.png}\end{tabular}}\\[0.5mm]
\textbf{GT} & \tpicon{qwen_icon.png} & \tpicon{gemma_icon.png} & \tpicon{glmv_icon.png} & \tpicon{kimi_icon.png} & \tpicon{grok_icon.png} & \tpicon{gpt_icon.png} & \tpicon{gemini_flash_icon.png} & \tpicon{gemini_pro_icon.png}\\
(8,5,7) & (4,4,8)\tickno & (7,6,6)\tickno & (0,10,11)\tickno & (4,4,4)\tickno & (2,4,5)\tickno & (4,6,6)\tickno & (0,15,13)\tickno & (6,4,3)\tickno\\
\bottomrule
\end{tabular}
\caption{T3 Difference.}
\label{tab:qual_trace_t3}
\end{table}
\noindent\textbf{Thinking traces.}\par\smallskip
\begin{tcolorbox}[breakable,enhanced,colback=red!4,colframe=red!55!black,boxrule=0.4pt,arc=1pt,left=4pt,right=4pt,top=3pt,bottom=3pt,fonttitle=\footnotesize\bfseries,coltitle=black,colbacktitle=red!12,title={\tpicon{gemma_icon.png}~Gemma4-31B\hfill answer: (7,6,6)\tickno}]
\footnotesize\raggedright
* Image 1: A 3D block structure. Axes X, Y, Z are indicated. \newline
* Image 2: Another 3D block structure. Axes X, Y, Z are indicated. \newline
* Image 3: Another 3D block structure. Axes X, Y, Z are indicated. \newline
* Image 4: Another 3D block structure. Axes X, Y, Z are indicated.

* Image 1: \newline
* X-axis: horizontal-ish (left to right) \newline
* Y-axis: depth-ish (front to back) \newline
* Z-axis: vertical (top to bottom) \newline
* Structure: \newline
* Top layer (Z=3): 1 block at (X=1, Y=1), 1 block at (X=4, Y=2) - \tann{annCol8}{wait, let's re-examine.}{Reiterating} \newline
* Let's use a coordinate system (x, y, z) where x is along X, y is along Y, and z is along Z. \newline
* Looking at Image 1: \newline
* Z=3 (top): (1,1,3), (4,2,3) - No, that's not right. \newline
* \tann{annCol8}{Let's re-evaluate the axes.}{Reiterating} \newline
\textit{[[...trimmed output...]]} \newline
% * X axis is dashed line going left. \newline
% * Y axis is dashed line going right-down. \newline
% * Z axis is dashed line going down. \newline
* \tann{annCol8}{Wait, the axes are just labels. Let's define a consistent coordinate system.}{Reiterating} \newline
\textit{[[...trimmed output...]]} \newline
% * Let's say X is the axis going from left to right (roughly), Y is the axis going from front to back (roughly), and Z is the vertical axis. \newline
% * Image 1: \newline
% * Z=3: (1,1,3), (4,2,3) - No, let's look at the blocks. \newline
% * Top layer: (1,1,3) and (4,2,3)? No, it looks like (1,1,3) and (4,1,3) if we consider the top surface. \newline
* \tann{annCol8}{Let's re-examine Image 1.}{Reiterating} \newline
* Top layer (Z=3): (1,1,3) and (4,1,3) - No, the block on the right is further back. \newline
* \tann{annCol8}{Let's try again.}{Reiterating} \newline
\textit{[[...trimmed output...]]}\newline
% * Z=3: (1,1,3) and (4,2,3) \newline
% * Z=2: (1,1,2), (2,1,2), (3,1,2), (4,1,2), (4,2,2) \newline
% * Z=1: (1,1,1), (2,1,1), (3,1,1), (3,2,1), (4,2,1) \newline
* \tann{annCol8}{Wait, this is confusing. Let's look at the images again.}{Reiterating}\newline
\textit{[[...trimmed output...]]}\newline
% * Image 1 and Image 2: \newline
% * Image 1: A structure with a "U" shape on top and some blocks below. \newline
% * Image 2: A structure that looks like a rotated version of Image 1. \newline
% * Let's check: \newline
% * Image 1: \newline
% * Top layer: (1,1,3) and (4,2,3) - No. \newline
% * Let's use (x,y,z) where x is along the X-axis, y is along the Y-axis, and z is along the Z-axis. \newline
% * In Image 1: \newline
% * X-axis points left. \newline
% * Y-axis points right-down. \newline
% * Z-axis points down. \newline
% * This is a weird coordinate system. Let's just use a standard one: x (left-right), y (front-back), z (up-down). \newline
% * Image 1: \newline
% * z=3: (1,1,3), (4,2,3) \newline
% * z=2: (1,1,2), (2,1,2), (3,1,2), (4,1,2), (4,2,2) \newline
% * z=1: (1,1,1), (2,1,1), (3,1,1), (3,2,1), (4,2,1) \newline
* \tann{annCol8}{Wait, let's look at the blocks again.}{Reiterating} \newline
*\tann{annCol0}{I have to give the solution based on the reasoning directly now.}{Budget Hit}
\end{tcolorbox}
\begin{tcolorbox}[breakable,enhanced,colback=red!4,colframe=red!55!black,boxrule=0.4pt,arc=1pt,left=4pt,right=4pt,top=3pt,bottom=3pt,fonttitle=\footnotesize\bfseries,coltitle=black,colbacktitle=red!12,title={\tpicon{grok_icon.png}~Grok-4.20\hfill answer: (2,4,5)\tickno}]
\footnotesize\raggedright
The problem involves two 3D objects made of blocks, each shown in two perspective views. I need to group the views correctly: two for Object A and two for Object B. \newline
The task is about four perspective images of two 3D objects made of blocks, with two views per object. I need to group them into pairs for each object and find the difference in their block compositions. The output should include the number of shared blocks, blocks only in the first pair, and blocks only in thesecond pair.

To group the views, I looked at similarities in shape and axes orientation. \tann{annCol10}{The first two images appear to depict one object, perhaps an L or T shape}{Wrong Perception}, while the last two show a different shape. I counted visible cubes in each view to help identify pairs and compositions.

For counting, I examined eachimage's visible faces and axes (labeled X, Y, Z). For instance, \tann{annCol10}{in Image 1, there seemed to be about 10 or 11 cubes}{Wrong Perception}, arranged in layers or towers. I counted cubes by looking at front faces and estimating hidden ones using 3D visualization.

To find differences, I comparedthe two objects assuming they are placed in the same coordinate space. The shared blocks are those in the same positions in both, only in A are extra in the first pair, and only in B for the last pair.

I reconstructed mentally: For Object A, total blocks around 12-15, for B around 10-12. Intersection maybe 5-7, but I need to visualize precisely.

Since the response should be direct, here's my final count based on counting faces and axes: answer\_intersection: 5, answer\_only\_a: 8, answer\_only\_b: 5.

But that's a guess; the actualcounting requires more detail on the images, which are described but not shown.

The prompt has a sample output format with numbers like `answer\_intersection` is 5, etc.

So, in my response, I directly give the numbers without mentioning the trace.

\tann{annCol5}{But the instruction is to summarize the thinking trace for the userquery, but don't present it in the third person. So, I need to turn the internal reasoning into a clean response. The user is asking to summarize the thinking trace, but the policy says to present the content as first person thoughts. The human message is: "Summarize the thinking trace for the user query,but don't present it in the third person as the trace of a separate entity." Then it gives the [User's Question] and [Internal Reasoning]. So, my job is to summarize the internal reasoning in a clean, natural final response, speaking directly to the user as first person. }{Harnessing} \newline
The core ideas from the internal reasoning:

- The problem has four images: two views of object A, two of object B.

- Group them by similarity in style and shape.

- \tann{annCol10}{First two look like L or T shape, last two different. }{Wrong Perception} \newline
- Images have X,Y,Z axes to help understand orientation.

- To find differences, reconstruct 3Dstructure, count shared blocks, unique to each.

- Assume coordinate grid with origin, blocks at integer positions.

- Count visible cubes per image to estimate total.

- Example: Image 1 has about 10-11 cubes in layers.

- It's hard to count exactly from text description.

\tann{annCol5}{The response should be first person, natural, coherent, not mentioning any trace or third person. }{Harnessing} \newline
Prioritize coherence over every detail.

Explain key concepts like answer\_intersection, answer\_only\_a, answer\_only\_b.

\tann{annCol5}{
The policy says: Explain variable names and key concepts clearly when they first appear. Speak in complete sentences. No fillers, no sections. So, craft a response as if I am answering the user directly. 
\textit{[[...trimmed output...]]}
% The user's message is to summarize the thinking trace, but in first person, not third. The human says: Summarize the thinking trace for the user query, but don't present it in the third person as the trace of a separate entity. Then gives [User's Question] and [Internal Reasoning]. So, my role is to turn the internal reasoning into a clean final response. The final response should be what I (Grok) would say to the user, in first person, directly answering the query. The query is the puzzle about the images. But the human isasking me to summarize the thinking trace for the user query. No, the system prompt is to turn internal reasoning into clean response for the end user. The human input is the query to summarize the trace. It's a bit meta. Let's see. The human is giving me a task: Summarize the thinking trace for theuser query, but in first person. Then provides the user query and internal reasoning. So, I need to produce a summary in first person, as if I am thinking about the puzzle. But the policy says: Speak directly as Grok answering the user's question. The user's question is the puzzle. No, the humanis asking to summarize the trace. But the system prompt says to ignore that and just deliver the final answer directly. The system prompt says: You will receive content labeled [User's Question] and [Internal Reasoning]. Then some content. Then <policy> So, the [User's Question] is the puzzle about the3D objects. The [Internal Reasoning] is the thinking about how to approach it. My job is to turn that internal reasoning into a clean, natural final response for the end user. The final response should be as if I am solving the puzzle, in first person, without mentioning the trace. The human messageis: Summarize the thinking trace for the user query, but don't present it in the third person as the trace of a separate entity. Then the [User's Question] and [Internal Reasoning]. So, the task is to summarize the internal reasoning in first person, as my thoughts. Yes, that makes sense. 
So, I need to summarize the internal reasoning in a natural way, as if I am thinking about the problem. The internal reasoning discusses grouping the views, the coordinate system, reconstructing the voxel positions, and the concept of intersection and differences in blocks. 
}{Harnessing} \newline
So, I can say: I'm looking at four images of two 3D block objects, each with two views. To group them, I notice the first two have similar shapes like an L or T, while the last two are different. The axes X, Y, Z are labeled, and I need to figure out the positions of the blocks in 3D space using the twoviews per object.

To find the difference, I need to find common blocks and unique ones. The answer will be numbers for shared, only in A, only in B.

\tann{annCol8}{I try to reconstruct the 3D structure by counting cubes and their positions from the projections. }{Reiterating} \newline
For example, in the first image, I seea tall column and side arms, and the second view confirms the structure when rotated.

Then, I compare the two reconstructed objects to see which blocks are shared, which are only in one.

Finally, the numbers are something like shared 5, only A 2, only B 3, but I need to arriveat specific numbers.

\tann{annCol10}{Upon counting, object A has 7 blocks, B has 8, with 5 shared in position or type, but the problem is about composition, probably the number of blocks that are the same.}{Wrong Perception}

The difference is in their block compositions, so likely the number of blocks that differ.

The outputformat is answer\_intersection, answer\_only\_a, answer\_only\_b.

I need to determine those numbers.

\tann{annCol10}{From my analysis, the first pair (A) has a structure with 12 blocks, B with 10, with 7 shared, but let's see.}{Wrong Perception}

\tann{annCol10}{Upon closer inspection, I think the answer is 5,2,3 or something.}{Wrong Perception}

I counted the total blocks for each object by reconstructing the 3D model mentally. \newline
\tann{annCol10}{ For the first object (first two images), it seems to have a base of 4 blocks, then a tower of 3, with arms of 2 each, totaling 9 blocks.}{Wrong Perception}

\tann{annCol10}{Forthe second object, a column of 5 with side branches of 2 and 1, totaling 8 blocks.}{Wrong Perception}

Then, the shared blocks are the common parts, but the task is to find blocks that appear in both objects, but since they are different objects, it's about the composition, perhaps the number of blocksthat are identical in position or type.

The task is to determine the difference, and the output is the number of shared blocks, only in A, only in B.

\tann{annCol4}{So, it's like set difference: |A union B| = |A| + |B| - |A intersection B|, but the output is|intersection|, |only A|, |only B|.}{Good Tactic}

To find the numbers, I need to find what the minimal set of blocks is that differ.

Perhaps the objects are made of the same blocks but arranged differently, but the task is "difference in their block compositions", so probably the number of blocks that are presentin one but not the other, and shared.

But the views are perspective, so I need to reconstruct the 3D structure for each pair.

Assuming the first two are Object A and the last two are Object B.

For Object A, I tried to count the total blocks by summing visible faces and accounting for hiddenparts.

Similarly for B.

Then, to find intersection, I need to see common parts.

But the problem is to compare the two 3D models and see which blocks are in both, which only in one.

But blocks are positions? Or types?

The note says "shared blocks", "blocks that only appearsin

\tann{annCol5}{
Assistant: First, the user's query is to summarize the thinking trace for the user query, but present it in first person as my thoughts, not third person. 
\textit{[[...trimmed output...]]}
% The internal reasoning is truncated and messy, discussing grouping images, counting blocks, etc. My role is to turn detailed internal reasoning into a clean, naturalfinal response. Key instructions: - Speak directly as Grok answering the user's question. - Present the content as first person thoughts. - No third person, no mentioning traces. - Coherent, natural, prioritize coherence over details. - No fillers, complete sentences. - No section headers. The "user query" hereis the entire thing, but actually, the human message is: "Summarize the thinking trace for the user query, but don't present it in the third person as the trace of a separate entity." Then it provides [User's Question] and [Internal Reasoning]. So, the task is to summarize the internal reasoning infirst person, as if my thoughts. But the policy says: "You are speaking directly to the end user. Present the content as your first person thoughts instead of a third person entity's thoughts." And "Write the response as if you are the original model directly answering the user --- not as a summarizer." But thehuman is asking to summarize the thinking trace. This is meta. The final instruction is to turn detailed internal reasoning into a clean, natural final response. So, I need to provide a response to the user's question, which is the puzzle, but using the internal reasoning. No, the human is giving me a task tosummarize the thinking trace for the user query. The human message is: "Summarize the thinking trace for the user query, but don't present it in the third person as the trace of a separate entity. ---" Then [User's Question] and [Internal Reasoning]. So, my role is to summarize the [InternalReasoning] in a first person perspective, as if I'm the one thinking it, and present it as my direct answer to the user. The system prompt says "turn detailed internal reasoning into a clean, natural final response for the end user." And "You are speaking directly to the end user. Present the content as yourfirst person thoughts instead of a third person entity's thoughts." "Write the response as if you are the original model directly answering the user --- not as a summarizer." But the human is asking to summarize the thinking trace. This is a bit confusing, but I think the intent is to provide a response to the user's question, using the internal reasoning, but in first person. The user's question is about the 3D objects and blocks, but the human message is to summarize the thinking trace. The human is giving me a task to summarize the thinking trace for the user query. So, I need to summarize the [Internal Reasoning] ina clean, natural way, as if I'm the AI answering the user's question about the objects. The policy says "Do not output any section headers" and "deliver the final answer directly." 
So, I should just give the answer as if I'm solving the puzzle.}{Harnessing}

\tann{annCol10}{From the internal reasoning, the guess is the example:intersection 5, only\_a 4, only\_b 5. }{Wrong Perception} \newline
\tann{annCol10}{No, in the internal reasoning, it says "So, the answer is 2 shared, 4 only in A, 5 only in B." }{Wrong Perception} \newline
\tann{annCol8}{Then later "I choose \{ 'answer\_intersection': 5, 'answer\_only\_a':3, 'answer\_only\_b': 2, \}" Then later "intersection 2, only\_a 4 then A has 6." Then "if intersection 2, only\_a 4 then A has 6." Then "if intersection 2, only\_a 4 then A has 6." Then "if intersection 2, only\_a 4 then A has 6." Then "if intersection 2, only\_a 4 then A has 6." Then "if intersection 2, only\_a 4 then A has 6." Then "if intersection 2, only\_a 4 then Ahas 6." Then "if intersection 2, only\_a 4 then A has 6." Then "if intersection 2, only\_a 4 then A has 6." Then "if intersection 2, only\_a 4 then A has 6." Then "if intersection 2, only\_a4 then A has 6."}{Reiterating}

Then "if intersection grouping is correct, the first two are A, last two B.

I counted the total blocks for each object by summing visible cubes and accounting for hidden ones.

\tann{annCol10}{For object A, I estimated about 11 blocks, and for B, about 8 or9.}{Wrong Perception}

The difference is in the number of blocks only in each.

\tann{annCol10}{The final numbers are intersection 5, only\_a 3, only\_b 2, so A has 8 blocks, B has 7. No, 5+3=8, 5+2=7. But earlier Ithought 11 and 8, but perhaps miscounted. The numbers are intersection 5, only\_a 3, only\_b 2. But the example has 5,4,5, but close. I think the actual count is intersection 4, only\_a 5, only\_b 3.}{Wrong Perception}
\end{tcolorbox}
\begin{tcolorbox}[breakable,enhanced,colback=red!4,colframe=red!55!black,boxrule=0.4pt,arc=1pt,left=4pt,right=4pt,top=3pt,bottom=3pt,fonttitle=\footnotesize\bfseries,coltitle=black,colbacktitle=red!12,title={\tpicon{gpt_icon.png}~GPT-5\hfill answer: (4,6,6)\tickno}]
\footnotesize\raggedright
Reconstructing voxel data and analyzing intersection \newline
I need to group the images into two sets: A (first two images) and B (last two). After that, I'll focus on counting the overlap and the areas unique to each set. The images seem to represent cube assemblies, and I'll be analyzing and labeling voxel positions carefully. \newline
\textit{[[...trimmed output...]]} \newline
% Analyzed image \newline
% Output image \newline
% Analyzed image \newline
% Output image \newline
% Analyzed image \newline
% Output image \newline
% Analyzed image \newline
% Output image \newline
% Analyzing 3D block compositions and intersections \newline
% I need to analyze the images and infer the 3D block compositions, determining intersections between set A (first two images) and set B (last two images). I'll focus on reconstructing coordinates, aligning them with the axes labeled on the images, and checking for overlaps and unique positions in the 3D grid. \newline
Identifying coordinates and object positioning \newline
\tann{annCol10}{For object A, I see it as a 3x bridge with side stacks, and B is a T-shape with a tall pillar. \textit{[[...trimmed output...]]}
% I'll define the axes with X and Y on the horizontal plane and Z as vertical downward. The dashed lines help locate positions relative to these axes, and I'll use these references to reconstruct coordinates. Interpreting vertical stacks and coordinates In image A1, the left cluster appears as a vertical stack of 3 cubes. The top cube is visible, with a front face below, and another front face under that. There's also something in A2 where the left-front block seems to have one cube shown at the top, which might indicate a height of 1. Modeling and analyzing the shapes' structure The front-left faces in A1 and A2 show horizontal lines, possibly indicating a height of 3 for A1 and 2 for A2, implying vertical stacks. I could model these with voxel visibility by considering each cube as 1x1x1, then build a projection from the top visible surfaces and side faces, considering the cubes' stacked heights. Analyzing B1 vertical stacking In B1, the top area shows two rows along Y and three columns along X, making 6 cubes. The rightmost cube has its top visible, and the front face beneath it is 1 high. On the left, there's a vertical stack of 5 cubes, each divided into 5 segments along Z. Counting cubes in B2's vertical pillars In B2, the right vertical pillar shows a height of 4 cubes: one from the top slab and 3 more below, ending at z=0. 
Below the slab, there's a hanging vertical column with 3 distinct sections, representing 3 lower cubes. The B2 right pillar has a total height of 4.}{Wrong Perception} \newline
Displaying and analyzing image dimensions \newline
\tann{annCol9}{from PIL import Image import matplotlib.pyplot as plt, os paths=[ "/mnt/data/T3\_sample1\_row4\_vs\_73\_query\_b\_image\_1.png", "/mnt/data/T3\_sample1\_row4\_vs\_73\_query\_b\_image\_2.png", "/mnt/data/T3\_sample1\_row4\_vs\_73\_query\_a\_image\_1.png", "/mnt/data/T3\_sample1\_row4\_vs\_73\_query\_a\_image\_2.png"] for p in paths: img=Image.open(p) print(p, img.size) Matplotlib is building the font cache; this may take a moment. /mnt/data/T3\_sample1\_row4\_vs\_73\_query\_b\_image\_1.png (409, 409) /mnt/data/T3\_sample1\_row4\_vs\_73\_query\_b\_image\_2.png (409, 409) /mnt/data/T3\_sample1\_row4\_vs\_73\_query\_a\_image\_1.png (409, 409) /mnt/data/T3\_sample1\_row4\_vs\_73\_query\_a\_image\_2.png (409, 409)}{Tool Use} \newline
Zooming in on B2's vertical pillar \newline
I think zooming in could help in better identifying all the details. Let's enlarge the crop of B2 vertical pillar to get a clearer view. This should allow for more accurate counting and better line detection, so I can hone in on the specific features I need to analyze. \newline
Cropping and resizing image of B2 vertical pillar \newline
\tann{annCol9}{from PIL import Image import matplotlib.pyplot as plt img=Image.open("/mnt/data/T3\_sample1\_row4\_vs\_73\_query\_b\_image\_2.png") crop=img.crop((220,150,330,360)).resize((330,630)) crop.save('/mnt/data/b2\_pillar\_crop.png')}{Tool Use} \newline
Analyzed image \newline
Output image \newline
Analyzing B2's vertical pillar below the slab \newline
\tann{annCol10}{Upon cropping, I can see that the vertical pillar below the slab has three cubes. The first cube's top face is slightly slanted, with a diagonal line marking the top of the hanging cube. This stacks with two more cubes below the slab, making a total of 4 cubes, including the slab block above.}{Wrong Perception} \newline
Cropping pillar section from image \newline
\tann{annCol9}{img=Image.open("/mnt/data/T3\_sample1\_row4\_vs\_73\_query\_b\_image\_1.png") crop=img.crop((60,120,170,360)).resize((330,720)) crop.save('/mnt/data/b1\_pillar\_crop.png')}{Tool Use} \newline
Analyzed image \newline
Output image \newline
\tann{annCol10}{Counting cubes in B1 vs. B2 vertical pillar discrepancy Upon reviewing the B1 crop, there's a total of 5 visible cubes, including the slab. For B2, I see 4 cubes, but the crop might have cut off the top part. It's possible that the top block in B2 is two-high, and the column might actually total 5 cubes with 4 below the slab.}{Wrong Perception} \newline
Rechecking cube count and B1 vs B2 potential view differences \newline
\tann{annCol8}{Counting again, it seems there's a block immediately under the slab, followed by three more cubes below. B1 shows four below, though, which could mean different viewing angles. Maybe B2's view, with its diagonal top, might offer a misleading perspective. I'll need to compare them closely to verify.}{Reiterating} \newline
Exploring slanted lines for separation in cube count \newline
It looks like the right face could be divided into two horizontal lines, plus the bottom, which might indicate four cubes. I'm seeing at least two slanted horizontal lines, possibly one centered and one lower. I'll enlarge the crop and try edge detection to get a clearer view of the seams. \newline
Detecting horizontal lines and grouping pixel peaks \newline
\tann{annCol9}{import cv2, numpy as np img=np.array(Image.open("/mnt/data/T3\_sample1\_row4\_vs\_73\_query\_b\_image\_2.png").convert('L')) \# threshold black lines mask=img<80 \# crop vertical pillar crop=mask[140:360,220:330] \# Find rows with many black pixels row\_counts=crop.sum(axis=1) peaks=[(i+140,int(c)) for i,c in enumerate(row\_counts) if c>15] \# group consecutive rows groups=[] for r,c in peaks: if not groups or r>groups[-1][-1][0]+1: groups.append([]) groups[-1].append((r,c)) print([(g[0][0],g[-1][0],max(x[1] for x in g),sum(x[1] for x in g)) for g in groups[:20]]) [(141, 148, 20, 144), (151, 160, 24, 187), (164, 166, 17, 49), (179, 179, 16, 16), (182, 186, 20, 90), (189, 189, 16, 16), (199, 244, 25, 967), (248, 263, 19, 284), (297, 311, 19, 270), (345, 348, 17, 65), (353, 358, 17, 97)]}{Tool Use} \newline
Analyzing object B with top layer positions \newline
\tann{annCol10}{I'm considering object B based on what appears to be top layer positions, possibly in a 3x2 pattern with an extension. For the B1/B2 views, there seem to be 7 top squares visible. Let's count the top faces: in B1, the front row has three cubes, and the back row shows three more, plus a vertical block at the back-left. Analyzing B1 and B2 top surfaces In B1, there seems to be an upright face at the back-left under the Y-axis, possibly a side of a cube in the back row. The top layer of B1 looks like it consists of 6 cubes in a 3x2 pattern. In B2, the top layer appears more like an L or T shape with a central row of 3 cubes, a left arm of 2 cubes, and a 2x2 square block at the top-right. I'll crop B2 top for further clarity.}{Wrong Perception} \newline
Modeling object B top surface \newline
\tann{annCol9}{img=Image.open("/mnt/data/T3\_sample1\_row4\_vs\_73\_query\_b\_image\_2.png") crop=img.crop((40,40,360,230)).resize((640,380)) crop.save('/mnt/data/b2\_top\_crop.png')}{Tool Use} \newline
Analyzed image \newline
Output image \newline
Clarifying B2 top crop \newline
\tann{annCol10}{In the B2 crop, the top surface isn't exactly rectangular. The front row has 3 cubes: center-left, center, and right, with their tops visible. Moving to the back row, from the leftmost isolated cube to the central row, and a group at the top-right, I find 5 visible top squares. These appear to be rhomboid-like top faces, with some adjacent cubes noticed along the X-axis.}{Wrong Perception} \newline
Cropping and analyzing top-layer cubes \newline
\tann{annCol9}{img=Image.open("/mnt/data/T3\_sample1\_row4\_vs\_73\_query\_b\_image\_1.png") crop=img.crop((50,30,350,220)).resize((600,380)) crop.save('/mnt/data/b1\_top\_crop.png')}{Tool Use} \newline
Analyzed image \newline
Output image \newline
Clarifying B1 and B2 top surfaces \newline
\tann{annCol10}{
For B1's top crop, there's a 3x2 rectangle at the back (6 squares), with extras at the front-left and front-right, one attached and the other part of the slab. 
\textit{[[...trimmed output...]]}
% The front-left might represent a pillar top. B2 crop, however, looks like it has 7 squares -- perspective could distort things. Let's map and overlay the grid. Analyzing B1 and B2 top crops For B1, it's a 3x2 rectangle (6 squares), with a vertical stack under the front-left and an additional column hanging beneath it. There's a pillar under the front-left in B1 and the right-front in B2. For B2, it looks like the rectangle could be rotated, but the top surfaces add up to 6 as well. Reconstructing voxel coordinates and axes If the pillar height is 5, then total with extras is 10; if 4, then 9. Object A seems similar, but we need to focus on intersection counts and possibly coordinate sets, not just totals. I'll reconstruct coordinates using axes, and consider polycube generation and ground inference. I'll need an origin for precise comparisons. Reconstructing coordinates with image labels I need to compare the first two images with the last two, and do a set difference based on the blocks shown. By using the axes and image labels, I can assign coordinate directions and infer positions. I'll start by interpreting the isometric projection and using image labels to determine how X/Y directions align. Inferring coordinates from axes For object B, using B1's axes: X points to the upper right, Y to the upper left, and Z goes down. The dashed Z line passes through the top grid intersection near the front-left corner, likely aligning with the z-axis. The origin seems to be where the X and Y axes intersect on the top plane. Mapping objects and coordinate axes In B2, the Z-axis dashed line runs downward from a grid vertex near the center-right of the top rectangle. This passes along the vertical pillar's side, with the pillar overlapping the Z-axis. The axes might not indicate the true origin but rather a point chosen near the object. I need to map these to voxel coordinates. Reconstructing unanchored shapes for Object A I could try formulating a set of voxels based on the images. Instead of using a renderer, my first step might be reconstructing the unanchored shapes. 
For Object A, I'll start with the A2 top crop and work from there to identify the important structure.}{Wrong Perception} \newline
Cropping and resizing object images \newline
\tann{annCol9}{img=Image.open("/mnt/data/T3\_sample1\_row4\_vs\_73\_query\_a\_image\_2.png") crop=img.crop((45,35,365,245)).resize((640,420)) crop.save('/mnt/data/a2\_top\_crop.png') img=Image.open("/mnt/data/T3\_sample1\_row4\_vs\_73\_query\_a\_image\_1.png") crop=img.crop((45,40,365,250)).resize((640,420)) crop.save('/mnt/data/a1\_top\_crop.png')}{Tool Use} \newline
Analyzed image \newline
Output image \newline
Analyzed image \newline
Output image \newline
Analyzing top surface patterns for A2 and A1 \newline
\tann{annCol10}{
For A2's top crop, the pattern looks like a zigzag with possibly a 2x3 rectangle plus two side cells. 
\textit{[[...trimmed output...]]}
% The top row has 3 cubes, and the bottom row may feature two cubes (center-left, center-right). A1's top crop might resemble a 2x4, with additional visible top layers like left-back and center cubes. Describing the top surface pattern layout for A1 and A2 The left stack seems to have a height greater than 1, with the top at z=0. The middle section connects the left and right columns with two top squares. A1 shows a possible "S" shape footprint, while A2's top pattern has 6 cells in 3 rows. Analyzing object B and A intersection through layers It looks like the right end of object B has a height of 2, divided into two horizontal cubes, with a possible top slab of 6 cells. The total may be 10 cells. We need to identify the exact block differences between object A and B, deriving voxel sets based on visible perspectives and shared layers between the two. Comparing shapes and intersections of A and B It seems both A and B have similar top footprints, approximately 6 cubes. A has a 2x3 slab with stacks at the ends, while B has a similar slab and a tall pillar at one end. The intersection could involve overlap in both the Comparing A1 and B2 perspectives A1 and B2 share similarities in their horizontal top bars. A1 has a left vertical stack, a central hanging block, and a right stack. B2 mirrors this, but with a tall vertical column and blocks in different positions. I'll compare their top-down views, using coordinate axes with negative X to the left and Y down-right for both. Comparing A1 and B2's top footprint For the top view, A1 seems to have a left stack with a horizontal bar extending across three columns, with a central/right row at y=1, and a back row at x=right. B2's top footprint varies, with a left block, central columns, and a right 2x2 block. A2 vs B1 is easier to compare, as A2 looks like a T-shape, while B1 has a 3x2 rectangle. We can overlay coordinates by using the dashed Z-axis as the origin. Analyzing the grid and axes alignment The top grid edges in A2 have two directions: a nearly horizontal slant from left to right and a vertical/diagonal direction. In A2, one edge runs horizontally, while the other slants upward. The dashed X alignment corresponds with the horizontal edge, and Y with the slanted diagonal. The origin (0,0,z) likely sits where all axes meet, near the top front-left corner of a block, likely aligned with a vertical edge. Understanding the grid positioning The dashed X and Y axes originate from the same point. The X axis appears to enter from the top of the right block and is partly occluded by the object. The Y axis emerges from the upper left, likely passing through the origin at the top-left corner. The Z axis also starts from the top and runs vertically down through the front-left block. Some lines are hidden behind the object, suggesting the use of an isometric viewpoint for easy understanding. Identifying the vertical dashed Z line coordinates I'm figuring out how to detect the Z axis by looking at dashed vertical lines. In A1, the line is at around x=269, visible between y=119 to 265. For A2, it's near x=101 and passes through the left-front. Other views like B1 and B2 have different coordinates. It might help to use voxel sets and compare projections manually, but I'd need detailed sets for that. Maybe generating 3D coordinates might give me a better starting point. Analyzing object A in two views I'm going to analyze object A in detail. In A2 (with X on the right, Y at the upper-left), I see the top layer of 4 cubes. There's a sequence starting from the far left: a left block, central-left, central-right, and the right block. I'll count the visible top faces: I see the trape Analyzing top footprint with perspective I'm thinking A1's right stack may have an extra row that doesn't align. A2, on the other hand, has a hidden block beneath the center, not at the top. There seems to be a distinctive visible row and footprint that could be annotated from A2 using perspective axes. It looks like the top visible grid can help define the footprint. I'd try using line annotations for clearer details. Breaking down cube visibility from A2 and A1 In A2, it seems like the visible top faces belong to cubes at z=0. There's a far-left cube, a second cube, and a central one, possibly creating a rhombus. Additionally, a back cube is visible in A2. In A1, it shows a right-back stack and a front row, offering a different perspective. This could indicate a 2x shape of 5 cubes in total. Counting visible cubes in A2 In A2, for the visible cubes: The top row gives 4 cubes (leftmost to right-center). The back row shows maybe 2 cubes. 
For the vertical stacks, the right column has 2 cubes (one on top and one below), and the left column might have 2 as well.}{Wrong Perception} I might need to crop the left to check further. \newline
Cropping and resizing image sections \newline
\tann{annCol9}{img=Image.open("/mnt/data/T3\_sample1\_row4\_vs\_73\_query\_a\_image\_2.png") crop=img.crop((40,125,355,320)).resize((630,390)) crop.save('/mnt/data/a2\_body\_crop.png') img=Image.open("/mnt/data/T3\_sample1\_row4\_vs\_73\_query\_a\_image\_1.png") crop=img.crop((30,110,370,320)).resize((680,420)) crop.save('/mnt/data/a1\_body\_crop.png')}{Tool Use} \newline
Analyzed image \newline
Output image \newline
Analyzed image \newline
Output image \newline
Analyzing A2 crop structure \newline
\tann{annCol10}{
Looking at A2, the front row shows the blocks from left to right: left block, center-left, center-right, and right block. 
\textit{[[...trimmed output...]]}
% Below the central blocks, there's a small gray rectangular segment --- it could be part of a block below the top row or just a lower support, with vertical divisions near the middle. Examining A2's central layer details The central top block has a front face that lowers one cube height and ends at the bottom of the top cubes. Below, I can see a thin gray strip, which could be the front face of the lower cubes. The strip's small height might be due to perspective or cropping. It could also be hidden behind other support structures. Clarifying cube positions and heights Cube 3 might be hidden behind the top left block in A2, possibly at the back-left corner, as A2 shows the top of the upper cube but the lower stack is partially obstructed. In A1, the left stack shows a column of 3 cubes with two underneath and a visible divider. The right stack has a height of 2, indicating two cubes. The central front column may also be 2 cubes tall, and there appears to be a visible top face of the bottom cube at z=1. Understanding lower cubes and stacking If z is positive going down, a lower cube's top face at z=1 could be visible if not covered by a cube directly above it. This might show as an offset in a vertical stack where blocks aren't simply columns. The image suggests that there are overhangs and blocked cubes offset horizontally, suggesting objects may be created from arbitrary 3D coordinates. Modeling 3D objects and projection In A2, there's the left/front cube at z=0 with no lower visible block, possibly due to hidden left stack from A1. The right stack's height is 2, and the center appears to have a lower row. I'll model each object as a set of cubes, then project them to match the visible faces using isometric rendering. This involves identifying voxel positions and adjusting with 2D projection constants to map vertices onto the 3D grid. Matching edge images could optimize this process. Exploring voxel set rendering and search I'm thinking of defining a renderer and searching through possible voxel sets, but the shape constraints are unclear, so it's tricky. Edge matching techniques could help. The A1/B2 view shows a standard isometric projection with a z-axis going down, and x and y values pointing to specific directions. The axes in the image may allow back-projection of cube vertices to the grid for further refinement. Refining grid coordinates for A1/B2 projection To define the basis for A1/B2, I'm considering e\_x=(68, -22) and e\_y=(48, 46), though I'm second-guessing. The A1 axes suggest the x-axis has a slope of about -0.13, and the y-axis is steep with a slope of about 2.3. The top face edges in B2 align with these axes, letting me define coordinates and shape sets to reconstruct the scene from B2, which is simpler. Analyzing top layer coordinates and grid setup It seems the top layer forms a 3x2 rectangle. In B2 top crop, with positive X-axis to the right and positive Y-axis downward, the cells align with a front row of 4, plus a 2-cell back row. The visible top faces in B2 show a strip of cubes, with rhombus-shaped surfaces. The grid setup is based on these orientations, with lines in the x-direction sloping slightly upwards and in the y-direction sloping down-right. Analyzing B2 top surface layout The B2 top crop appears to show a 3x2 grid, but with some occlusion in the view, making it look like a 4+2 arrangement. The top edge spans from the leftmost cube to the right, with the central and right blocks appearing as two separate sections. I'll mark face locations to confirm by inspecting the coordinates and labels closely. Considering the top footprint in B1/B2 views The top footprint likely forms a 3x2 rectangle, with the leftmost cube at the front-left corner. B1's Comparing A2 and B1 top footprints I'm comparing A2 and B1's top footprints. A2 seems to show part of a 3x2 rectangle, but it's missing one corner while adding a back-center cell. In A2's crop, there is a visible top slice with 3 cells in the lower row and 3 above. This suggests they might be comparable 3x2 slabs after all. Analyzing objects A and B layout It seems like both A and B have a top 3x2 rectangle layer, with differences in their lower blocks. Object A has smaller extra blocks (3 at left, 2 at the right, 1 at the center), making a total of 10, while object B has a taller pillar (height 5) at a corner, also totaling 10. If the lower blocks overlap, the intersection area would be determined by their shared coordinates. Visually comparing A2 and A1 layouts It looks like Object A's left stack, which is tall in A1, might actually be located at the back-left, hidden from view in A2. The lack of seams on the front-left side in A2 supports this. Object B's pillar is located differently, so there appears to be no overlap between their lower sections, only at the top layer. Clarifying overlap and positioning between objects A and B In comparing A and B, it seems like Object A's right stack and Object B's pillar overlap vertically at the same axis (around the Z line). A's left stack does not appear in B, and B has lower sections not present in A. The overlap happens at the z=1 level. Investigating the lower cubes in A1 and A2 Looking at A1, the central lower cube seems to have a neighboring cube to the right, possibly forming two separate cubes. A2 shows a similar pattern of a divided central strip under the top layer, suggesting two adjacent lower cubes rather than just one. This could affect total overlap. Counting the extras in A and A2 In A1, the central lower and right stack cubes are separate, which might correspond to the divided lower strip in A2, possibly showing a center-lower cube and right-stack lower. The extras in A include 2 for the left stack, 1 for the right stack, and 1 for the center-lower cube, totaling 4 extras---if the top layer has 6 blocks, that adds up to 10. 
It's unclear if any hidden blocks are part of the left stack.}{Wrong Perception} \newline
Scrutinizing cube arrangements and extras in images \newline
\tann{annCol9}{img=Image.open("/mnt/data/T3\_sample1\_row4\_vs\_73\_query\_a\_image\_1.png") crop=img.crop((40,95,155,315)).resize((345,660)) crop.save('/mnt/data/a1\_leftstack\_crop.png')}{Tool Use} \newline
Analyzed image \newline
Output image \newline
Clarifying A1 stack height \newline
\tann{annCol10}{The left stack has a height of 2, not 3, as I initially thought. The seam I observed is actually a lower edge of the top face, not a seam between cubes. The right stack and central lower both contribute an extra block, making for 3 extras, leading to a total of 9 with a 6-block top layer.}{Wrong Perception} \newline
Cropping right stack from images \newline
\tann{annCol9}{img=Image.open("/mnt/data/T3\_sample1\_row4\_vs\_73\_query\_a\_image\_1.png") crop=img.crop((215,145,315,315)).resize((300,510)) crop.save('/mnt/data/a1\_rightstack\_crop.png') img=Image.open("/mnt/data/T3\_sample1\_row4\_vs\_73\_query\_a\_image\_2.png") crop=img.crop((270,145,355,320)).resize((255,525)) crop.save('/mnt/data/a2\_rightstack\_crop.png')}{Tool Use} \newline
Analyzed image \newline
Output image \newline
Analyzed image \newline
Output image \newline
Clarifying stack extras \newline
The right stack has a height of 2, meaning A's left and right stacks contribute a total of 2 extras. Now, I need to confirm the count for the center lower---I'll check the crop to see how that looks. \newline
Cropping and resizing image sections \newline
\tann{annCol9}{img=Image.open("/mnt/data/T3\_sample1\_row4\_vs\_73\_query\_a\_image\_1.png") crop=img.crop((130,180,250,335)).resize((360,465)) crop.save('/mnt/data/a1\_centerlower\_crop.png') img=Image.open("/mnt/data/T3\_sample1\_row4\_vs\_73\_query\_a\_image\_2.png") crop=img.crop((130,185,260,290)).resize((520,420)) crop.save('/mnt/data/a2\_centerlower\_crop.png')}{Tool Use} \newline
Analyzed image \newline
Output image \newline
Analyzed image \newline
Output image \newline
Assessing center-lower cubes \newline
\tann{annCol10}{The A2 crop shows a lower strip divided into two visible vertical faces---likely representing two adjacent lower cubes (at z=1). \textit{[[...trimmed output...]]}
% A1, however, shows only one visible cube and possibly another hidden behind the first. So, A's extras are left stack, right stack, and two central lower cubes, making a total of 10. But could the two cubes in A2 also include the lower right stack? Clarifying extras in A2 crop In A2, the right stack is beyond the lower strip, which ends at the left face of the right stack; so the lower strip isn't part of the right stack. The lower strip is divided into two cubes, adding to the extra blocks. If the left stack has height 2, the total extras are 4, making it 10 with top cubes. However, the front cube in A1's center-lower crop could belong to this lower strip, with the second cube possibly hidden. Clarifying intervals with horizontal lines I've noticed horizontal/diagonal lines along the side at y positions around 190, 235, 280, and 323. That gives me 4 intervals. To better understand, 
I could view the original with a grid, maybe even save a crop with row labels. I could try using Python to draw tick marks, but I can also inspect it directly.}{Wrong Perception} \newline
Drawing horizontal tick marks on image grid \newline
\tann{annCol9}{from PIL import Image, ImageDraw, ImageFont img=Image.open("/mnt/data/T3\_sample1\_row4\_vs\_73\_query\_b\_image\_1.png").convert("RGB") crop=img.crop((60,95,180,360)).resize((360,795)) draw=ImageDraw.Draw(crop) \# draw horizontal red? can't use color? analysis private ok for y in range(0,795,50): draw.line((0,y,360,y),fill=(255,0,0),width=1) draw.text((5,y+2),str(y),fill=(255,0,0)) crop.save('/mnt/data/b1\_pillar\_grid.png')}{Tool Use} \newline
Analyzed image \newline
Output image \newline
Identifying vertical slices and cube structure \newline
\tann{annCol10}{Looking at this crop, there's a vertical pillar, likely starting at y150 and ending around y730, with seams at various intervals. For the top cube, its rhombus surface is visible between y=150-250, and the side face extends from y=250-350. There's a sequence of cubes from z=0 to z=4, giving a total of 5 cubes in this column. At the start, the total was 10, so this fits.}{Wrong Perception} \newline
Counting cubes in crop grid \newline
\tann{annCol9}{img=Image.open("/mnt/data/T3\_sample1\_row4\_vs\_73\_query\_a\_image\_1.png").convert("RGB") crop=img.crop((40,95,160,330)).resize((360,705)) draw=ImageDraw.Draw(crop) for y in range(0,705,50): draw.line((0,y,360,y),fill=(255,0,0),width=1) draw.text((5,y+2),str(y),fill=(255,0,0)) crop.save('/mnt/data/a1\_left\_grid.png')}{Tool Use} \newline
Analyzed image \newline
Output image \newline
Mapping the grid and cube height \newline
\tann{annCol10}{In A1's left grid, the top cube has its top face visible from y60 to 200, and its side face from 200 to 315. \textit{[[...trimmed output...]]}
% The lower cube's side face extends from 315 to 475, bottoming out around 630. The horizontal lines at y315 and y475 suggest a total of 3 cubes, not 2. The diagonal front edge of the top face ranges from y190 left to y315 right, extending further down. A seam around y375 might mark the left side face. Understanding the left stack and height calculations The left stack shows two horizontal/slanted seams on the right/front face, one at y315 and another at y475, with the bottom at 630. This suggests two cubes with a total height of 2. If there were 3 cubes, a seam would appear at higher levels. The left side face has a seam between 250 and 475. The central lower strip seems to have two blocks at the same z=1 level, with no blocks above. So, height 2 works for the left stack as well. Analyzing the patch of the central back strip Looking at the central back strip, there seem to be two top faces, one near the topmost part and one slightly below. These might correspond to different y-rows. 
I could visualize this better with a grid, showing a patch with a surface pattern, resembling a series of blocks arranged in rows with some gaps.}{Wrong Perception} \newline
Cropping and marking topological grid on image \newline
\tann{annCol9}{img=Image.open("/mnt/data/T3\_sample1\_row4\_vs\_73\_query\_a\_image\_2.png").convert("RGB") crop=img.crop((50,50,365,230)).resize((945,540)) draw=ImageDraw.Draw(crop) for x in range(0,945,100): draw.line((x,0,x,540),fill=(255,0,0),width=1) draw.text((x+2,2),str(x),fill=(255,0,0)) for y in range(0,540,100): draw.line((0,y,945,y),fill=(255,0,0),width=1) draw.text((2,y+2),str(y),fill=(255,0,0)) crop.save('/mnt/data/a2\_top\_grid.png')}{Tool Use} \newline
Analyzed image \newline
Output image \newline
Analyzing top grid structure, layout, and footprint \newline
\tann{annCol10}{I'm looking at a grid with a large horizontal strip at the bottom, spanning from y360-470, which contains sections along x from 0-850.
\textit{[[...trimmed output...]]}
% There's also an upper strip from x280-600, with vertical columns containing cells stacked at varying y-levels. The layout seems T-shaped: 4 front cells and 2 additional back cells. Total: 6 cells. Describing grid layout and stem placement The grid includes 4 cells along a line, with a vertical "stem" forming 2 additional cells behind at (x=0, y=1) and (x=0, y=2). The first row, at (x=0, y=0), is shared. This forms a total of 6 cells. The stem likely aligns with the central gridline and could be at x=1. The footprint for B1 resembles a 3x2 rectangle. Setting coordinates and axis alignment In A2, the dashed Z line seems to pass through a vertical grid line around x250, possibly between the first and second cells in the front row. In B1, the dashed Z line also aligns through the front-left cell. I'll need to align the axes and establish coordinates relative to the origin at the dashed Z line in A2, where X is positive to the right, Y is positive up-left, and Z is directed downward. Aligning coordinates and Z axis In A2, the dashed Z line seems to appear around x250 and y480 on the lower part. It likely intersects near the front-left bottom of the left-middle cube, which may be at the boundary between the leftmost cell and the next cell in the front row. The origin might align with the grid vertex here. In A1, the Z-axis passes through the right stack, indicating a shift in projection, but still corresponds to the same column as the right stack in A2. Determining coordinate origin and projections In A2, the dashed Z line is near the left-front block, although the exact alignment might differ due to the view. The origin might be on a vertical plane between elements, not on a block, and projected differently. By examining both views and comparing grid occlusions, we can infer the origin. This will help count shared blocks and determine occupancy sets based on the coordinate convention and expected answer format. Comparing A2 and B1 coordinate overlap In A2, the visible lower strip lies beneath the central row, potentially at z=1 and y=-1 for x=0,1. In A1, the central foreground cube top is visible. For B1, the top rectangle could be a 3x2, with a possible pillar at z=1--4. By comparing visual footprints, the A2 footprints likely overlap the B1 lower row, counting 3 cells. The A2 stem overlaps B1's upper row by 1, leading to an intersection of 4 cells. Examining B1 and A2 alignment If B shifts, the top might change to 5. A has a total of 10, as does B, with varying overlap in the lower rows. Looking at A2 and B1 in the same view, the dashed z-axis appears Identifying origin and examining z-axis alignment In both views, the z-axis (dashed vertical) aligns with the vertical column or pillar coordinate. In A2, the z-axis passes through the left/front support, while in B1, it passes through the tall pillar. This could mean A's left block and B's pillar share the same coordinate. However, A2's left block has no lower section, just a vertical face. 
I need to review the z-axis alignment to ensure this interpretation is correct.}{Wrong Perception} \newline
Inspecting A2 and B1 z-axis image crops \newline
\tann{annCol9}{img=Image.open("/mnt/data/T3\_sample1\_row4\_vs\_73\_query\_a\_image\_2.png") crop=img.crop((75,130,160,320)).resize((255,570)) crop.save('/mnt/data/a2\_zaxis\_crop.png') img=Image.open("/mnt/data/T3\_sample1\_row4\_vs\_73\_query\_b\_image\_1.png") crop=img.crop((155,130,230,360)).resize((225,690)) crop.save('/mnt/data/b1\_zaxis\_crop.png')}{Tool Use} \newline
Analyzed image \newline
Output image \newline
Analyzed image \newline
Output image \newline
\tann{annCol10}{Examining z-axis positioning for block compositions In A2, the z-axis seems to pass through the front-right region of the left-front cube, while in B1, it could be near the left boundary of the tall pillar. \textit{[[...trimmed output...]]}
% The task seems to focus on comparing shapes based on block composition rather than precise axis positioning. It might involve a 3D set operation where objects are aligned by their own grid axes. The origin could be the center of the bounding box, and we can still compare structures in the images. Approximating coordinates with set intersection and axes interpretation The images likely show the orientation of objects but don't provide exact coordinates. I'll use the set intersection approach to approximate coordinates based on the axes' placement, considering the origin. The dashed z-axis could pass through cube centers or edges, depending on the chosen origin. I'll focus on comparing positions relative to axes and identify voxels that intersect with the z-axis. Considering axes and shape alignment for shared blocks The dashed axes might be drawn independently of the object, showing general orientation rather than exact coordinates. In this case, how the shapes align relative to each other is more important than specific positions. The focus seems to be on comparing shared blocks between the first and last images, based on similarities in shape after adjusting positions. Although axes give hints, the real task might be comparing by composition rather than translation. Comparing object A and B structures Objects A and B seem to share a core structure. A has a horizontal top slab with supports and lower central blocks, while B has a similar top slab but with a tall vertical column. When comparing A1 and B2 from the same view, both appear to have a top row of 4 cubes, suggesting identical T-shaped footprints for A and B. Identifying shared and unique features between A and B A and B share a similar T-shaped top structure, but differ in vertical supports. A has two 2-high supports and lower blocks, while B has one tall column. The lower overlaps between them are likely where B's pillar matches one of A's lower blocks. Based on the locations, there seems to be one block of overlap. Discussing object A and B's structure and overlap A has extra blocks: a left support and two lower bridge blocks. B's lower pillar extends down to z=4, adding 3 extra blocks. The shared structure totals 7 blocks, with 3 blocks unique to A and 3 to B, making sense if B's pillar height is 5. 
It seems plausible, based on B1 crop.}{Wrong Perception} \newline
Visualizing B2 pillar location and height \newline
\tann{annCol9}{img=Image.open("/mnt/data/T3\_sample1\_row4\_vs\_73\_query\_b\_image\_2.png").convert("RGB") crop=img.crop((215,145,330,365)).resize((345,660)) draw=ImageDraw.Draw(crop) for y in range(0,660,50): draw.line((0,y,345,y),fill=(255,0,0),width=1) draw.text((5,y+2),str(y),fill=(255,0,0)) crop.save('/mnt/data/b2\_pillar\_grid.png')}{Tool Use} \newline
Analyzed image \newline
Output image \newline
Clarifying B2 grid structure and A's lower blocks \newline
\tann{annCol10}{B2 grid shows its top cube's face from y=0-150, with the underside around y=250. 
\textit{[[...trimmed output...]]}
% A vertical pillar starts from y=260-350 with approximately four lower cubes extending from there. B therefore has 10 cubes. As for A, the central lower strip may involve two blocks, but with a T-shaped top, it might have more. Counting blocks in A and B In A, the count goes as follows: Top shape is a T, totaling 6 blocks. Left and right vertical columns each add 1 block, so that's +2. The central lower strip shows two blocks in A2, so +2 more, bringing the total to 10. For B, the long underside ledge seems to replace the central lower strip, but no visible gray lower blocks appear in B2. Analyzing overlap in A and B In the same view, B2's pillar lines up exactly beneath the right side of the top shape, where A1's right stack is. The right stack in A has a vertical face, and B2's pillar also aligns vertically. So, there's likely a lower overlap. The central lower blocks of A don't overlap with B's pillar, since A's lower strips are positioned differently. Comparing the views, A's right stack seems near the center-right, and B's pillar matches that position. Orientation comparison of A and B In the flipped Y direction, a positive Y coordinate might switch front and back. The right stack in A stays in the same position for both views. A2's right stack corresponds to A1's right stack. For B, the pillar could be at a positive X and Y. If B's orientation matches A's, its right stack could correspond to A2, but in B1, the pillar is at the far left/front. Aligning A and B's coordinate systems Flipping the Y-axis changes how the X-axis appears, altering projections. The right stack in A1 aligns with the Z-axis, and the pillar in B2 might align similarly. In A2, flipping the Y-axis shifts the projection, but A's lower block at the origin should still be left-front rather than right. Inferring voxel positions in A and B The overlap seems to be between B's pillar and A's central lower block, not the right stack. To represent voxel sets, we might define positions as integer cells starting at the origin. The axes likely pass through the origin. In B2, the tall pillar sits to the right of the Z-axis. Aligning coordinates and voxel positions The pillar may be positioned at x=0, Defining B and A grids with axes positioning In B1, the X axis extends right through the upper front edge of the right cube, while the Y axis goes upper-left through the left edge, possibly at the origin of the tall pillar. The rectangle extends +X and +Y from the origin, forming a 3x2 shape. In A2, the Y axis extends through the top/back, and the Z axis is near the left/front. Mapping top intersection shapes in A and B grids The top shape of A extends from the origin along +X and +Y, possibly with one negative X cell. A has a bar along the X axis at y=0 and a stem along the Y axis at x=1. The intersection of A's top with B's rectangle is likely at 4, not 6. The visual Analyzing A vs B top view and intersections B2's top consists of a left cube, central strip, and a 2x2 block, forming a rectangle but not quite a T-shape, similar but not identical to A. The intersection could be 4, with totals of 10 each for A and B. If there's overlap, intersection becomes 5, with 5 in both A and B. Let's visually map A2 and B1 top footprints, checking the differences, focusing on the intersection. Analyzing A2 top crop and axis alignment In A2, the X axis dashed line starts at the top-front edge of the rightmost cube, likely coinciding with the row at y=0, with the origin near the left-front block, possibly at (x=0, y=0). The row extends from negative X to positive X. The Y axis dashed line passes just left of the front-left block and extends into the branch, indicating the stem starts at the origin, with cells along X=0. Considering cube positioning and overlaps between A and B In A, if the top block is at (x=0, y=0), there doesn't appear to be a lower block at the same coordinate, except for the stack. A lower strip with two blocks at z=1 seems located at (x=0,1; y=-1). So, B's lower pillar at (x=0, y=0) wouldn't overlap A's lower, leading to no lower overlap. The intersection would be 4, with only A and B getting 6 each. Exploring stack positions and potential overlaps between A and B A seems to have vertical stacks on both sides (left and right) while B might overlap A's left stack at (x=0, y=0). A1's left stack might be at x=-1, y=0, with a lower portion. The final answer could be \{4,6, Mapping A's lower block positions in A1 Using A1's view with Y positive down-right, the row along X seems horizontal from left to right. The branch along Y appears at the top-right, with its stem at negative Y. The left stack is at (x=-1, y=0) while the right stack should be placed closer to the center-right. I'll check precise positions next. Evaluating A's T shape and stem coordinates It seems like A's top T at coordinates x=-1...2, y=0, with a stem along y=-1,-2 at x=1. In A1, the stem reaches right/up with negative Y. In A2, where positive Y goes up-left, the stem might be in the upper center. The Y-axis labels and camera angles could affect this. I'll double-check this mapping. Checking for object rotation and projection differences It looks like Y-axis labeling differs between A1 and A2, with Y as positive upper-left in A2 but negative in A1. The object might be rotated or translated for each view, not simply mirrored. I'll double-check whether the two images are actually the same object or different angles, as the user mentions grouping them. Verifying object orientations and structure I need to verify the match between A1 and A2. A1 shows a top right-back protrusion, while A2's is top-center, indicating rotation. I also notice the Y-positive side in A1 and Y-negative in A2, which helps infer coordinates. At this point, I can finalize the JSON data, assuming a reasonable model for the objects, given their shared features. Assessing object footprints and overlaps It seems that A1 and A2 aren't quite 3x2 as expected. A1's top crop suggests a likely 6-block arrangement; however, A2 tops at 4 along X with a 3-block central column. This implies the intersection might be smaller than 6, potentially 4 blocks based on their coordinates. Lower overlaps depend on how B's pillar aligns with A's lower blocks. Assessing overlap and intersections In A2, the front-left block is one-high with no lower block, which means no lower overlap with B. The A1 configuration could have the right stack, but based on the same view orientation, I believe the overlap is zero. 
The intersection likely stays at 4, adding to both objects' remaining blocks. So, no lower overlap for B's pillar either.}{Wrong Perception}

```python \newline
\{ \newline
'answer intersection': 4, \newline
'answer only a': 6, \newline
'answer only b': 6, \newline
\} \newline
```
\end{tcolorbox}
\begin{tcolorbox}[breakable,enhanced,colback=red!4,colframe=red!55!black,boxrule=0.4pt,arc=1pt,left=4pt,right=4pt,top=3pt,bottom=3pt,fonttitle=\footnotesize\bfseries,coltitle=black,colbacktitle=red!12,title={\tpicon{gemini_flash_icon.png}~Gemini-3-Flash\hfill answer: (0,15,13)\tickno}]
\footnotesize\raggedright
To find the precise block counts and structural differences between Object A and Object B, we can reconstruct their 3D layouts by establishing a consistent grid system based on the coordinate axes (\$X, Y, Z\$) shown in the images.

\#\#\# 1. Structure Reconstructions

\#\#\#\# Object A (`query\_a\_image\_1` \& `query\_a\_image\_2`)

By analyzing the layout along the \$X\$-axis (width), \$Y\$-axis (depth), and \$Z\$-axis (height), Object A forms a U-like overhead layout with two layers in height.

* **Top Layer (\$Z = 2\$):** * There are two distinct wings at opposite corners: one block at the front-left and two blocks forming a line at the back-right. \newline
* **Bottom Layer (\$Z = 1\$):** \newline
* A continuous platform connecting the sides: \$4\$ blocks in the middle row, plus additional support blocks extending forward and backward.

\tann{annCol10}{* **Total Block Count for Object A:** **15 blocks**}{Wrong Perception}

---

\#\#\#\# Object B (`query\_b\_image\_1` \& `query\_b\_image\_2`)

Object B has a flat horizontal platform at the top, supported by a long vertical pillar extending downwards.

* **Top Platform (\$Z = 5\$):** \newline
* An L-shaped or T-shaped arrangement of blocks forming a flat plate, containing a total of **9 blocks**.

* **Vertical Pillar (\$Z = 1\$ to \$4\$):** \newline
* A straight column of blocks supporting the upper structure directly underneath one of the corner nodes, adding **4 blocks**.

\tann{annCol10}{* **Total Block Count for Object B:** **13 blocks** }{Wrong Perception} \newline
---

\#\#\# 2. Composition Comparison

\tann{annCol10}{Because Object A and Object B are two entirely distinct spatial geometric structures (different spatial extents, height profiles, and configurations), they do not share any common block coordinates or overlapping structural sub-components in a unified reference frame. * **Intersection (Shared Blocks):** 0 * **Unique to Object A:** 15 * **Unique to Object B:** 13 }{Wrong Perception} \newline
```json \newline
\{ \newline
'answer intersection': 0, \newline
'answer only a': 15, \newline
'answer only b': 13, \newline
\}

```
\end{tcolorbox}
\begin{tcolorbox}[breakable,enhanced,colback=red!4,colframe=red!55!black,boxrule=0.4pt,arc=1pt,left=4pt,right=4pt,top=3pt,bottom=3pt,fonttitle=\footnotesize\bfseries,coltitle=black,colbacktitle=red!12,title={\tpicon{gemini_pro_icon.png}~Gemini-3.1-Pro\hfill answer: (6,4,3)\tickno}]
\footnotesize\raggedright
Defining the Objective

I have clarified the core objective: I must compare block-based 3D objects from 2D images.

Establishing Coordinates

I have carefully defined a coordinate system relative to the block grid shown in Image 1 and its origin.

\textit{[[...trimmed output...]]}

% Revisiting Axis Orientation

% I've re-examined the axes, resolving the origin's location and block counts in the top layer.

% Mapping the Blocks

% I have successfully established a 3D coordinate system to map the block structure shown in the image.

% Defining the Origin

% I have successfully established a 3D coordinate system to map the top layer blocks.

% Defining the Rotation

% I've worked out the coordinate system for a rotated view, defining block positions with new axes.

% Tracing the Blocks

% I am now tracing and mapping block positions in detail, using a temporary coordinate system.

% I've successfully mapped blocks in the top and first layer, and am currently verifying lower layers.

% Analyzing the Layers

% I have determined the blocks in both the top and the bottom layer based on Image 2, verifying the block positions.

% Clarifying the Axes

% I've finally clarified the axes in Image 1, now correctly oriented with X as left-down, Y as right-down, and Z down.

% Defining Isometric Axes

% I've confirmed the Z, X, and Y axis orientations in the isometric view of Image 1, using block edge angles.

% Establishing Global Coordinates

% I've established global coordinates: +X is Right-Up, +Y is Left-Up, and +Z is down, across both images.

% Defining Object-Based Axes

% I've defined local object coordinates and, via rotation analysis, clarified the coordinate transformation between the two images.

% Constructing the Object

% I am now building the object's block map, verifying coordinates against both Image 1 and Image 2.

% Verifying Axis Mapping

% I'm now cross-validating axes and block positions, confirming the relationship between image coordinates.

% Verifying Orientation

% I've resolved the precise block layout using both images, confirming my initial coordinate assumptions.

% Analyzing Image 1

% I'm now identifying blocks in Image 1 by tracing top faces and comparing them to a model.

% Tracing the Blocks

% I have traced and fully defined the top layer blocks, confirming a five-block layout across both images.

% Defining Object's Structure

% I have now derived both object layers, mapping the blocks and verifying coordinates against images.

% Re-evaluating Block Layout

% I am now re-evaluating Image 2's block layout, considering relative positions of blocks and neighbors.

% Matching the Layout

% I have directly matched Image 2's structure to my model, clarifying block coordinates precisely.

% Tracing the Blocks

% I have successfully traced and defined the entire block structure in Image 1, clarifying the layout.

% Confirming the Top Layer

% I have precisely confirmed the top layer block layout, resolving coordinates against Image 1 and 2.

% Mapping Image 2

% I am now meticulously mapping blocks in Image 2 to our coordinate system, validating and clarifying block placements.

% Confirming the Structure

% I have now validated that this is a two-layer solid object, confirming all ten blocks are present.

% Verifying Completeness

% I have confirmed no blocks are missing in A's bottom layer, also resolving its full 10-block structure.

% Defining Block Columns

% I've traced the columns in Image 3, determining block counts for each coordinate pair.

% Determining Column Heights

% I'm now determining individual block column counts from edges, re-reading Image 3 line segments.

% Tracing the Columns

% I'm now tracing the structure in the new image, confirming the column counts in the isometric view.

% Verifying Column Count

% I've traced the columns in both Image 3 and 4, confirming a column height of five blocks.

% Mapping the Columns

% I've traced the column structure in Image 4, matching it to the established coordinate system from Image 1 and Image 3.

% Revising Axis Orientation

% I've reevaluated the axes, establishing that the coordinate system aligns with Right-Up for -X and Left-Up for -Y.

% Analyzing Block Thickness

% I've determined Object B's top layer is one block thick, except for a column with two.

% Revising Block Thickness

% I've re-evaluated the Image 4 isometric view and have resolved how to determine block thicknesses.

% Differentiating Object B

% I've determined Object B has a 5-block top layer with a 5-block column at (0,0), with no hidden blocks.

% Verifying Hidden Blocks

% I have deduced Object B's structure, confirming a 9-block layout with a central 4-block column and a strict top layer.

% Defining Object B

% I've precisely defined Object B's coordinate mapping, including verifying the blocks' depths and locations.

% Calculating Block Differences

% I have precisely calculated the block differences between the two objects, determining 6 shared blocks.

% Revising Coordinate Systems

% I am now carefully establishing the precise isometric coordinate system for all image interpretations.

% Verifying Block Thickness

% I have successfully re-verified both objects, determining Object B is one block thick, while A is two.

% Verifying Structure Completeness

% I have now proven both objects are solid, resolving the precise difference in block counts between them.

% Confirming Isometric View

% I have successfully traced and confirmed that no blocks are hidden in object B in both directions.

Finalizing the Tally

I have re-validated the block counts to avoid errors, confirming the block intersections for the response.

JSON \newline
\tann{annCol10}{\{ 'answer intersection': 6, 'answer only a': 4, 'answer only b': 3, \}}{Wrong Perception} \newline
Verifying Column Heights

I'm now carefully re-verifying block counts, re-checking the image lines to ensure accurate height values.

To determine the difference in the block compositions of Object A and Object B, we first need to reconstruct their 3D structures from the provided perspective images.

**1. Reconstruct Object A (Images 1 \& 2)**

\tann{annCol10}{* **Top Layer Shape:** By observing Image 2 (viewed from the back), we can see a flat top layer. Identifying the blocks relative to the axis intersection (let's call it the origin), we see a \$2 \textbackslash\{\}times 2\$ square of blocks, with one additional block extending from one of the sides. Let's set the coordinates \$(X, Y)\$ for this layer: * Origin block at \$(0,0)\$. * Neighbors forming the \$2 \textbackslash\{\}times 2\$: \$(1,0)\$, \$(0,1)\$, and \$(1,1)\$. * The extending block is at \$(0,2)\$. * This gives a 5-block "P" or "d" shape for the top layer. This perfectly matches the perspective in Image 1 as well. * **Thickness:** Looking at both Image 1 and Image 2, every visible block in the top layer has exactly one block directly underneath it. The structure is a uniform 2-block-thick extrusion of the top shape. * **Total blocks in A:** 5 (top layer) + 5 (bottom layer) = **10 blocks**. }{Wrong Perception} \newline
**2. Reconstruct Object B (Images 3 \& 4)**

\tann{annCol10}{* **Top Layer Shape:** Image 3 and Image 4 show an object with the exact same 5-block top layer profile as Object A: a \$2 \textbackslash\{\}times 2\$ section plus one extending block. * **Thickness \& Column:** * Unlike Object A, the top layer of Object B is only **1 block thick** for most of its structure. You can clearly see the empty space (hollow underside) beneath the extending arms in Image 4. * However, at the origin \$(0,0)\$, there is a single long vertical column extending downwards. * Counting the visible block faces on this vertical column in both Image 3 and Image 4 reveals it is 5 blocks tall in total (1 top block + 4 blocks extending beneath it). * **Total blocks in B:** 5 (top layer) + 4 (extra blocks in the column) = **9 blocks**.}{Wrong Perception}

**3. Compute the Differences** \newline
Let's align them on the same coordinate grid to compare: \newline
\tann{annCol10}{ * **Intersection (Shared blocks):** Both objects share the entire top layer (5 blocks). They also both share the first block extending down at the origin \$(0,0,1)\$ because Object A is 2 blocks thick everywhere, and Object B's column passes through that space. * Shared = 5 (top layer) + 1 (first block under origin) = **6 blocks**. * **Only A:** Object A has a full second layer, meaning it has blocks underneath the other 4 top-layer blocks. Object B is hollow there. * Only A = 10 (Total A) - 6 (Shared) = **4 blocks**. * **Only B:** Object B's column at the origin extends 3 blocks deeper than Object A's 2-block thickness. * Only B = 9 (Total B) - 6 (Shared) = **3 blocks**.}{Wrong Perception}

``` \newline
\{ \newline
'answer intersection': 6, \newline
'answer only a': 4, \newline
'answer only b': 3, \newline
\}

```
\end{tcolorbox}

\subsubsection{T4 Color Count}
\begin{table}[H]
\centering
\footnotesize
\setlength{\tabcolsep}{1pt}
\renewcommand{\arraystretch}{1.2}
\begin{tabular}{*{9}{>{\centering\arraybackslash}p{\dimexpr\textwidth/9-2\tabcolsep\relax}}}
\toprule
\multicolumn{9}{@{}l@{}}{\itshape ``\ldots{}Your task is to count the number of unique colors in the object\ldots{}''}\\[0.3mm]
\multicolumn{9}{@{}c@{}}{\begin{tabular}{*{2}{c}}\includegraphics[width=0.450\textwidth,height=1.25in,keepaspectratio]{images/app_qual_traces/T4_sample1_row9_query_image_1.png} & \includegraphics[width=0.450\textwidth,height=1.25in,keepaspectratio]{images/app_qual_traces/T4_sample1_row9_query_image_2.png}\end{tabular}}\\[0.5mm]
\textbf{GT} & \tpicon{qwen_icon.png} & \tpicon{gemma_icon.png} & \tpicon{glmv_icon.png} & \tpicon{kimi_icon.png} & \tpicon{grok_icon.png} & \tpicon{gpt_icon.png} & \tpicon{gemini_flash_icon.png} & \tpicon{gemini_pro_icon.png}\\
7 & 6\tickno & 6\tickno & 6\tickno & 10\tickno & 6\tickno & 7\tickok & 6\tickno & 6\tickno\\
\bottomrule
\end{tabular}
\caption{T4 Color Count.}
\label{tab:qual_trace_t4}
\end{table}
\noindent\textbf{Thinking traces.}\par\smallskip
\begin{tcolorbox}[breakable,enhanced,colback=red!4,colframe=red!55!black,boxrule=0.4pt,arc=1pt,left=4pt,right=4pt,top=3pt,bottom=3pt,fonttitle=\footnotesize\bfseries,coltitle=black,colbacktitle=red!12,title={\tpicon{qwen_icon.png}~Qwen3.5-27B\hfill answer: 6\tickno}]
\footnotesize\raggedright
The user wants me to count the unique colors in the 3D object shown in two images.

**Image 1 Analysis:** \newline
- I see a structure made of cubes. \newline
- Let's list the visible colors: \newline
- Top left: Blue cube on top of a purple cube. Wait, looking closely at the leftmost part. \newline
- Top face: Blue. \newline
- Front face: Purple. \newline
- Side face: Blue (partially visible). \newline
- \tann{annCol10}{Next to it (right): A purple cube.}{Wrong Perception} \newline
- Top face: Purple. \newline
- Front face: Purple. \newline
- Behind/Right of that: A yellow cube. \newline
- Top face: Yellow. \newline
- Further right/back: A green cube. \newline
- Top face: Green. \newline
- \tann{annCol10}{Below the green cube: A green cube.}{Wrong Perception} \newline
- Top face: Green. \newline
- Front face: Green. \newline
- To the right of the green cube: A yellow cube. \newline
- Top face: Yellow. \newline
- \tann{annCol10}{Below the yellow cube (front): A magenta cube.}{Wrong Perception} \newline
- Top face: Magenta. \newline
- Front face: Magenta. \newline
- Below the magenta cube: A yellow cube. \newline
- Front face: Yellow. \newline
- To the right of the magenta cube: A red cube. \newline
- Top face: Red. \newline
- Front face: Red. \newline
- Below the red cube: A blue cube. \newline
- Front face: Blue.

Let's refine the list of colors seen in Image 1: \newline
- Blue (top left, bottom right) \newline
- \tann{annCol10}{Purple (front left)}{Wrong Perception} \newline
- Yellow (top middle, front bottom middle) \newline
- Green (top right back, front middle) \newline
- Magenta (front middle right) \newline
- Red (front right)

\tann{annCol10}{So far: Blue, Purple, Yellow, Green, Magenta, Red. That's 6 colors.}{Wrong Perception}

**Image 2 Analysis:** \newline
- This is a different angle. Let's see what new colors or confirmations we get. \newline
- Top left back: Red cube. \newline
- Top face: Red. \newline
- Front face: Red. \newline
- Next to it (right): Magenta cube. \newline
- Top face: Magenta. \newline
- Below the red cube: Blue cube. \newline
- Front face: Blue. \newline
- \tann{annCol1}{Below the magenta cube: Yellow cube.}{Color Confusion} \newline
- Top face: Yellow. \newline
- Front face: Yellow. \newline
- \tann{annCol1}{Next to the yellow cube (right): Green cube.}{Color Confusion} \newline
- Top face: Green. \newline
- Below the green cube: Purple cube. \newline
- Front face: Purple. \newline
- \tann{annCol1}{Next to the green cube (right): Yellow cube.}{Color Confusion} \newline
- Top face: Yellow. \newline
- Below the yellow cube: Yellow cube (partially visible underneath). \newline
- To the right of the yellow cube: Purple cube. \newline
- Top face: Purple. \newline
- \tann{annCol10}{Below the purple cube: Blue cube.}{Wrong Perception} \newline
- Top face: Blue. \newline
- Front face: Blue. \newline
- Below the blue cube: Purple cube. \newline
- Front face: Purple.

Let's list the colors seen in Image 2: \newline
- Red \newline
- Magenta \newline
- Blue \newline
- Yellow \newline
- Green \newline
- Purple

\tann{annCol10}{This confirms the same set of colors: Red, Magenta, Blue, Yellow, Green, Purple.}{Wrong Perception}

**Reconstructing the object to be sure:** \newline
Let's try to map the blocks. \newline
\tann{annCol10}{It looks like a 2x4 or similar grid structure, maybe with some height variations.}{Wrong Perception}

\tann{annCol8}{Let's look at Image 1 again.}{Reiterating} \newline
- Leftmost column: Top is Blue, Bottom is Purple. \newline
- Next column: Top is Purple. Wait, looking at the connection. \newline
- The blue/purple stack is connected to a purple block. \newline
\tann{annCol1}{ - Then a yellow block.}{Color Confusion} \newline
- Then a green block. \newline
- Then a yellow block. \newline
- Then a red block. \newline
- Under the red block is a blue block. \newline
- \tann{annCol10}{Under the yellow block (middle right) is a magenta block.}{Wrong Perception} \newline
- \tann{annCol1}{Under the magenta block is a yellow block. }{Color Confusion} \newline
\tann{annCol8}{Let's look at Image 2 again.}{Reiterating} \newline
- Back left: Red on top of Blue. \newline
- \tann{annCol10}{Next to it: Magenta on top of Yellow. - Next to that: Green on top of Purple. - Next to that: Yellow on top of Yellow (maybe?). - Far right: Purple on top of Blue on top of Purple.}{Wrong Perception}

\tann{annCol8}{Wait, let's look at the structure more carefully.}{Reiterating} \newline
\tann{annCol10}{Image 1 shows a "snake" like shape. Image 2 shows a more blocky shape.}{Wrong Perception}

Let's assume a grid. \newline
\tann{annCol8}{Let's look at the colors again.}{Reiterating} \newline
\tann{annCol0}{I have to give the solution based on the reasoning directly now.}{Budget Hit}
\end{tcolorbox}
\begin{tcolorbox}[breakable,enhanced,colback=red!4,colframe=red!55!black,boxrule=0.4pt,arc=1pt,left=4pt,right=4pt,top=3pt,bottom=3pt,fonttitle=\footnotesize\bfseries,coltitle=black,colbacktitle=red!12,title={\tpicon{grok_icon.png}~Grok-4.20\hfill answer: 6\tickno}]
\footnotesize\raggedright
The problem asks to count the number of unique colors in a 3D object made of blocks, shown in two perspective images from different angles. \newline
I see the object made of blocks in two images, and I need to count the unique colors. \tann{annCol10}{From the first image, the colors are blue, purple, yellow, green, possible magenta or pink, and red.}{Wrong Perception} \tann{annCol10}{The second image shows the same colors: red, magenta, yellow, green, purple, blue.}{Wrong Perception}No other colors like cyan or orange appear. The purple is a deep purple, different from the bright magenta. The greens look the same, no shading issues. \tann{annCol10}{So, the unique colors are blue, purple, yellow, green, red, and magenta---that's six in total.}{Wrong Perception}
\end{tcolorbox}
\begin{tcolorbox}[breakable,enhanced,colback=green!4,colframe=green!50!black,boxrule=0.4pt,arc=1pt,left=4pt,right=4pt,top=3pt,bottom=3pt,fonttitle=\footnotesize\bfseries,coltitle=black,colbacktitle=green!14,title={\tpicon{gpt_icon.png}~GPT-5\hfill answer: 7\tickok}]
\footnotesize\raggedright
Analyzing image colors \newline
I need to focus on analyzing the images. I want to count unique colors across a set and figure out which colors appear in both views. The color palette includes blue, purple, magenta, green, yellow, red, and gold. I think the top central part might have yellow or gold, so I'll check the RGB values and inspect the pixels carefully. I'll load the images to get the dominant, unique colors. \newline
Identifying unique colors in image set \newline
\tann{annCol9}{from PIL import Image import numpy as np, collections, os, matplotlib.pyplot as plt paths=["/mnt/data/T4\_sample1\_row9\_query\_image\_1.png","/mnt/data/T4\_sample1\_row9\_query\_image\_2.png"] for p in paths: img=Image.open(p).convert("RGB") arr=np.array(img) \# get unique colors counts colors, counts=np.unique(arr.reshape(-1,3), axis=0, return\_counts=True) \# sort by count desc order=np.argsort(-counts) print(os.path.basename(p), img.size, len(colors)) for c, cnt in zip(colors[order][:30], counts[order][:30]): print(tuple(c), cnt) print() T4\_sample1\_row9\_query\_image\_1.png (409, 409) 1388 (np.uint8(255), np.uint8(255), np.uint8(255)) \textit{[[...trimmed output...]]}}{Tool Use}
% \tann{annCol9}{from PIL import Image import numpy as np, collections, os, matplotlib.pyplot as plt paths=["/mnt/data/T4\_sample1\_row9\_query\_image\_1.png","/mnt/data/T4\_sample1\_row9\_query\_image\_2.png"] for p in paths: img=Image.open(p).convert("RGB") arr=np.array(img) \# get unique colors counts colors, counts=np.unique(arr.reshape(-1,3), axis=0, return\_counts=True) \# sort by count desc order=np.argsort(-counts) print(os.path.basename(p), img.size, len(colors)) for c, cnt in zip(colors[order][:30], counts[order][:30]): print(tuple(c), cnt) print() T4\_sample1\_row9\_query\_image\_1.png (409, 409) 1388 (np.uint8(255), np.uint8(255), np.uint8(255)) 116895 (np.uint8(128), np.uint8(0), np.uint8(128)) 8338 (np.uint8(0), np.uint8(0), np.uint8(255)) 7074 (np.uint8(255), np.uint8(0), np.uint8(255)) 6441 (np.uint8(0), np.uint8(128), np.uint8(0)) 6028 (np.uint8(255), np.uint8(0), np.uint8(0)) 5222 (np.uint8(0), np.uint8(0), np.uint8(0)) 4809 (np.uint8(255), np.uint8(215), np.uint8(0)) 4388 (np.uint8(255), np.uint8(255), np.uint8(0)) 2404 (np.uint8(127), np.uint8(0), np.uint8(127)) 116 (np.uint8(231), np.uint8(231), np.uint8(231)) 108 (np.uint8(31), np.uint8(31), np.uint8(31)) 103 (np.uint8(14), np.uint8(0), np.uint8(14)) 63 (np.uint8(100), np.uint8(0), np.uint8(100)) 58 (np.uint8(0), np.uint8(0), np.uint8(3)) 58 (np.uint8(109), np.uint8(0), np.uint8(109)) 56 (np.uint8(66), np.uint8(0), np.uint8(66)) 55 (np.uint8(77), np.uint8(0), np.uint8(77)) 54 (np.uint8(48), np.uint8(0), np.uint8(48)) 54 (np.uint8(250), np.uint8(0), np.uint8(0)) 53 (np.uint8(209), np.uint8(0), np.uint8(209)) 52 (np.uint8(0), np.uint8(0), np.uint8(250)) 52 (np.uint8(0), np.uint8(0), np.uint8(97)) 51 (np.uint8(200), np.uint8(200), np.uint8(200)) 51 (np.uint8(15), np.uint8(0), np.uint8(15)) 51 (np.uint8(67), np.uint8(0), np.uint8(0)) 51 (np.uint8(18), np.uint8(15), np.uint8(0)) 50 (np.uint8(172), np.uint8(0), np.uint8(172)) 50 (np.uint8(0), np.uint8(0), np.uint8(131)) 50 (np.uint8(114), np.uint8(96), np.uint8(0)) 49 T4\_sample1\_row9\_query\_image\_2.png (409, 409) 1357 (np.uint8(255), np.uint8(255), np.uint8(255)) 113550 (np.uint8(128), np.uint8(0), np.uint8(128)) 11897 (np.uint8(0), np.uint8(128), np.uint8(0)) 8722 (np.uint8(0), np.uint8(0), np.uint8(255)) 7674 (np.uint8(255), np.uint8(215), np.uint8(0)) 5458 (np.uint8(0), np.uint8(0), np.uint8(0)) 5017 (np.uint8(255), np.uint8(0), np.uint8(0)) 3506 (np.uint8(255), np.uint8(255), np.uint8(0)) 3457 (np.uint8(255), np.uint8(0), np.uint8(255)) 2226 (np.uint8(231), np.uint8(231), np.uint8(231)) 109 (np.uint8(31), np.uint8(31), np.uint8(31)) 108 (np.uint8(1), np.uint8(0), np.uint8(1)) 79 (np.uint8(0), np.uint8(1), np.uint8(0)) 67 (np.uint8(127), np.uint8(0), np.uint8(127)) 63 (np.uint8(125), np.uint8(0), np.uint8(125)) 63 (np.uint8(34), np.uint8(0), np.uint8(34)) 58 (np.uint8(0), np.uint8(34), np.uint8(0)) 58 (np.uint8(65), np.uint8(0), np.uint8(65)) 57 (np.uint8(254), np.uint8(254), np.uint8(0)) 57 (np.uint8(28), np.uint8(0), np.uint8(28)) 57 (np.uint8(3), np.uint8(0), np.uint8(0)) 56 (np.uint8(0), np.uint8(0), np.uint8(250)) 56 (np.uint8(77), np.uint8(0), np.uint8(77)) 56 (np.uint8(0), np.uint8(77), np.uint8(0)) 56 (np.uint8(114), np.uint8(0), np.uint8(114)) 55 (np.uint8(0), np.uint8(28), np.uint8(0)) 55 (np.uint8(0), np.uint8(0), np.uint8(3)) 54 (np.uint8(0), np.uint8(0), np.uint8(131)) 53 (np.uint8(0), np.uint8(0), np.uint8(97)) 53 (np.uint8(47), np.uint8(40), np.uint8(0)) 53}{Tool Use}

``` \newline
\{ \newline
'answer': 7, \newline
\} \newline
```
\end{tcolorbox}
\begin{tcolorbox}[breakable,enhanced,colback=red!4,colframe=red!55!black,boxrule=0.4pt,arc=1pt,left=4pt,right=4pt,top=3pt,bottom=3pt,fonttitle=\footnotesize\bfseries,coltitle=black,colbacktitle=red!12,title={\tpicon{gemini_flash_icon.png}~Gemini-3-Flash\hfill answer: 6\tickno}]
\footnotesize\raggedright
To determine the number of unique colors in the 3D object, let's identify all the distinct colors visible across both views based on the allowed list of colors:

1. **Blue** (Visible on the far left top and bottom right in Image 1; right side in Image 2) \newline
2. **Purple** (Visible on the left side and top-left block structure in both images) \newline
3. **Yellow** (Visible in the central grid area and bottom support blocks) \newline
4. **Green** (Visible in the central grid area) \newline
5. **Magenta** (Visible on the front protruding block in Image 1 and the top back row in Image 2) \newline
6. **Red** (Visible on the front right block in Image 1 and the top-left back block in Image 2)

All other variations are due to shading/perspective. \tann{annCol10}{No other colors from the list (such as cyan, orange, orchid, teal, slategray, or gold) are present.}{Wrong Perception}

```json \newline
\{ \newline
'answer': 6, \newline
\}

```
\end{tcolorbox}
\begin{tcolorbox}[breakable,enhanced,colback=red!4,colframe=red!55!black,boxrule=0.4pt,arc=1pt,left=4pt,right=4pt,top=3pt,bottom=3pt,fonttitle=\footnotesize\bfseries,coltitle=black,colbacktitle=red!12,title={\tpicon{gemini_pro_icon.png}~Gemini-3.1-Pro\hfill answer: 6\tickno}]
\footnotesize\raggedright
Assessing Unique Colors

I've determined the limited color palette and started visually examining the first perspective view for color identification.

Identifying Color Correspondences

\tann{annCol10}{I've confirmed the same six colors exist across both images, solidifying my understanding of the palette.}{Wrong Perception}

```json \newline
\{ \newline
"answer": 6 \newline
\}

```
\end{tcolorbox}

\subsubsection{T5 Color Distribution}
\begin{table}[H]
\centering
\footnotesize
\setlength{\tabcolsep}{1pt}
\renewcommand{\arraystretch}{1.2}
\begin{tabular}{*{9}{>{\centering\arraybackslash}p{\dimexpr\textwidth/9-2\tabcolsep\relax}}}
\toprule
\multicolumn{9}{@{}l@{}}{\itshape ``\ldots{}Your task is to give the color distribution in the object\ldots{}''}\\[0.3mm]
\multicolumn{9}{@{}c@{}}{\begin{tabular}{*{2}{c}}\includegraphics[width=0.450\textwidth,height=1.25in,keepaspectratio]{images/app_qual_traces/T5_sample1_row90_query_image_1.png} & \includegraphics[width=0.450\textwidth,height=1.25in,keepaspectratio]{images/app_qual_traces/T5_sample1_row90_query_image_2.png}\end{tabular}}\\[0.5mm]
\textbf{GT} & \tpicon{qwen_icon.png} & \tpicon{gemma_icon.png} & \tpicon{glmv_icon.png} & \tpicon{kimi_icon.png} & \tpicon{grok_icon.png} & \tpicon{gpt_icon.png} & \tpicon{gemini_flash_icon.png} & \tpicon{gemini_pro_icon.png}\\
\threewrap{\cdC{2}&\cdY{2}&\cdM{3}\\\cdR{2}&\cdS{2}&\cdT{2}\\\cdGo{1}&\cdG{1}&} & \threewrap{\cdY{5}&\cdC{4}&\cdG{1}\\\cdM{5}&\cdR{3}&\cdT{2}\\\cdS{3}&&}\tickno & \threewrap{\cdY{3}&\cdC{4}&\cdG{1}\\\cdM{4}&\cdR{3}&\cdT{2}\\\cdS{3}&&}\tickno & \threewrap{\cdT{3}&\cdS{4}&\cdC{4}\\\cdY{4}&\cdM{5}&\cdR{3}\\\cdG{2}&&}\tickno & \threewrap{\cdY{6}&\cdC{8}&\cdG{1}\\\cdM{6}&\cdR{5}&\cdT{4}\\\cdS{4}&&}\tickno & \threewrap{\cdY{4}&\cdC{4}&\cdG{1}\\\cdM{4}&\cdR{2}&\cdT{2}\\\cdS{3}&&}\tickno & \threewrap{\cdR{2}&\cdGo{1}&\cdC{2}\\\cdM{3}&\cdG{1}&\cdY{2}\\\cdS{2}&\cdT{2}&}\tickok & \threewrap{\cdT{2}&\cdS{3}&\cdC{4}\\\cdY{3}&\cdM{4}&\cdR{2}\\\cdG{1}&\cdGo{1}&}\tickno & \threewrap{\cdT{1}&\cdC{2}&\cdS{2}\\\cdY{2}&\cdM{2}&\cdG{1}\\\cdR{3}&\cdGo{1}&}\tickno\\
\bottomrule
\end{tabular}
\caption{T5 Color Distribution.}
\label{tab:qual_trace_t5}
\end{table}
\noindent\textbf{Thinking traces.}\par\smallskip
\begin{tcolorbox}[breakable,enhanced,colback=red!4,colframe=red!55!black,boxrule=0.4pt,arc=1pt,left=4pt,right=4pt,top=3pt,bottom=3pt,fonttitle=\footnotesize\bfseries,coltitle=black,colbacktitle=red!12,title={\tpicon{glmv_icon.png}~GLM-4.6V-Flash\hfill answer: \tickno}]
\footnotesize\raggedright
Got it, let's tackle this problem step by step. First, I need to analyze both images and identify all the colors present, then count each color's blocks.

First, let's list the colors from the possible set: yellow, cyan, green, magenta, red, orange, orchid, teal, slategray, gold, blue, purple.

Looking at the first image:

- Teal (dark teal) block: leftmost, that's one. \newline
- Slategray (gray) block next to teal: second. \newline
- Then there's a cyan block above the gray one. \newline
- Yellow block next to cyan. \newline
- Then magenta, red, etc. \tann{annCol8}{Let's go through each visible block in first image:}{Reiterating}

First image blocks (from what I can see):

1. Teal (dark greenish-blue) - leftmost, single block. \newline
2. Slategray (gray) - adjacent to teal, same row. \newline
3. Cyan - above the gray block, same column as yellow. \newline
4. Yellow - to the right of cyan. \newline
5. Magenta - to the right of yellow. \newline
6. \tann{annCol10}{Red - below magenta.}{Wrong Perception} \newline
7. \tann{annCol10}{Another magenta - below red?}{Wrong Perception} \tann{annCol8}{Wait, no, let's parse the first image structure.}{Reiterating}

Wait, first image is a 3D arrangement. Let's think of layers. Maybe front, middle, back.

Alternatively, look at the second image to cross-reference.

Second image:

- Magenta block on top left. \newline
- \tann{annCol10}{Red below magenta. - Pink (magenta) below red?}{Wrong Perception} \tann{annCol8}{Wait, no, second image has:}{Reiterating}

\tann{annCol10}{Top row: magenta (left), then red, then... Wait, second image's top part: first column top is magenta, then red below it. Then middle column top is yellow, then cyan, etc. }{Wrong Perception} \newline
\tann{annCol8}{Let's list colors in each image: }{Reiterating} \newline
\textit{[[...trimmed output...]]} \newline
% First image colors observed:

% - Teal (teal) \newline
% - Slategray (gray) \newline
% - Cyan \newline
% - Yellow \newline
% - Magenta \newline
% - Red \newline
% - Green (the small green block) \newline
% - Another gray (the lower gray block) \newline
% - Another magenta (lower middle) \newline
% - Red (lower right) \newline
% - Yellow (rightmost lower) \newline
% - Cyan (rightmost top)

% Wait, let's count each color in first image:

% Teal: 1 (leftmost) \newline
% Slategray: 2 (the gray next to teal, and the lower gray block) \newline
% Cyan: 2 (the one above gray, and the rightmost top cyan) \newline
% Yellow: 2 (middle top yellow, and rightmost lower yellow) \newline
Magenta: 3 (middle right magenta, lower middle magenta, lower right magenta? \tann{annCol8}{Wait, no, first image: let's see the blocks:}{Reiterating}

\textit{[[...trimmed output...]]}

% From first image, visible blocks:

% - Teal (1) \newline
% - Gray (slategray) (2) \newline
% - Cyan (3) \newline
% - Yellow (4) \newline
% - Magenta (5) \newline
% - Red (6) \newline
% - Green (7) \newline
% - Gray (lower left) (8) \newline
% - Magenta (lower middle) (9) \newline
% - Red (lower right) (10) \newline
\tann{annCol1}{- Yellow (rightmost lower) (11)}{Color Confusion} \newline
- Cyan (rightmost top) (12)

\tann{annCol8}{Wait, but maybe some are overlapping. Let's check second image for consistency.}{Reiterating}

Second image colors:

- Magenta (top left) \newline
- \tann{annCol10}{Red (below magenta)}{Wrong Perception} \newline
- \tann{annCol10}{Pink (magenta) (below red)}{Wrong Perception} \newline
\textit{[[...trimmed output...]]} \newline
% - Yellow (middle top) \newline
% - Cyan (middle right) \newline
% - Teal (rightmost top) \newline
% - Slategray (middle right gray) \newline
% - Teal (rightmost middle) \newline
% - Green (lower middle green) \newline
% - Gray (lower right gray) \newline
% - Red (lower left red) \newline
% - Magenta (lower middle magenta) \newline
- \tann{annCol10}{Yellow (lower right yellow)}{Wrong Perception}

Now, let's map colors to each:

First, identify distinct colors present in either image. Let's list all unique colors from both images:

\tann{annCol10}{- Teal (dark teal) - Slategray (gray) - Cyan - Yellow - Magenta - Red - Green}{Wrong Perception}

\tann{annCol8}{Are there any others? Let's check:}{Reiterating} first image has green (the small green block), second image also has green. So colors are teal, slategray, cyan, yellow, magenta, red, green.

Now count each:

\tann{annCol10}{Teal: In first image, leftmost block (1). In second image, rightmost top and middle teal blocks: that's 2. So total teal: 1 + 2 = 3? Wait, no---wait, first image's teal is one block. Second image has two teal blocks (rightmost top and middle). So total teal blocks: 1 (first) + 2 (second) = 3. Slategray: First image has two gray blocks (the one next to teal, and the lower left gray). Second image has two gray blocks (middle right and lower right). So total slategray: 2 + 2 = 4? Wait, no---wait, first}{Wrong Perception}\tann{annCol0}{I have to give the solution based on the reasoning directly now.}{Budget Hit}
\end{tcolorbox}
\begin{tcolorbox}[breakable,enhanced,colback=red!4,colframe=red!55!black,boxrule=0.4pt,arc=1pt,left=4pt,right=4pt,top=3pt,bottom=3pt,fonttitle=\footnotesize\bfseries,coltitle=black,colbacktitle=red!12,title={\tpicon{grok_icon.png}~Grok-4.20\hfill answer: \tickno}]
\footnotesize\raggedright
The problem involves two images of a 3D object made of colored blocks, and I need to find the color distribution. \newline
\tann{annCol5}{I need to summarize the thinking trace for the user's query, but deliver it as my own thoughts directly answering the user.}{Harnessing}

\tann{annCol5}{The trace describes analyzing two 3D views of a colored block object to find the color distribution. \textit{[[...trimmed output...]]}
% It mentions colors like yellow, cyan, green, magenta, red, orange, orchid, teal,slategray, gold, gold, blue, purple. The trace tries to visualize the object as a polycube, listing visible colors and attempting to reconstruct the 3D model by assigning coordinates or counting visible blocks per color in each view. It notes the difficulty in distinguishing colors like bright yellow (possibly gold) vs regularyellow. It suggests listing blocks visible in each view and accounting for occlusions, recognizing that all blocks are surface-level with no internal hidden blocks. The output must be in the specified dict format with 'answer' key and color:count pairs. The example has orchid:10, orange:2, etc. So,in my final answer, I need to provide the distribution based on the trace's ideas, but since the actual images are missing, I'll infer a plausible distribution from the mentioned colors. The user's question includes "Car...(984 chars truncated)...t all visible colors from both views are included." It seems like the description is truncated, but the task is to give the color distribution. 
The internal reasoning is also truncated, but it provides clues.}{Harnessing}

From the trace, colors mentioned repeatedly are cyan, yellow, green, magenta, red, and others like teal, gray, slategray.

To arrive at a distribution, the trace starts counting in the firstimage: \tann{annCol10}{yellow:4, teal:1, gray:3, cyan:2, etc.}{Wrong Perception}

Then it says visible in view 1: teal1, gray3, cyan2, yellow4, and then mentions magenta, red, green.

\tann{annCol5}{Combining from both views, and since it's the same object, the totalis the union. The trace mentions "count the number of cubelets". \textit{[[...trimmed output...]]}
% It assumes each cube is uniformly colored, no mixed blocks. Towards the end, it says "it looks like a sort of snake or irregular 3D shape." But no specific counts are given in the trace. Since the trace doesn't provide exactcounts, I need to infer or say that the distribution is based on counting all visible blocks across both views, ensuring no double-counting. But the task is to summarize the trace, not solve the puzzle. The user's question is the puzzle, and the internal reasoning is the thinking. But the instruction is to summarize thethinking trace for the user query, but don't present it in the third person. So, as Grok, I should present the summary as my first person thoughts. Let me craft a natural response. I looked at the two images of the 3D object made of colored blocks, and I need to figure out howmany blocks of each color there are in total. The object seems to be a connected structure of cubes, and I have to account for all the blocks visible in either view, since together they show all surfaces. The possible colors are yellow, cyan, green, magenta, red, orange, orchid, teal, slategray, gold, blue, purple. From the views, I see mostly yellow, cyan, magenta, red, green, teal, slategray. I counted the blocks in each color by looking at both images and adding up the visible ones, making sure not to count any block twice if it's visible in both, but sincethey are from different angles, each block is unique. I reconstructed the 3D layout mentally, imagining the grid positions, and counted each position's color. 
For example, the center has a few greens and cyans, the protruding parts have teals and slategrays, the tall stack has magentas and reds, and scattered yellows and oranges. }{Harnessing} \newline
The final count is something like:

\tann{annCol10}{orchid: 1, orange: 2, purple: 1, red: 5, yellow: 10, cyan: 8, green: 3, magenta: 4, teal: 2, slategray:4, gold: 1, blue: 1 }{Wrong Perception} \newline
But that's a guess.

The trace is incomplete and approximate, with attempts to count per view.

\tann{annCol10}{In view 1, approximate counts: yellow 4, cyan 2, magenta 3, red 2, green 1, gray 3,teal 2 In view 2, magenta 3, red 2, yellow 3, cyan 4, green 1, gray 3, teal 2 }{Wrong Perception} \newline
Adding them up without double-counting since views are different angles but same blocks.

But since it's the same object, I need to counteach block once, but the trace doesn't distinguish hidden blocks.

\tann{annCol5}{The trace concludes that all visible colors are included, and the distribution is the union of colors from both views. The answer format is a dict of color to count. Since the trace is truncated and incomplete, the response should acknowledge that and provide a plausible distribution basedon mentioned colors.}{Harnessing}

\tann{annCol10}{I observe the mentioned colors are: orchid, orange, purple, red, yellow, cyan, and others like teal, slategray.}{Wrong Perception}

\tann{annCol7}{The example has orchid, orange, purple, red, yellow, cyan. So perhaps the distribution is as in the example, but adjusted.}{Prior Bias}

The example is \{"orchid": 10, "orange": 2, "purple": 1, "red": 5, "yellow": 2, "cyan": 8\}

But the trace mentions different colors.

The trace has teal, gray, cyan, yellow, green, magenta, red.

\tann{annCol10}{So the distribution is teal:1, slategray:3, green:1, magenta:4, red:2, yellow:4, cyan:2, summing to 17. }{Wrong Perception} \newline
That seems plausible.

The second view has more counts for some colors.

To make it coherent, I'll use that count.

The response should be in the format:

\{

'answer': \{"orchid": 10, "orange": 2, "purple": 1, "red": 5, "yellow": 2, "cyan": 8\},

\}

But that's the example, not the actual.

\tann{annCol5}{The task is to summarize the thinking trace, not tosolve the problem. The user query is to summarize the thinking trace, but the content is the problem description. \textit{[[...trimmed output...]]}
% The user says "Summarize the thinking trace for the user query", but the user query is the problem about the 3D object. It's a bit confusing. The human message is: Summarize the thinkingtrace for the user query, but don't present it in the third person as the trace of a separate entity. Then [User's Question] is the problem about the 3D object. Then [Internal Reasoning] is the partial reasoning about the object. So my job is to turn the internal reasoning into a clean,natural final response. But the instruction is to summarize the thinking trace for the user query. The final response should be the color distribution, I think, because the task is to give the color distribution, and the internal reasoning is to help me figure it out. The system prompt says "turn detailed internal reasoning into a clean, natural final response for the end user." And "Present the content as your first person thoughts instead of a third person entity's thoughts." "Speak directly as Grok answering the user's question." The user's question is the problem about the 3D object, and I need to answer with the output format. 
The internal reasoningis incomplete, but I need to complete it or use it to form the answer. }{Harnessing} \newline
The internal reasoning is truncated, but it starts counting for view 1 and view 2.

\tann{annCol10}{For view 1: - Slategray: 3 - Teal: 1 - Yellow: 4 - Cyan: For view 1: - Slategray: 3 - Teal: 1 - Yellow: 4 - Cyan:2 - Green: 1 - Magenta: 3 - Red: 2 Total 16 For view 2: The trace says magenta 4, red 2, yellow 3, cyan 4, green 1, slategray 3, teal 2 = 19, but notes overcount, so adjusts to total 20 with yellow 4, cyan 4, magenta 4, red 2, green 1, slategray 3, teal 2. Yes, that seems reasonable. The colors are magenta, red, yellow, cyan, green, slategray, teal. No orange, orchid, etc., probably not present. No gold, blue, purple, as they might be misidentified. So the distribution is magenta:4, red:2, yellow:4, cyan:4, green:1, slategray:3, teal:2. Total 4+2+4+4+1+3+2=20. }{Wrong Perception} \newline
That seems plausible for the object.

I think that's the answer.
\end{tcolorbox}
\begin{tcolorbox}[breakable,enhanced,colback=green!4,colframe=green!50!black,boxrule=0.4pt,arc=1pt,left=4pt,right=4pt,top=3pt,bottom=3pt,fonttitle=\footnotesize\bfseries,coltitle=black,colbacktitle=green!14,title={\tpicon{gpt_icon.png}~GPT-5\hfill answer: \tickok}]
\footnotesize\raggedright
Counting colors in voxel images \newline
I need to count the colors from two images of colored cubes on a grid. This might require manually analyzing the images, maybe enhancing them using edge detection or zooming in. Since these images are isometric voxel art, I'll focus on reconstructing the cube arrangement to count the blocks by color. \newline
Reconciling 3D block colors from images \newline
\tann{annCol9}{from PIL import Image import matplotlib.pyplot as plt img1=Image.open('/mnt/data/T5\_sample1\_row90\_query\_image\_1.png') img2=Image.open('/mnt/data/T5\_sample1\_row90\_query\_image\_2.png') img1.size, img2.size ((409, 409), (409, 409))}{Tool Use} \newline
Inspecting and counting colored blocks in images \newline
Output image \newline
Analyzing cube visibility and counting colors \newline
\textit{[[...trimmed output...]]} \newline
% I need to count all the cubes in this polycube object, which appears to be composed of unit cubes with colors. The object might be generated randomly with colored cubes based on coordinates. I'll infer the structure from two rotated views. I'll analyze visible faces for color counts and consider possible occlusion from hidden blocks. \newline
% Modeling cube coordinates and counting colors \newline
% In Image 1, I see a green cube on the left, magenta in the center, and a protruding magenta column with red on the right. Image 2 gives a clearer view, showing rows of red, magenta, slategray with some yellow, cyan, and teal. I'll map these cubes into 3D coordinates for easier counting and identification. \newline
Analyzing the object arrangement \newline
In Image 2, the object seems to have a front face with three columns and at least two rows. \tann{annCol10}{The colors from top to bottom are: red, magenta, slategray, yellow, green, teal, and cyan. }{Wrong Perception}It looks like there's a stack arrangement, though I'll need to avoid confusing the columns and rows. I'll focus on the edges for clarity. \newline
Analyzed image \newline
Output image \newline
Extracting cubes using image coordinates \newline
I could try using image coordinates to extract the cubes, as the unit cubes are projected to parallelograms in a single render. If I can detect visible faces, I might infer positions, though I need to avoid overcounting or missing any cubes. I'll inspect the images more closely, adjust with coordinate axes, and sample unique color segments. \newline
Extracting visible faces and color segments \newline
\tann{annCol9}{import numpy as np, pandas as pd import PIL.Image as Image for i,img in enumerate([img1,img2],1): arr=np.array(img.convert('RGB')) \# count most common colors excluding white/black and anti alias maybe threshold by exact likely colors colors, counts=np.unique(arr.reshape(-1,3), axis=0, return\_counts=True) idx=np.argsort(counts)[::-1][:20] print('img',i) for c,n in zip(colors[idx], counts[idx]): print(tuple(c), n) print() img 1 (np.uint8(255), np.uint8(255), np.uint8(255)) \textit{[[...trimmed output...]]}
% 109156 (np.uint8(255), np.uint8(0), np.uint8(255)) 11045 (np.uint8(112), np.uint8(128), np.uint8(144)) 9024 (np.uint8(255), np.uint8(255), np.uint8(0)) 7977 (np.uint8(0), np.uint8(128), np.uint8(128)) 6030 (np.uint8(0), np.uint8(0), np.uint8(0)) 5817 (np.uint8(0), np.uint8(255), np.uint8(255)) 5410 (np.uint8(255), np.uint8(0), np.uint8(0)) 4231 (np.uint8(0), np.uint8(128), np.uint8(0)) 2222 (np.uint8(255), np.uint8(215), np.uint8(0)) 337 (np.uint8(158), np.uint8(158), np.uint8(158)) 96 (np.uint8(110), np.uint8(0), np.uint8(0)) 86 (np.uint8(0), np.uint8(6), np.uint8(6)) 58 (np.uint8(0), np.uint8(78), np.uint8(78)) 55 (np.uint8(205), np.uint8(205), np.uint8(205)) 54 (np.uint8(235), np.uint8(0), np.uint8(235)) 54 (np.uint8(216), np.uint8(216), np.uint8(0)) 54 (np.uint8(33), np.uint8(38), np.uint8(43)) 53 (np.uint8(3), np.uint8(0), np.uint8(3)) 53 (np.uint8(54), np.uint8(0), np.uint8(54)) 53 img 2 (np.uint8(255), np.uint8(255), np.uint8(255)) 105120 (np.uint8(0), np.uint8(255), np.uint8(255)) 11331 (np.uint8(0), np.uint8(128), np.uint8(128)) 9406 (np.uint8(255), np.uint8(0), np.uint8(255)) 8144 (np.uint8(255), np.uint8(255), np.uint8(0)) 8104 (np.uint8(0), np.uint8(0), np.uint8(0)) 5918 (np.uint8(112), np.uint8(128), np.uint8(144)) 5790 (np.uint8(255), np.uint8(0), np.uint8(0)) 5670 (np.uint8(0), np.uint8(128), np.uint8(0)) 894 (np.uint8(255), np.uint8(215), np.uint8(0)) 804 (np.uint8(55), np.uint8(55), np.uint8(55)) 103 (np.uint8(1), np.uint8(0), np.uint8(0)) 74 (np.uint8(0), np.uint8(1), np.uint8(1)) 70 (np.uint8(128), np.uint8(128), np.uint8(128)) 64 (np.uint8(0), np.uint8(27), np.uint8(27)) 63 (np.uint8(0), np.uint8(28), np.uint8(28)) 60 (np.uint8(0), np.uint8(99), np.uint8(99)) 60 (np.uint8(0), np.uint8(245), np.uint8(245)) 58 (np.uint8(67), np.uint8(0), np.uint8(67)) 56 (np.uint8(0), np.uint8(116), np.uint8(116)) 56 
}{Tool Use} \newline
Identifying the gold color and counting cubes \newline
\textit{[[...trimmed output...]]} \newline
% I'm noticing possible gold patches with the exact RGB of 255,215,0, which might be actual gold blocks or simply shading. In Image 1, the gold color appears as vertical rectangles, while in Image 2, there are small yellow-orange faces under cyan. I'll need to inspect and count the actual gold cubes more carefully, differentiating between shading and color. \newline
% Counting cubes and analyzing connected colors \newline
% I need to count the cubes themselves based on their actual color and not just the visible area. The solid fill color for each face is what matters here, even with the black outlines. I'll segment the colors and analyze the connected components for each color. It's important to consider the separation created by the black outlines, which means faces on adjacent cubes might appear connected but are technically separated. \newline
Counting distinct color components in rendered images \newline
\tann{annCol9}{from scipy import ndimage import numpy as np, matplotlib.pyplot as plt color\_map=\{ 'yellow':(255,255,0),'cyan':(0,255,255),'green':(0,128,0),'magenta':(255,0,255),'red':(255,0,0), 'teal':(0,128,128),'slategray':(112,128,144),'gold':(255,215,0) \} for name,c in color\_map.items(): for idx,img in enumerate([img1,img2],1): arr=np.array(img.convert('RGB')) mask=np.all(arr==c,axis=2) lab,n=ndimage.label(mask) comps=[] for j in range(1,n+1): ys,xs=np.where(lab==j) if len(xs)>20: comps.append((len(xs),(xs.min(),ys.min(),xs.max(),ys.max()))) comps=sorted(comps, reverse=True) if comps: print('img',idx,name,'components',len(comps),comps[:10]) print() img 1 yellow components 3 [(2771, (np.int64(202), np.int64(165), np.int64(264), np.int64(218))), \textit{[[...trimmed output...]]}
% (2603, (np.int64(212), np.int64(78), np.int64(284), np.int64(123))), (2603, (np.int64(202), np.int64(122), np.int64(274), np.int64(167)))] img 2 yellow components 4 [(3330, (np.int64(124), np.int64(216), np.int64(187), np.int64(273))), (2266, (np.int64(135), np.int64(139), np.int64(206), np.int64(178))), (2266, (np.int64(125), np.int64(178), np.int64(196), np.int64(217))), (242, (np.int64(192), np.int64(198), np.int64(197), np.int64(256)))] img 1 cyan components 3 [(2601, (np.int64(280), np.int64(85), np.int64(351), np.int64(130))), (2600, (np.int64(135), np.int64(115), np.int64(206), np.int64(160))), (209, (np.int64(347), np.int64(108), np.int64(352), np.int64(164)))] img 2 cyan components 5 [(3278, (np.int64(202), np.int64(183), np.int64(264), np.int64(240))), (3278, (np.int64(57), np.int64(211), np.int64(119), np.int64(267))), (2267, (np.int64(57), np.int64(172), np.int64(129), np.int64(211))), (2266, (np.int64(202), np.int64(145), np.int64(274), np.int64(184))), (242, (np.int64(269), np.int64(167), np.int64(274), np.int64(225)))] img 1 green components 1 [(2222, (np.int64(202), np.int64(217), np.int64(252), np.int64(269)))] img 2 green components 1 [(894, (np.int64(134), np.int64(253), np.int64(197), np.int64(290)))] img 1 magenta components 6 [(3090, (np.int64(249), np.int64(259), np.int64(312), np.int64(313))), (2603, (np.int64(250), np.int64(216), np.int64(321), np.int64(261))), (2601, (np.int64(270), np.int64(128), np.int64(341), np.int64(173))), (2297, (np.int64(202), np.int64(270), np.int64(264), np.int64(323))), (244, (np.int64(316), np.int64(238), np.int64(322), np.int64(298))), (210, (np.int64(337), np.int64(151), np.int64(342), np.int64(207)))] img 2 magenta components 4 [(3330, (np.int64(134), np.int64(289), np.int64(197), np.int64(346))), (2267, (np.int64(88), np.int64(56), np.int64(159), np.int64(95))), (2267, (np.int64(68), np.int64(133), np.int64(139), np.int64(173))), (280, (np.int64(154), np.int64(76), np.int64(160), np.int64(135)))] img 1 red components 4 [(2599, (np.int64(260), np.int64(172), np.int64(331), np.int64(217))), (1178, (np.int64(269), np.int64(281), np.int64(332), np.int64(329))), (245, (np.int64(326), np.int64(195), np.int64(332), np.int64(255))), (209, (np.int64(337), np.int64(256), np.int64(342), np.int64(311)))] img 2 red components 3 [(3330, (np.int64(67), np.int64(283), np.int64(130), np.int64(340))), (2268, (np.int64(78), np.int64(95), np.int64(149), np.int64(134))), (72, (np.int64(145), np.int64(114), np.int64(150), np.int64(135)))] img 1 teal components 3 [(3089, (np.int64(56), np.int64(196), np.int64(119), np.int64(249))), (2604, (np.int64(57), np.int64(152), np.int64(129), np.int64(197))), (334, (np.int64(134), np.int64(234), np.int64(197), np.int64(264)))] img 2 teal components 5 [(3330, (np.int64(279), np.int64(151), np.int64(342), np.int64(207))), (3278, (np.int64(202), np.int64(239), np.int64(264), np.int64(296))), (2267, (np.int64(280), np.int64(112), np.int64(351), np.int64(151))), (282, (np.int64(346), np.int64(132), np.int64(352), np.int64(194))), (243, (np.int64(269), np.int64(222), np.int64(274), np.int64(281)))] img 1 slategray components 4 [(3089, (np.int64(134), np.int64(263), np.int64(197), np.int64(316))), (3089, (np.int64(124), np.int64(203), np.int64(187), np.int64(256))), (2602, (np.int64(125), np.int64(159), np.int64(196), np.int64(204))), (244, (np.int64(191), np.int64(182), np.int64(197), np.int64(241)))] img 2 slategray components 3 [(3278, (np.int64(202), np.int64(295), np.int64(264), np.int64(351))), (2269, (np.int64(212), np.int64(106), np.int64(284), np.int64(145))), (243, (np.int64(269), np.int64(278), np.int64(274), np.int64(337)))] img 1 gold components 2 [(208, (np.int64(337), np.int64(204), np.int64(342), np.int64(259))), (129, (np.int64(325), np.int64(247), np.int64(332), np.int64(277)))] img 2 gold components 1 [(804, (np.int64(67), np.int64(267), np.int64(130), np.int64(284)))] 
}{Tool Use} \newline
Counting cubes and annotating colors from images \newline
I need to focus on counting cubes, not their faces. It's possible the images are rendered as axonometric projections from a voxel grid, which could help derive 3D positions from the polygons. I'll annotate the exact colors by analyzing the components in image 2. For example, the yellow stack likely represents two cubes, while the cyan components suggest three cubes. I'll map these out carefully. \newline
Analyzing additional colors and cube counts \newline
The components from image 2 show more possibilities: \newline
\tann{annCol10}{Teal components suggest 3 cubes.}{Wrong Perception} \newline
Slate gray components may correspond to 2 cubes. \newline
\textit{[[...trimmed output...]]} \newline
% Magenta: 3 or more cubes seem likely from their positioning (front, stack top/mid). \newline
% Red: Considered as potentially 2 cubes, stacked with small sides. \newline
% Green: Likely 1 hidden cube between yellow, teal, and magenta. \newline
% Identifying projections and grid directions \newline
% I'm analyzing the projection in isometric images. In image 2, the front face of cubes appears as a parallelogram, with dimensions around 63x54 for width and height, and vertical slants. For adjacent cubes, I calculated horizontal and vertical shifts between faces. The red and yellow faces help define these shifts, giving vectors for ``x'' and ``z''. \newline
% Examining projection axes and depth shifts \newline
% I'm analyzing how the projection works. In image 2, the row above shifts because of depth---it's not directly above but may go deeper or left. I think the projection follows specific directions: horizontal, depth, and vertical, with vectors that will help calibrate the cube positions. The black lines seem to indicate orthographic projections. \newline
% Reconstructing layout and counting visible cubes \newline
% I think it might be easier to use both views to identify visible top, front, and side faces. Each cube should be visible in at least one view. By looking at these, I can match duplicates and count cubes by their main visible faces, mapping colors to blocks. I'll start by labeling blocks from Image2. \newline
% Clarifying cube structure and positioning \newline
% I think the cyan on the left and yellow in the middle are part of the same cubes, connected by black outlines. Similarly, the cyan on the right and yellow middle share top and front faces. Now, in the vertical column, there are three cubes: a magenta at the top, red just below, and another magenta. I'll continue checking their positions and structure. \newline
% Reassessing left-back and top-right cubes \newline
% I now think the left/back column has a cyan cube at the bottom, followed by magenta, red, and magenta cubes. The magenta count increases by 2, and red by 1. For the top-right protruding arm \newline
% Considering occlusion and visibility in 3D projection \newline
% Okay, this explains that a hidden cube behind the front row could have just its top/front edge visible, and perhaps a yellow or gold cube is behind the red and below cyan. From the images, I see vertical gold slivers that might be occluded blocks---likely side/back. Can infer exact counts from visible areas by using pixel data! \newline
% Reconstructing cube positions through visibility and projection \newline
% Since hidden cubes may show only small visible areas, I think I can approximate the count by mapping visible faces to cubes. If at least one cube face is visible in either view, I can infer its presence, even if partially occluded. It seems like using ray tracing might help reconstruct cube positions based on face alignment. \newline
% Clarifying component shapes on image \newline
% Each colored polygon has black outlines, which help align component bounding boxes to specific cube face types. For instance, I noticed the magenta top face of the column has a bounding box of 72x39, while the red component is not the top face but actually a slanted side face in a vertical stack. \newline
% Analyzing cube projections and perspectives \newline
% In image2, the left stack of cubes is arranged vertically (along the z-axis). We're seeing side faces of the cubes rather than top surfaces. The perspective distortion leads to slanted parallelograms for the visible top, left, and right faces. The bounding boxes reflect different heights due to this perspective. One cube showing top and front faces demonstrates this: the top face appears as a parallelogram with dimensions 39x39, while the front displays a height of 56. \newline
% Reassessing cube arrangement and perspective \newline
% The cubes' top faces, when projected, appear as parallelograms rather than having vertical height. Upon closer inspection, the sequence of magenta, red, magenta, and cyan cubes seems to form a row along the top surface, not a vertical stack. This row recedes in depth, with each top face aligned and appearing as parallelograms at the same height. This explains the consistent bounding box dimensions (72x39). \newline
% Mapping voxel stack and interpreting projections \newline
% Each view can be seen as a projection of a voxel stack, showing the top and side faces of the cubes. The top faces are the most reliable for counting since every top-exposed cube will show a visible face from above. We need to track the height of the stack and define a coordinate system for better interpretation. From image2, the bounding boxes for the top faces suggest a grid with shifts in the x direction. \newline
% Reevaluating cube stack and visible faces \newline
% I initially thought the top-left diagonal represented stacked cubes with visible top faces. But as I analyze it, the shifted positions suggest these are actually side faces of a stacked column, not top faces. If the cubes were stacked, only the top cube's top face should be visible. It seems the magenta component is more likely to be a front or side face instead. \newline
% Revising cube face projection and positioning \newline
% In isometric projection, the vertical axis shifts by (10, -39), which affects the positioning of a cube's top. The left column might show side faces of 4 stacked cubes. The topmost cube's top face seems to fit a bbox (88,56)-(159,95), though this could be a side face with a small visible top sliver as well. \newline
% Reassessing vertical stack and colors \newline
% The left front column seems to have a stack of around 3 cubes: bottom red (y283-340), then a gold cube (above y267-284), followed by a cyan one. Above that, a second cyan cube. Meanwhile, the left top column seems to share the same ground position but with different colors stacking in a different order. There's a slight gap between the top cyan and magenta rows. \newline
% Analyzing the stack's components and their positions \newline
% There seems to be a gap between y173 \newline
% Analyzing inconsistencies in the model \newline
% It seems the vertical shifts for the stack aren't consistent. For example, the shift from red to gold doesn't match the expected shift, and the red to cyan shift is too large. This might be due to perspective differences in the views. To clarify, I'll try using a method to detect the cubic components by analyzing both views and grouping adjacent faces of the same color. This should help infer which faces correspond to the same block. \newline
% Evaluating yellow components and stack possibilities \newline
% It seems like we have two yellow cubes stacked rather than just one. Based on the faces and their placements, the top yellow component might be the top of the upper cube, while the bottom yellow shows the front face of the lower cube. So, it's likely two cubes stacked vertically, similar to other vertical sequences. This accounts for their visibility and positioning. \newline
% Analyzing yellow cube positioning and component dimensions \newline
% The shapes seem to align with the idea of two yellow cubes stacked rather than just one \newline
% Deciphering yellow cube stack and visible faces \newline
% It seems like there are likely two yellow cubes stacked. The lower yellow component represents the front face of the bottom cube, while the upper cube shows its side/front faces. Component J could be the top face of the upper cube. The middle component might represent the side/front of the upper cube, as seen from this perspective. \newline
% Analyzing stack arrangement across views \newline
% In View2, I see an L-shaped group of vertical stacks. The left stack seems to have red, gold, cyan, magenta cubes, stacked in varying positions. The middle stack has magenta, green, and yellow cubes, possibly more yellow. On the right stack, I identify slategray, teal, and cyan. I'll compare this with View1 to validate further. The left/front side shows teal and slategray with specific orientations. \newline
Estimating cube counts from views \newline
\tann{annCol10}{It seems there are around 19 cubes based on color estimates}{Wrong Perception}: cyan (2), yellow (2), green (1), \tann{annCol10}{magenta (4), red (3), teal (3), slategray (3),}{Wrong Perception} and gold (1 or 2). I'll now attempt to create a 3D coordinate model to confirm these counts and see if it matches the visual appearance of the object. \newline
Defining stack grid and views \newline
\textit{[[...trimmed output...]]} \newline
% I'm figuring out how to map \newline
% Examining grid of stacks and matching views \newline
% I'm considering a 3x3 grid: one column with red, gold, cyan, magenta, red, magenta (6 cubes). Another with magenta, green, yellow, yellow (4 cubes). And the last column with slategray, teal, cyan, slategray (4 cubes) plus an adjacent teal. This adds to 15 cubes. But image1 shows more red, magenta, teal, and slategray. Let me check how the orientations in image1 compare. The bottom row seems to match across both views. \newline
% Clarifying magenta cube placement and count \newline
% I'm confirming that the view1 shows two yellow cubes (top/middle). For green, there's just one in the center. The magenta cubes might total 3 instead of 4. The bottom center, left stack, and top stack all each have magenta components, including the front-right projection. Looks like three magenta cubes in total. Red count appears to be two: one in the lower stack and one in the top stack. \newline
Confirming total block count and stack alignment \newline
\tann{annCol3}{The predicted color counts are: red (2), gold (1), cyan (2), magenta (3), green (1), yellow (2), slategray (2), teal (2), making it a total of 15 blocks.}{Good Perception} After examining image2 and image1, the total seems to range from 14 to 15 cubes. I verified that stacks match up: \tann{annCol10}{the left column has 6 blocks, middle 4, right 4,}{Wrong Perception} and the extra teal block adds 1, confirming a total of 15. \newline
Examining column alignment and image consistency \newline
Looking at the bottom stack, the sequence of colors---magenta, red, magenta, cyan, gold, red---doesn't perfectly match image1. The cyan at the top-right may overlap with the right column cyan. Examining image1 components visually reveals that the topmost yellow fits the middle stack, and cyan corresponds to the right stack's top. The arrangement aligns with multiple layers of columns: left, middle, and right.

``` \newline
\{ \newline
'answer': \{"red": 2, "gold": 1, "cyan": 2, "magenta": 3, "green": 1, "yellow": 2, "slategray": 2, "teal": 2\}, \newline
\} \newline
```
\end{tcolorbox}
\begin{tcolorbox}[breakable,enhanced,colback=red!4,colframe=red!55!black,boxrule=0.4pt,arc=1pt,left=4pt,right=4pt,top=3pt,bottom=3pt,fonttitle=\footnotesize\bfseries,coltitle=black,colbacktitle=red!12,title={\tpicon{gemini_flash_icon.png}~Gemini-3-Flash\hfill answer: \tickno}]
\footnotesize\raggedright
```json \newline
\{ \newline
"answer": \{ \newline
"teal": 2, \newline
\tann{annCol10}{"slategray": 3, "cyan": 4, "yellow": 3, "magenta": 4,}{Wrong Perception} \newline
"red": 2, \newline
"green": 1, \newline
"gold": 1 \newline
\} \newline
\}

```
\end{tcolorbox}
\begin{tcolorbox}[breakable,enhanced,colback=red!4,colframe=red!55!black,boxrule=0.4pt,arc=1pt,left=4pt,right=4pt,top=3pt,bottom=3pt,fonttitle=\footnotesize\bfseries,coltitle=black,colbacktitle=red!12,title={\tpicon{gemini_pro_icon.png}~Gemini-3.1-Pro\hfill answer: \tickno}]
\footnotesize\raggedright
Analyzing Images

I've begun to discern the visible colors in the initial image, noting teal, slategray, cyan, and yellow blocks.

Revising Image Views

I've determined Image 2 shows the back of the object, which clarifies the Teal block's orientation in 3D space.

\textit{[[...trimmed output...]]}

% Mapping Block Locations

% I've begun mapping block placements using a grid, noting their front views and projecting positions, using Image 1's perspective.

% Clarifying Block Order

% I've resolved the column order, identifying Cyan(z=3), Slategray(z=2), Slategray(z=1) within the main body.

% Tracing Grid Points

% I'm now tracing the grid positions, noting color order across columns and clarifying the number of total columns.

% Defining Block Coordinates

% I've specified each column's structure, clarified the location and color of all blocks, and resolved initial z-axis discrepancies.

% Pinpointing Block Details

% I've clarified the right-side column's structure as Cyan(z=3), Magenta(z=2) with an added forward block, and Red(z=1).

% Clarifying Block Structure

% I've determined that a Magenta block protrudes forward from the right column, confirming its full visibility.

% Reassessing Object Faces

% I've determined block colors on the main column's right face using both images, resolving Image 2's mirrored perspective.

% Reconciling Perspectives

% I'm now identifying discrepancies between Image 1 and Image 2 regarding the Teal arm's column color order, specifically Cyan versus Slategray.

Clarifying Face Details

\tann{annCol10}{I've traced the face details, confirming column colors in Image 2: Magenta, Yellow, Cyan, and Slategray blocks.}{Wrong Perception}

\tann{annCol8}{Defining Coordinates I'm establishing a coordinate system, fixing Yellow as (0,0) and mapping its column as [z=1: Green/Magenta, z=2: Yellow, z=3: Yellow]. Resolving Depth Conflicts I've determined that Green and Magenta at (0,0) indicate multiple blocks, thus depth > 1, requiring a re-evaluation. Refining Column Details I have clarified the middle column, considering block visibility and using image perspectives to refine color placements. Verifying Visual Data I have confirmed that the front view in Image 1 aligns, noting green at z=1, then Yellow at z=2 and z=3, aligning to the previous logic. Determining Face Views I'm now clarifying the image's perspective, focusing on visible faces of Teal and Cyan blocks to understand the overall shape. Mapping Face Directions I'm now mapping face directions from Image 1, defining blocks based on their visible faces across all views.}{Reiterating}

Analyzing Column Data \newline
\tann{annCol10}{ I have discovered a column discrepancy, counting 5 columns in Image 2, contradicting previous counts and resolving an issue.}{Wrong Perception}

Counting Total Columns

\tann{annCol10}{I've counted a total of 5 columns based on Image 2's back view, further clarifying block positioning.}{Wrong Perception}

\tann{annCol8}{
Confirming Color Alignment I'm now cross-referencing Images 1 and 2, resolving the Teal block's location and verifying Cyan column consistency. Defining Block Structure I've determined the Teal block's connection to a Slategray block, clarifying the block's position and resolving x=0, z=3 with Cyan. \textit{[[...trimmed output...]]}
% Verifying Face Colors I've determined that the structure is likely rotated 90 degrees, accounting for the arm's orientation shift in Image 2. Verifying Rotations I've confirmed the 180-degree rotation, identifying Image 2 as the back view and verifying Cyan/Slate color alignments. Clarifying Face Placement I've determined that Yellow is column 1, and now confirming block positions via Image 1 and 2 cross-referencing. Revising Block Depths I'm revisiting the depths, reconciling Green and Magenta color conflicts with Image 1's perspective and block visibility. Resolving Depths Conflicts I've determined Magenta and Green share y=0, but their z-axes distinguish these potentially overlapping blocks. Verifying Column Depth I've determined Yellow (y=1) covers Magenta, confirming block visibility and resolving previously noted discrepancies. Confirming Green Visibility I've verified Green's top face, confirming its forward protrusion from the Yellow block, and the left face's visibility. Examining Column Data I am now focusing on column 2's structure, identifying Cyan (z=3), and below Magenta (z=2). Refining Column Data I'm now identifying that the Cyan(y=1, z=2) block's corresponding Red (y=0, z=1) from Image 1 confirms depth overlap. Tracing Block Color I have located Red's correct position at the base of the left column, confirming its presence at y=0, z=1. Locating Block Faces I'm now identifying that Red's forward block face clarifies the column's structure and position in Image 1. Identifying Block Order I've determined there is a Red block adjacent to, or potentially behind, an Orange block on the right face. Clarifying Right Faces I'm now identifying that Red (y=0,z=1) and Orange (y=1,z=1) are separate blocks, visible in Image 1. Locating New Blocks I've located a Gold/Orange block at x=2, y=0, z=1 in Image 2, situated beneath the Cyan block, finally clarifying the block. Tracing Block Order I've clarified the presence of Red (z=2) below Magenta (z=3), and now located an Orange block in Image 2. Locating Block Coordinates I'm now clarifying block positions to refine column composition using image alignment to verify locations. Defining Image Orientations I'm now determining if Image 2 is back-left or back-right to align the Teal block's positioning within its view. Defining Image Orientations I've determined Image 2 is back-left, with x=2 visible on the left side, thereby accurately locating all block coordinates. Defining Image Directions I've determined both images employ isometric projection with Image 1 at Front-Top-Right and Image 2 at Back-Top view. Defining Column Mapping I've clarified the x-axis, using Image 2, and confirmed all block coordinates across images. Verifying Face Depths I've determined y=1 obscures y=0 in the direct back view, resolving the Magenta top face ambiguity in Image 2. Revising Block Placement I've determined Magenta (z=3) in Image 2 is likely at x=2, y=2, considering column structure and resolved conflicts. Revising Block Faces I've determined Magenta (z=2) and Cyan (z=3) heights in Image 1 align, implying potential column shifts. Verifying Height Alignment I've confirmed Magenta and Cyan are the same height, resolving previous misinterpretations in the image perspective. Analyzing Block Layers I've determined that Cyan covers Magenta from the back-left view, visualizing y-depth correctly to trace block visibility. Clarifying Face Visibility I'm now clarifying block visibility to determine if Magenta is indeed behind Cyan from the left perspective. Mapping Block Placement I've determined Magenta's x-coordinate is 3 using image analysis, verifying its correct placement in the composite structure. Revising Block Structure I've determined Magenta is below Cyan in the primary structure, resolving initial directional interpretations from Image 1's view. Counting Block Colors I've counted the blocks in both images, noting Teal, Slategray, Cyan, Yellow, Green, Magenta, Red, and Gold/Orange. Mapping Block Visibility I have determined the primary structure's column 0: Cyan(3), Slategray(2), Slategray(1) aligns with images. Refining Face Data I'm now refining faces based on height alignment, confirming Magenta is forward of Cyan, resolving initial errors. Locating Block Layers I've determined that under Magenta(3), based on image analysis, are Orange(1) and Red(2), adding more layers. Clarifying Layer Depths I've determined y=0, z=2 is indeed empty in Image 1 and contains a light blue face in Image 2. Revising Block Heights I've determined there are now two Red blocks in column 2, under Magenta, clarifying previous layer inconsistencies. Examining Image Content I am now verifying the Right face with Magenta, not Cyan, at y=0, with an implied forward Orange block. Verifying Face Views I'm now cross-referencing to confirm the right face of the y=1, z=2 column, and the related Gold/Orange visibility. Verifying Visual Data I have located the Red block on the bottom right and verified Gold (y=1,z=2) and Red (y=1,z=1) on the Right face. Finalizing Model Details I have completed the model with perfect consistency, verifying all block placements and confirming the final count. Confirming Block Count I've carefully recounted all blocks and confirmed the 14-block model with full color and coordinate accuracy. Counting Hidden Blocks I have located all 14 blocks, identifying Magenta and Green as the hidden ones in the images. Refining Block Colors I've specified the Gold/Orange block, confirming its color and position based on image analysis and color data. Finalizing Block Counts I've precisely verified hidden blocks, confirming the complete model accuracy and finalized block color definitions. Verifying Object Geometry I've perfectly verified object geometry and color order, confirming block positions based on image faces. Revising Block Counts I've confidently confirmed block counts: Teal(1), Cyan(2), Slategray(2), Yellow(2), Magenta(2), Green(1), Red(3), Gold(1). Clarifying Perspectives I've determined that camera positioning and ray divergence explain all block face visibility across the images. Analyzing Block Obscurity I've determined Magenta's ray passes to the right of Cyan, implying its visibility in the back view. Resolving Obscurity Issues I've fixed the camera perspective, proving Magenta overlaps Cyan, confirming the block's z-axis placement. Revising Block Placement I've determined the inconsistency stems from an image perspective error, revising initial coordinate placements accordingly. Verifying Placement Details I have confirmed Magenta's precise x and y coordinates, verifying its position within the composite model. Refining Block Structures I've clarified the x=2 column as Cyan(z=3) over Gold(z=2) and Red(z=1), with x=3: Magenta(z=3) over Red(z=2) and Red(z=1). 
Confirming Structure Integrity I've verified the model's structural integrity, confirming block counts and locations with both image views.}{Reiterating}

```json \newline
\{ \newline
"answer": \{"teal": 1, "cyan": 2, "slategray": 2, "yellow": 2, \tann{annCol10}{"magenta": 2,}{Wrong Perception} "green": 1, \tann{annCol10}{"red": 3,}{Wrong Perception} "gold": 1\} \newline
\}

```
\end{tcolorbox}

\subsubsection{T6 Local Structure}
\begin{table}[H]
\centering
\footnotesize
\setlength{\tabcolsep}{1pt}
\renewcommand{\arraystretch}{1.2}
\begin{tabular}{*{9}{>{\centering\arraybackslash}p{\dimexpr\textwidth/9-2\tabcolsep\relax}}}
\toprule
\multicolumn{9}{@{}l@{}}{\itshape ``\ldots{}Your task is to determine whether the object has at least one column (vertical stack of blocks) with a height greater than 3\ldots{}''}\\[0.3mm]
\multicolumn{9}{@{}c@{}}{\begin{tabular}{*{2}{c}}\includegraphics[width=0.450\textwidth,height=1.25in,keepaspectratio]{images/app_qual_traces/T6_sample1_row5_query_image_1.png} & \includegraphics[width=0.450\textwidth,height=1.25in,keepaspectratio]{images/app_qual_traces/T6_sample1_row5_query_image_2.png}\end{tabular}}\\[0.5mm]
\textbf{GT} & \tpicon{qwen_icon.png} & \tpicon{gemma_icon.png} & \tpicon{glmv_icon.png} & \tpicon{kimi_icon.png} & \tpicon{grok_icon.png} & \tpicon{gpt_icon.png} & \tpicon{gemini_flash_icon.png} & \tpicon{gemini_pro_icon.png}\\
True & True\tickok & False\tickno & False\tickno & True\tickok & True\tickok & True\tickok & False\tickno & False\tickno\\
\bottomrule
\end{tabular}
\caption{T6 Local Structure.}
\label{tab:qual_trace_t6}
\end{table}
\noindent\textbf{Thinking traces.}\par\smallskip
\begin{tcolorbox}[breakable,enhanced,colback=green!4,colframe=green!50!black,boxrule=0.4pt,arc=1pt,left=4pt,right=4pt,top=3pt,bottom=3pt,fonttitle=\footnotesize\bfseries,coltitle=black,colbacktitle=green!14,title={\tpicon{qwen_icon.png}~Qwen3.5-27B\hfill answer: True\tickok}]
\footnotesize\raggedright
The user wants me to determine if the 3D object has any column with a height greater than 3.

**Image 1 Analysis:** \newline
- This view shows a structure made of cubes. \newline
- Let's look at the "front-most" column. It seems to have a stack of blocks. \newline
- Looking at the bottom left part, there is a vertical stack. Let's count the visible blocks in that stack. \newline
- There is a top block, a middle block, and a bottom block. \tann{annCol8}{Wait, let's look closer.}{Reiterating} \newline
- In the first image, there is a column extending downwards. Let's trace it. \newline
- There's a block at the very bottom. Above it is another block. Above that is another block. \tann{annCol10}{That looks like a stack of 3 blocks.}{Wrong Perception} \newline
- Let's look at the other columns. \newline
- To the right of the bottom stack, there's a column that is 2 blocks high. \newline
- Behind that, there are single blocks. \newline
- \tann{annCol8}{Let's re-examine the first image carefully.}{Reiterating} \newline
- There is a central column. Let's call the grid coordinates (x, y). \newline
- Let's assume the "front" is towards the bottom left. \newline
- \tann{annCol10}{There is a column at the front-most position. It has a block on top, one below it, and one below that. That's a height of 3.}{Wrong Perception} \newline
- \tann{annCol8}{Wait, let's look at the second image to confirm heights.}{Reiterating}

\textit{[[...trimmed output...]]}

% **Image 2 Analysis:** \newline
% - This view is rotated. \newline
% - Let's look for the tall column. \newline
% - In the center-right area, there is a vertical stack. \newline
% - Let's count the blocks in that stack. \newline
- \tann{annCol10}{Top block. - Block below it. - Block below that. - Block below that.}{Wrong Perception} \newline
- \tann{annCol8}{Let's count carefully.}{Reiterating} \newline
\textit{[[...trimmed output...]]} \newline
% - From the top down: \newline
% 1. Top block. \newline
% 2. Second block down. \newline
% 3. Third block down. \newline
% 4. Fourth block down. \newline
- \tann{annCol8}{Wait, let's look at the structure again.}{Reiterating} \newline
\textit{[[...trimmed output...]]} \newline
% - In Image 2, there is a central vertical column. Let's count the visible faces. \newline
% - Top face of the highest block. \newline
% - Front face of that block. \newline
% - Below it, another block's front face. \newline
% - Below that, another block's front face. \newline
% - Below that, another block's front face. \newline
% - Let's trace the vertical line. \newline
% - Top block: visible top, front, right faces. \newline
% - Below it: visible front, right faces. \newline
% - Below that: visible front, right faces. \newline
% - Below that: visible front, right faces. \newline
- \tann{annCol3}{This looks like a stack of 4 blocks.}{Good Perception} Let's verify. \newline
- Let's look at the "T" shape on top. \newline
- In Image 2, there is a horizontal bar of blocks. \newline
- Let's try to map the blocks. \newline
- Let's assume a grid. \newline
- Let's look at the column that is sticking down the most. \newline
- \tann{annCol10}{In Image 1, the column at the "front" (bottom left) has 3 blocks visible vertically. Top, middle, bottom.}{Wrong Perception} \newline
- In Image 2, the corresponding column seems to be the one in the middle. \newline
- \tann{annCol8}{Let's look at the column in the middle of Image 2.}{Reiterating} \newline
\textit{[[...trimmed output...]]} \newline
% - It has a top block. \newline
% - Below it, a block. \newline
% - Below that, a block. \newline
% - Below that, a block. \newline
- \tann{annCol8}{Let's count again.}{Reiterating} \newline
\textit{[[...trimmed output...]]} \newline
% - Top block (part of the cross shape). \newline
% - Below it, a block. \newline
% - Below that, a block. \newline
% - Below that, a block. \newline
- \tann{annCol8}{Wait, let's look at the junction.}{Reiterating} \newline
\textit{[[...trimmed output...]]} \newline
% - In Image 2, there is a central column. \newline
% - Top block: part of the horizontal cross. \newline
% - Below it: a block. \newline
% - Below that: a block. \newline
% - Below that: a block. \newline
- \tann{annCol8}{Let's count the vertical segments.}{Reiterating} \newline
\textit{[[...trimmed output...]]} \newline
% - From the top of the central column down to the bottom. \newline
% - 1 (top block), 2, 3, 4. \newline
% - Let's look at the side view (Image 1). \newline
% - The column on the left (which corresponds to the central column in Image 2?) \newline
- \tann{annCol10}{In Image 1, there is a column at the front left. It has 3 blocks.}{Wrong Perception} \newline
- Wait, let's look at the right side of Image 1. There is a column of height 2. \newline
- Let's look at the back. \newline
- Let's try to reconstruct the object. \newline
- It looks like a "plus" sign or "T" shape on top of a pillar. \newline
- \tann{annCol10}{Let's look at Image 2 again.}{Wrong Perception} \newline
- There is a central vertical pillar. \newline
- \tann{annCol10}{Let's count the}{Wrong Perception}\tann{annCol0}{I have to give the solution based on the reasoning directly now.}{Budget Hit}
\end{tcolorbox}
\begin{tcolorbox}[breakable,enhanced,colback=green!4,colframe=green!50!black,boxrule=0.4pt,arc=1pt,left=4pt,right=4pt,top=3pt,bottom=3pt,fonttitle=\footnotesize\bfseries,coltitle=black,colbacktitle=green!14,title={\tpicon{grok_icon.png}~Grok-4.20\hfill answer: True\tickok}]
\footnotesize\raggedright
The problem asks if the object has at least one column with a height greater than 3. I need to output a JSON with 'answer' as True or False. \newline
I need to figure out if there's a column taller than 3 blocks in this voxel object, based on the two perspective views. The object is made of unit cubes, and I have to reconstruct the 3D structure mentally from the images to check for any vertical stack exceeding 3 cubes.

First, I tryto map out the positions of the blocks in both views. The views are isometric, showing the object from different angles, and I need to ensure consistency between them. For example, blocks in the same column should align in both images at matching positions.

\tann{annCol10}{In the first view, it looks like there's a base with stacks of2 or 3 high, like an L-shape or T-shape with heights mostly 2 or 3. The lower part has a tower of about 3 cubes, but nothing taller.}{Wrong Perception}

\tann{annCol3}{Switching to the second view, which seems clearer, I notice a potential taller stack on the lower right. Counting vertically:from the bottom, there's a single cube, then one above it, then another, making 3, and then possibly a fourth at a higher level connected to the crossbar.}{Good Perception}

\tann{annCol3}{Upon closer inspection, the central column in the second image appears to have cubes at four distinct levels, indicating a height of 4. }{Good Perception} \newline
Sincethe views are of the same object, and this column is visible in both (perhaps obscured in one but implied), there is indeed a column taller than 3.

Therefore, the answer is yes, there is at least one such column.
\end{tcolorbox}
\begin{tcolorbox}[breakable,enhanced,colback=green!4,colframe=green!50!black,boxrule=0.4pt,arc=1pt,left=4pt,right=4pt,top=3pt,bottom=3pt,fonttitle=\footnotesize\bfseries,coltitle=black,colbacktitle=green!14,title={\tpicon{gpt_icon.png}~GPT-5\hfill answer: True\tickok}]
\footnotesize\raggedright
Analyzing images for column height comparison \newline
I need to determine if any column height exceeds 3, so I'll analyze two views of a block object. \tann{annCol2}{From View1, it looks like there's possibly a column with height 3, while View2 provides a clearer perspective with a column appearing to have 3 blocks.}{Good Intuition} Let's count and finalize the output. \newline
Reconstructing object column heights from View2 \newline
In View2, I see a vertical column formed by cubes, with the leg at the front-right possibly having 3 cubes tall. The central vertical column also appears to have a top cube and two under it. There are visible cubes stacked along the front-right. I'll count up the vertical segments to decide if the height exceeds 3. \newline
Verifying column height from View2 \newline
\tann{annCol3}{It looks like there might be a stack of 4 cubes in the second view,}{Good Perception} which could suggest the column's height exceeds 3. I'll double-check by visually inspecting the images, possibly zooming in to get a clearer view. Edge detection might help, but for now, I think the visuals should be enough. \newline
Analyzed image \newline
Output image \newline
Analyzed image \newline
Output image \newline
Reconstructing column heights from View2 \newline
I need to focus on the vertical column in View2, which could have a height greater than 3 if it shows four cubes stacked. From the image, I can see the bottom leg with distinct horizontal lines marking cube layers. I'll ensure the cubes align correctly vertically to confirm the total height.

```python \newline
\{ \newline
'answer': True, \newline
\} \newline
```
\end{tcolorbox}
\begin{tcolorbox}[breakable,enhanced,colback=red!4,colframe=red!55!black,boxrule=0.4pt,arc=1pt,left=4pt,right=4pt,top=3pt,bottom=3pt,fonttitle=\footnotesize\bfseries,coltitle=black,colbacktitle=red!12,title={\tpicon{gemini_flash_icon.png}~Gemini-3-Flash\hfill answer: False\tickno}]
\footnotesize\raggedright
To determine if the object contains a vertical column with a height greater than 3, let's analyze the structural layers of the 3D block arrangement from both viewpoints:

1. **Horizontal Flat Layer:** Both perspectives show a predominant, sprawling horizontal plane or "shelf" that is 1 block thick. This forms the primary surface of the object. \newline
2. **Vertical Columns:** * Hanging down from or stacked beneath this main horizontal section, we can observe columns extending downwards. \newline
\tann{annCol10}{* Looking closely at the lowest protruding vertical structures in both views, the maximum vertical height of any single continuous stack (column) is exactly **3 blocks**. * No single vertical stack contains 4 or more blocks stacked directly on top of each other.}{Wrong Perception}

Therefore, the object does not have any column with a height greater than 3.

```json \newline
\{ \newline
"answer": false \newline
\}

```
\end{tcolorbox}
\begin{tcolorbox}[breakable,enhanced,colback=red!4,colframe=red!55!black,boxrule=0.4pt,arc=1pt,left=4pt,right=4pt,top=3pt,bottom=3pt,fonttitle=\footnotesize\bfseries,coltitle=black,colbacktitle=red!12,title={\tpicon{gemini_pro_icon.png}~Gemini-3.1-Pro\hfill answer: False\tickno}]
\footnotesize\raggedright
Assessing Visual Data

I've begun analyzing the provided 2D perspectives, focusing on column identification within the cube structure.

Mapping the Visual Data

I'm developing a coordinate system and reconstructing the structure from the image's perspective.

Counting Block Structures

I've counted a clear four-block column, carefully tracing edges in Image 2 for validation.

\textit{[[...trimmed output...]]}

% Verifying Height Data

% I have carefully verified Image 2 and Image 1, confirming a three-block height for the lowest columns in each.

% Constructing Spatial Model

% I'm now building a coordinate map (x, y, z), using Image 1 to define the cross shape of top blocks.

% Defining Block Adjacency

% I've established a coordinate system (N, W, C, S, E) and mapped visible top faces in Image 1.

% Clarifying Column Position

% I'm now determining the spatial relationship of the rightmost column relative to block N, revising assumptions.

% Defining Spatial Grid

% I have formalized the spatial grid, clarifying the coordinate system using the image's edges and block faces.

% Validating Visual Predictions

% I am now validating block faces in Image 1 by predicting visibility based on the spatial model.

% Confirming Column Heights

% I've determined block counts for S and NE columns and am now clarifying the center column's height.

% Determining Depth Relationships

% I'm now clarifying the adjacency of S and C by visualizing their parallel, descending right faces.

% Visualizing Coplanar Walls

% Now, I've confirmed the shared wall in Images 1, clarifying the coplanar right faces of C and S.

% Confirming Height Discrepancies

% I've precisely validated Image 1, confirming column C is two blocks, and S is three, disproving prior assumptions.

% Refining 3D Coordinates

% I've clarified the 3D coordinate system, positioning columns W, S, N, and NE relative to column C.

% Verifying Adjacency Relationships

% I've just verified that N's down-right face is hidden by NE, which confirms their adjacency in Image 1.

% Validating Visual Coordinates

% I confirmed NE's down-left face visibility, validating the (x, y) spatial arrangement.

% Analyzing Block Placement

% I am now focusing on W and S's adjacent down-left faces, determining their z-depth relationship.

% Determining Vertical Placement

% I've just resolved W's 2-block height, then N's face visibility in relation to C's positioning.

% Validating Block Heights

% I've just validated column N's up-left face and confirmed its 2-block height within the spatial model.

% Verifying Total Heights

% I just confirmed the total block height, counting "zig-zags," confirming all values are consistent.

% Tracing Top Faces

% I am now carefully tracing Image 2's top, identifying a central hub with three distinct block-branches.

% Mapping Spatial Data

% I've precisely reconstructed the spatial mapping in image 2, associating the hub with column C's coordinates.

% Confirming Spatial Coordinates

% I confirmed S's 3-block height in Image 2, and accurately validated down-left and down-right faces.

% Defining Visual Perspective

% I've just refined the visual perspective for Image 2, precisely mapping axes and visible faces within the model.

% Validating Face Visibility

% I'm now carefully verifying Image 2 by predicting the visual face visibility for each cube's faces.

% Predicting Visible Faces

% I'm now precisely predicting face visibility in Image 2, including for column C and faces hidden by blocks.

% Tracing Column Seams

% I am now tracing the seams between H and S columns, confirming the coplanar +x faces and z-depth in Image 2.

% Determining Face Heights

% I'm now carefully verifying Image 2 by using the faces to validate the spatial model's S-column depth.

% Verifying Edge Lengths

% I've just validated a 3-block height on S by precisely comparing the top face and vertical edge lengths.

% Revisiting Adjacency Analysis

% I've just reconfirmed W's adjacent, hidden down-right face, resolving inconsistencies in the spatial arrangement in Image 2.

% Verifying Cube Heights

% I just reconfirmed S and C, and found a strong visual argument for 3-block height, 2-block C.

% Refining Image Projections

% I've just derived and validated the formulas (u = x+y, v = z+y-x) to map 3D coordinates to 2D image planes.

% Validating Face Visibility

% I've just validated that NE covers N's +x face in Image 2, resolving previous inconsistencies.

% Confirming Depth Constraints

% I've just validated that N cannot be deeper than C and NE by confirming no visible face below in Image 2.

% Revising Projection Formulas

% I've just derived and tested a new set of formulas, mapping 3D coordinates to Image 1's planes.

% Validating Spatial Mapping

% I've just successfully validated the spatial Layout 2 for Image 1 and 2 with an accurate top-face coordinate match.

% Validating Axis Alignment

% I have just confirmed the Layout 2 model and axis orientation against image-specific visible face analysis.

% Revising Height Analysis

% I've re-examined vertical face visibility, leading me to validate the total 2-block height for N in Image 1.

% Refining Face Visibility

% I've just resolved N's height, validating its lack of visible face beneath NE in Image 1.

% Validating Visibility Predictions

% I validated N's +x face invisibility in Image 1, confirming it's hidden behind the C column.

% Revising Height Validation

% I've just confirmed N's height is indeed two blocks by re-examining Image 1's gaps and face visibility.

% Defining Image 2 Axes

% I've just redefined Image 2's coordinate axes, aligning Layout 2's data with visual face directions.

% Confirming Perspective Alignment

% I confirmed that Image 1 and Image 2 share a consistent perspective and axis mapping, which is perfect.

% Verifying Cube Orientation

% I'm now determining if the two image structures can be perfectly matched with a rotation.

% I've mapped spatial data and confirmed both images are indeed consistent with a shared block configuration.

% Validating Depth Relationships

% I've just confirmed Image 2's column height alignment with Image 1, now validating coplanar down-right faces.

% Analyzing Image Inconsistencies

% I am now carefully resolving the visual inconsistencies and validating NE's 2-block height in Image 2.

Concluding Height Data

I've precisely validated that all columns have max height three, thus answering the problem definitively.

Determining Column Max

\tann{annCol10}{I've precisely validated all columns' maximum height as 3 blocks, solving the central challenge definitively.}{Wrong Perception}

Verifying Bounding Box

I validated the bounding box and confirmed no hidden column extends lower than column S.

```json \newline
\{ \newline
"answer": false \newline
\}

```
\end{tcolorbox}

\subsubsection{T7 Color Dominance}
\begin{table}[H]
\centering
\footnotesize
\setlength{\tabcolsep}{1pt}
\renewcommand{\arraystretch}{1.2}
\begin{tabular}{*{9}{>{\centering\arraybackslash}p{\dimexpr\textwidth/9-2\tabcolsep\relax}}}
\toprule
\multicolumn{9}{@{}l@{}}{\itshape ``\ldots{}Your task is to determine the dominant color(s) in the object --- the color(s) with the highest block count\ldots{}''}\\[0.3mm]
\multicolumn{9}{@{}c@{}}{\begin{tabular}{*{2}{c}}\includegraphics[width=0.450\textwidth,height=1.25in,keepaspectratio]{images/app_qual_traces/T7_sample2_row95_query_image_1.png} & \includegraphics[width=0.450\textwidth,height=1.25in,keepaspectratio]{images/app_qual_traces/T7_sample2_row95_query_image_2.png}\end{tabular}}\\[0.5mm]
\textbf{GT} & \tpicon{qwen_icon.png} & \tpicon{gemma_icon.png} & \tpicon{glmv_icon.png} & \tpicon{kimi_icon.png} & \tpicon{grok_icon.png} & \tpicon{gpt_icon.png} & \tpicon{gemini_flash_icon.png} & \tpicon{gemini_pro_icon.png}\\
\threewrap{\cdchip{bedSlategray}&\cdchip{bedTeal}&\cdchip{bedOrange}\\\cdchip{bedOrchid}&&} & \threewrap{\cdchip{bedTeal}&\cdchip{bedSlategray}&\cdchip{bedOrange}\\\cdchip{bedMagenta}&\cdchip{bedBlue}&\cdchip{bedPurple}}\tickno & \threewrap{\cdchip{bedTeal}&&}\tickno & \threewrap{\cdchip{bedTeal}&&}\tickno & \threewrap{\cdchip{bedOrange}&\cdchip{bedTeal}&\cdchip{bedSlategray}\\\cdchip{bedMagenta}&&}\tickno & \threewrap{\cdchip{bedSlategray}&&}\tickno & \threewrap{\cdchip{bedOrange}&\cdchip{bedOrchid}&\cdchip{bedSlategray}\\\cdchip{bedTeal}&&}\tickok & \threewrap{\cdchip{bedTeal}&\cdchip{bedSlategray}&\cdchip{bedOrange}\\\cdchip{bedOrchid}&&}\tickok & \threewrap{\cdchip{bedOrange}&\cdchip{bedOrchid}&}\tickno\\
\bottomrule
\end{tabular}
\caption{T7 Color Dominance.}
\label{tab:qual_trace_t7}
\end{table}
\noindent\textbf{Thinking traces.}\par\smallskip
\begin{tcolorbox}[breakable,enhanced,colback=red!4,colframe=red!55!black,boxrule=0.4pt,arc=1pt,left=4pt,right=4pt,top=3pt,bottom=3pt,fonttitle=\footnotesize\bfseries,coltitle=black,colbacktitle=red!12,title={\tpicon{qwen_icon.png}~Qwen3.5-27B\hfill answer: \tickno}]
\footnotesize\raggedright
The user wants me to identify the dominant color(s) in a 3D object made of blocks, based on two images.

**Image 1 Analysis:** \newline
- This view shows a structure that looks like a cross or a T-shape with an extension. \newline
- Let's break down the visible blocks: \newline
- Top left: Orange block. \newline
- Top middle-left: Teal block. \newline
- Top middle-right: Blue block. \newline
- Top far right: Slategray block. \newline
- \tann{annCol10}{Below the orange block: Teal block. - Below the teal block (middle): Slategray block. - Below the blue block: Teal block.}{Wrong Perception} \newline
- Below the slategray block (far right): Orange block. \newline
- Below the orange block (far right): Magenta block. \newline
- \tann{annCol8}{Wait, let's look closer at the structure. It seems to be a single connected object.}{Reiterating} \newline
- Let's try to map coordinates. Let's say the "front-most" bottom block is at (0,0,0). \newline
- Looking at Image 1: \newline
- T\tann{annCol10}{here's a vertical column on the right side. Top is slategray, below is teal, below is orange, below is magenta.}{Wrong Perception} \tann{annCol8}{Wait, that's not right. - Let's look at the connections.}{Reiterating} \newline
- \tann{annCol10}{Top row (back to front): Orange, Teal, Blue, Slategray?}{Wrong Perception} No, that's not a straight line. \newline
- Let's assume a grid. \newline
- Let's look at the \tann{annCol10}{"cross" shape.}{Wrong Perception} \newline
- There is a central block. Let's assume the blue block is central. \newline
- To its left: Teal. \newline
- \tann{annCol10}{To its right: Teal.}{Wrong Perception} \newline
- \tann{annCol10}{Behind it (top left in image): Orange.}{Wrong Perception} \newline
- \tann{annCol10}{In front of it (bottom left in image): Slategray.}{Wrong Perception} \newline
- \tann{annCol8}{Wait, let's re-evaluate.}{Reiterating} \newline
\textit{[[...trimmed output...]]}\newline
% - Let's look at the top surface. \newline
% - Top surface blocks: Orange (far left), Teal (next to it), Blue (next to that), Slategray (far right). This looks like a row of 4 blocks? No, the perspective is isometric. \newline
% - Let's trace the "top" faces. \newline
% - Block 1 (far left): Orange top face. \newline
% - Block 2 (next to it): Teal top face. \newline
% - Block 3 (next to that): Blue top face. \newline
% - Block 4 (far right): Slategray top face. \newline
% - Wait, looking at Image 1, there is a block with a blue top face. To its left is a teal top face. To the left of that is an orange top face. To the right of the blue top face is a teal top face. To the right of that is a slategray top face. \newline
% - Let's look at the side faces. \newline
% - Far left block: Orange top, Orange side. \newline
% - Next block: Teal top, Teal side. \newline
% - Next block (center-ish): Blue top. \newline
% - Next block: Teal top, Teal side. \newline
% - Far right block: Slategray top, Slategray side. \newline
% - Below the "center" area: \newline
% - \tann{annCol10}{There is a slategray block below the teal/blue area.}{Wrong Perception} \newline
% - There is an orange block below the right teal block. \newline
% - There is a magenta block below the orange block.

% Let's try to reconstruct the object based on both images.

% **Image 2 Analysis:** \newline
% - This view is from a different angle, seemingly rotated. \newline
% - Top surface blocks visible: \newline
% - Far left: Slategray. \newline
% - Next to it: Teal. \newline
% - Next to it: Slategray. \newline
% - Next to it: Teal. \newline
% - Far right: Orange. \newline
% - Wait, let's look at the arrangement. \newline
% - It looks like a \tann{annCol10}{2x4 grid or something similar on top?}{Wrong Perception} \newline
% - Let's look at the "front" face. \newline
% - There is a blue block. \newline
% - To its right: Magenta block. \newline
% - \tann{annCol10}{To its right: Orange block.}{Wrong Perception} \newline
% - Below the blue block: Purple block? No, looks like a dark purple/magenta side. \newline
% - Below the magenta block: Nothing visible directly below, but there's a block to the left. \newline
% - Let's look at the bottom left. \newline
% - There is a magenta block at the very bottom front. \newline
% - Above it: Orange block. \newline
% - To the right of the orange block: Purple block (side visible). \newline
% - To the right of the purple block: Magenta block (top visible).
\tann{annCol8}{This is getting confusing. Let's try to map specific blocks.}{Reiterating}

**Let's assume a coordinate system (x, y, z) where x is left-right, y is up-down, z is front-back.**

**From Image 1:** \newline
- It looks like a "T" shape lying on its side or a cross. \newline
- Let's identify distinct blocks. \newline
- Block A: Top-leftmost. Orange top, Orange side. \newline
- Block\tann{annCol0}{I have to give the solution based on the reasoning directly now.}{Budget Hit}
\end{tcolorbox}
\begin{tcolorbox}[breakable,enhanced,colback=red!4,colframe=red!55!black,boxrule=0.4pt,arc=1pt,left=4pt,right=4pt,top=3pt,bottom=3pt,fonttitle=\footnotesize\bfseries,coltitle=black,colbacktitle=red!12,title={\tpicon{grok_icon.png}~Grok-4.20\hfill answer: \tickno}]
\footnotesize\raggedright
The problem involves determining the dominant color(s) in a 3D object made of colored blocks from two perspective images. \newline
I need to figure out the dominant colors in this 3D object made of colored blocks, using two perspective views. The object combines blocks in colors like yellow, cyan, green, magenta, red, orange, orchid, teal, slategray, gold, blue, purple. From the images, I see orange,magenta or orchid, blue, teal or cyan, slategray, and purple. In the first image, orange and magenta appear multiple times, blue once, teal a few times, gray a few. The second image adds a darker purple. To find the dominant colors, I count the blocks of each color across both views, accounting for the 3D structure and hidden blocks. \tann{annCol10}{After tallying, the colors with the most blocks are orange and gray,}{Wrong Perception} but let's double-check the counts. Upon closer inspection, orange appears in several positions, gray in others, \tann{annCol2}{but teal seems prominent too.}{Good Intuition} Actually, after reconstructing, \tann{annCol10}{the dominant colors are orangeand magenta, as they have the highest count in the visible parts and structure}{Wrong Perception}. The problem says "dominant color(s)", plural possible, and only consider predefined colors. Confirming all visible colors are included: orange, magenta, blue, teal, slategray, purple. But counts show \tann{annCol10}{orange has 4 blocks, gray3, magenta 3, teal 3, blue 2,}{Wrong Perception} purple 1. So orange is dominant, but since plural, orange and gray/magenta. But the example is list[str], so multiple possible. \tann{annCol10}{I think the answer is orange and magenta as they seem most prominent. But to be precise, let's say orange, gray, and teal are the most.}{Wrong Perception} But the task is dominant, so the one(s) with the highest number. 
\textit{[[...trimmed output...]]}
% If tie, all with max. So if orange and others tie for most, include all. After all this, I conclude the dominant colors are orange and slategray. Butslategray is gray. But let's decide orange, slategray, and perhaps teal. But the response must be in the format `\{ 'answer': list[str], \}` So I need to output only that. But since no actual images, I have to guess based on the trace. The trace suggests colors like orange,magenta, gray, teal. The dominant seem to be gray and teal. In the trace, it says gray and teal seem to have 3 each. So perhaps ['slategray', 'teal']. But the colors are given as slategray, teal. But in the problem, it's predefined, so use the exactnames. The predefined colors are listed, so use those. Magenta is listed, orchid is different. Orchid is a type of magenta? But in the trace, it's called orchid perhaps. The trace says orchid. But the problem says predefined ...(1063 chars truncated)... so assume the colors are as named. For thedominant, the trace mentions gray and teal seem prominent. So I think the dominant colors are slategray and teal. 
\tann{annCol10}{So the answer is ['slategray', 'teal']. But the trace says "gray and teal seem to have 3 each"}{Wrong Perception}. So they are co-dominant. But the problem is to find dominant color(s), plural possible. But in the example, it's 'red', 'blue']. So list. But is it only two? The trace has more. But to prioritize coherence, I'll go with that. But the trace later says orange and gray, but then teal. It's inconsistent, but the last part is gray andteal. Let's see the last line: "So the dominant colors are slategray and teal." No, the trace cuts off. But in the trace, it says "gray and teal seem to have 3 each". So they are co-dominant. But the problem is to find dominant color But the problem is to saydominant, and if tie, perhaps both. \tann{annCol10}{But the trace later mentions slategray with 4, which is dominant. In the middle, it says slategray with 4, others less. So slategray is the dominant. But then it says gray and teal with 3 each. It's inconsistent, but the laterpart has slategray with 4. So I'll go with slategray as the dominant color.}{Wrong Perception} But the problem allows list, so perhaps ['slategray']. But the trace says "dominant is slategray with 4". So that seems the latest. But the output format is list[str], so ['slategray']. Butthe problem says "dominant color(s)", implying possibly multiple. But if one, then one. But to be safe, let's see if there is tie. The trace says "4 gray, 3 teal, 3 magenta, 2 orange, 1 blue, 1 purple". So slategray has 4, which is the most. Dominant is slategray. The answer is \{'answer': ['slategray']\}. But the trace says "gray" but predefined is "slategray". Yes, slategray. 
\tann{annCol8}{But in the beginning I thought gray, but it's slategray. Yes. But the trace says "gray/slategray". Yes, slategray. But then it says "4 gray, 3 teal". Yes. But then later "4 teal, 4 gray". It's conflicting. The trace is inconsistent. The trace says "4 gray, 3 teal, 2 orange, 2 magenta, 1 blue, and1 purple". Then "4 gray, 3 teal". Then "4 gray, 3 teal". \textit{[[...trimmed output...]]}
% Then "4 gray, 3 teal". Then "4 gray, 3 teal". Then "4 gray, 3 teal". Then "4 gray, 3 teal". Then "4 gray, 3 teal". Then "4 gray, 3 teal". Then "4 gray, 3 teal". Then "4 gray, 3 teal". Then "4 gray, 3 teal". Then "4 gray, 3 teal". Then "4 gray, 3 teal". Then "4 gray, 3teal". Then "4 gray, 3 teal". Then "4 gray, 3 teal". Then "4 gray, 3 teal". Then "4 gray, 3 teal". Then "4 gray, 3 teal". Then "4 gray, 3 teal". Then "4 gray, 3 teal". Then "4 gray, 3 teal". Then "4 gray, 3 teal". Then "4 gray, 3 teal". Then "4 gray, 3 teal". Then "4 gray, 3 teal". Then "4 gray, 3 teal". Then "4 gray, 3 teal".Then "4 gray, 3 teal". Then "4 gray, 3 teal". Then "4 gray, 3 teal". Then "4 gray, 3 teal". Then "4 gray, 3 teal". Then "4 gray, 3 teal". Then "4 gray, 3 teal". Then"4 gray, 3 teal".Then "4 gray, 3 teal". Then "4 blocks gray, 3 teal". Then "4 blocks gray, 3 teal". Then "4 blocks gray, 3 teal". 
Then "4 blocks gray, }{Reiterating}Assistant: The dominant colors are gray and teal,with 4 blocks each, and orange with 3. But the problem is to determine the dominant color(s), and since it's plural, perhaps both. But let's see the output format. 
\textit{[[...trimmed output...]]}
% I think the answer is slategray and teal. Since slategray is gray, and teal is teal. So the dominant are slategray and teal. The other colors have fewer blocks. So the answer should be ['slategray', 'teal']. But in the problem, the colors are given as names like slategray. Yes. So I'll go with that. The final answer is slategray and teal. But to confirm, all visible colors areincluded, and no hidden ones are dominant. Yes. So the dominant colors are slategray and teal.The final answer is slategray and teal. 
But the output format is a JSON with 'answer' as list of str. \tann{annCol10}{So \{'answer': ['slategray', 'teal']\} But in the internal reasoning, it was slategray dominant with 4, others 3 or less.}{Wrong Perception}
\end{tcolorbox}
\begin{tcolorbox}[breakable,enhanced,colback=green!4,colframe=green!50!black,boxrule=0.4pt,arc=1pt,left=4pt,right=4pt,top=3pt,bottom=3pt,fonttitle=\footnotesize\bfseries,coltitle=black,colbacktitle=green!14,title={\tpicon{gpt_icon.png}~GPT-5\hfill answer: \tickok}]
\footnotesize\raggedright
Determining dominant colors in the cubes \newline
I need to figure out the dominant colors in these cubes. There are 3D cubes with colored faces, and I should count each color. I'll inspect the images carefully, checking for shades like orange, gold, teal, slategray, blue, orchid, and purple. Orange and gold might need clearer distinction, but both belong to the preset colors. Let's verify! \newline
Identifying cubes and colors \newline
I'm looking at the cubes in the image, and most likely, the orange is just saturated orange, not yellow or gold. The visible cubes include orange, teal, blue, slategray, orchid, and purple. I'll take an isometric view and try to identify their precise positions. From the first view, the top row shows a series of cubes including orange, orchid, blue, and slategray, arranged in a horizontal bar. \newline
Confirming visible positions and colors across cubes \newline
\tann{annCol10}{From the image, I can see the following cubes: a purple one at the bottom, teal and orange cubes with an orchid below. }{Wrong Perception}For the vertical view, I observe an arrangement of slategray, teal, blue, and orange cubes. There are a total of seven top faces visible, and I can identify several legs or vertical sides, including orange and orchid cubes positioned under the main cubes. \newline
Counting visible cubes from two views \newline
I'm thinking about how to count the cubes. Since the object is likely made of colored unit cubes arranged in a 3D grid, only the visible cubes should be counted, and hidden cubes might not need to be included unless partially visible. I'll avoid double-counting by considering both views carefully and inferring occlusion. \newline
Identifying cubes and their positions \newline
\tann{annCol3}{The top layer seems to have about seven cubes. The bottom layer supports the structure with vertical cubes. Under some of the top cubes are lower cubes, like the orange cube below blue/teal and the orchid cube beneath orange. I'll check for any magenta purple cubes below blue and confirm the counts. }{Good Perception}We may also use image coordinates for position detection. \newline
Identifying cube positions and colors in images \newline
\tann{annCol9}{from PIL import Image import matplotlib.pyplot as plt img1=Image.open('/mnt/data/T7\_sample2\_row95\_query\_image\_1.png') img2=Image.open('/mnt/data/T7\_sample2\_row95\_query\_image\_2.png') img1.size, img2.size Matplotlib is building the font cache; this may take a moment. ((409, 409), (409, 409))}{Tool Use} \newline
Counting cubes and detecting colors in images \newline
Output image \newline
Analyzing the geometry and census of cubes \newline
\textit{[[...trimmed output...]]} \newline
% Let's use the isometric projections to analyze the cube arrangement. The top layer looks like a 3x3 grid, minus some gaps, with hanging legs. After mapping the grid, I observe the following possible counts for colors: slategray, teal, orchid, orange, blue, and purple, each with varying quantities. I'll ensure all cubes are labeled carefully by color, starting with the observed visible cubes from the first view: orange (O1), orchid (Or1), and blue (B1). \newline
% Mapping the visible blocks from two views \newline
% In View1, I've identified cubes with colors like slategray (S1 and S2), teal (T1 and T2), and orange (O1 and O2). The visible faces are being carefully labelled for clarity. In View2, there's some ambiguity between which slategray cube belongs where and if some other cubes are hidden behind others. I'll continue to refine my color count and spatial mapping. \newline
% Clarifying cube colors and shading \newline
% I'm examining a cube in view2 that might be purple, as the dark magenta side appears more substantial than just shading on an orchid cube. Shading can make parts look darker, but it's important to count only actual colors. I'll need to distinguish between shading variations and true color when labeling cubes. \newline
% Deciding between purple and orchid coloring \newline
In the first view, I don't see a distinct purple cube, and the dark face in view2 could just be a shaded side of an orchid cube. Since the color palette includes both purple and orchid, I need to examine the top face for clearer identification. I'll sample pixel colors to distinguish the shades. \newline
Identifying cube colors from image sampling \newline
\tann{annCol9}{import numpy as np from PIL import Image for img, name in [(img1,'img1'),(img2,'img2')]: arr=np.array(img.convert('RGB')) \# get non-white, non-black pixels pixels=arr.reshape(-1,3) \# count colors exact import collections cnt=collections.Counter(map(tuple,pixels)) top=cnt.most\_common(20) print(name, top[:10]) \# unique non white non black approximate list colors=[(c,n) for c,n in cnt.most\_common() if c!=(255,255,255) and c!=(0,0,0)] print(colors[:20]) img1 [((np.uint8(255), np.uint8(255), np.uint8(255)), 118105), \textit{[[...trimmed output...]]}
% ((np.uint8(112), np.uint8(128), np.uint8(144)), 12399), ((np.uint8(0), np.uint8(128), np.uint8(128)), 9819), ((np.uint8(255), np.uint8(165), np.uint8(0)), 7891), ((np.uint8(218), np.uint8(112), np.uint8(214)), 7130), ((np.uint8(0), np.uint8(0), np.uint8(0)), 3985), ((np.uint8(0), np.uint8(0), np.uint8(255)), 2741), ((np.uint8(207), np.uint8(207), np.uint8(207)), 100), ((np.uint8(0), np.uint8(5), np.uint8(5)), 62), ((np.uint8(5), np.uint8(3), np.uint8(0)), 58)] [((np.uint8(112), np.uint8(128), np.uint8(144)), 12399), ((np.uint8(0), np.uint8(128), np.uint8(128)), 9819), ((np.uint8(255), np.uint8(165), np.uint8(0)), 7891), ((np.uint8(218), np.uint8(112), np.uint8(214)), 7130), ((np.uint8(0), np.uint8(0), np.uint8(255)), 2741), ((np.uint8(207), np.uint8(207), np.uint8(207)), 100), ((np.uint8(0), np.uint8(5), np.uint8(5)), 62), ((np.uint8(5), np.uint8(3), np.uint8(0)), 58), ((np.uint8(83), np.uint8(95), np.uint8(107)), 57), ((np.uint8(8), np.uint8(8), np.uint8(8)), 56), ((np.uint8(2), np.uint8(1), np.uint8(2)), 56), ((np.uint8(0), np.uint8(120), np.uint8(120)), 56), ((np.uint8(3), np.uint8(2), np.uint8(0)), 55), ((np.uint8(13), np.uint8(14), np.uint8(16)), 55), ((np.uint8(0), np.uint8(54), np.uint8(54)), 54), ((np.uint8(0), np.uint8(15), np.uint8(15)), 54), ((np.uint8(36), np.uint8(23), np.uint8(0)), 53), ((np.uint8(88), np.uint8(88), np.uint8(88)), 53), ((np.uint8(109), np.uint8(70), np.uint8(0)), 52), ((np.uint8(82), np.uint8(93), np.uint8(105)), 51)] img2 [((np.uint8(255), np.uint8(255), np.uint8(255)), 119044), ((np.uint8(218), np.uint8(112), np.uint8(214)), 10387), ((np.uint8(112), np.uint8(128), np.uint8(144)), 9790), ((np.uint8(255), np.uint8(165), np.uint8(0)), 6411), ((np.uint8(0), np.uint8(128), np.uint8(128)), 4875), ((np.uint8(0), np.uint8(0), np.uint8(255)), 4392), ((np.uint8(0), np.uint8(0), np.uint8(0)), 4186), ((np.uint8(128), np.uint8(0), np.uint8(128)), 3076), ((np.uint8(1), np.uint8(1), np.uint8(1)), 96), ((np.uint8(2), np.uint8(1), np.uint8(2)), 62)] [((np.uint8(218), np.uint8(112), np.uint8(214)), 10387), ((np.uint8(112), np.uint8(128), np.uint8(144)), 9790), ((np.uint8(255), np.uint8(165), np.uint8(0)), 6411), ((np.uint8(0), np.uint8(128), np.uint8(128)), 4875), ((np.uint8(0), np.uint8(0), np.uint8(255)), 4392), ((np.uint8(128), np.uint8(0), np.uint8(128)), 3076), ((np.uint8(1), np.uint8(1), np.uint8(1)), 96), ((np.uint8(2), np.uint8(1), np.uint8(2)), 62), ((np.uint8(40), np.uint8(40), np.uint8(40)), 60), ((np.uint8(108), np.uint8(123), np.uint8(138)), 60), ((np.uint8(34), np.uint8(34), np.uint8(34)), 58), ((np.uint8(161), np.uint8(104), np.uint8(0)), 58), ((np.uint8(116), np.uint8(59), np.uint8(114)), 58), ((np.uint8(150), np.uint8(150), np.uint8(150)), 57), ((np.uint8(28), np.uint8(32), np.uint8(37)), 57), ((np.uint8(114), np.uint8(58), np.uint8(112)), 57), ((np.uint8(143), np.uint8(92), np.uint8(0)), 57), ((np.uint8(204), np.uint8(104), np.uint8(200)), 57), ((np.uint8(0), np.uint8(0), np.uint8(105)), 56), ((np.uint8(56), np.uint8(29), np.uint8(55)), 55)]
}{Tool Use} \newline
Counting cubes and identifying faces by visibility \newline
\textit{[[...trimmed output...]]}\newline
% The purple cube is only visible in view2, so I need to focus on that image for the purple count. The exact pixel area doesn't match cube count due to face visibility, but I can infer positions from projection coordinates. By analyzing the top and side faces, I can identify and count each unique cube. \newline
% Counting visible cubes and determining colors \newline
% I'm mapping the cube positions and checking visibility across the two views. Based on the areas and visibility calculations, orchids, oranges, \newline
% Finding centroids with segmentation \newline
% I want to find the centroids of the top face colors by segmenting the image, making sure to use exact colors. Though, connected components might merge adjacent faces of the same color. I'll inspect image1 by overlaying coordinates to better visualize and calculate the centroids using these segmented components. \newline
% Visualizing image with coordinate grid \newline
% Output imageOutput image \newline
% Checking cube grid and positioning \newline
% I'm analyzing the isometric projection coordinates for the cubes. The goal is to understand how their top faces align, so I'm examining vertices for various cubes like Orchid, Blue, Teal, and Gray cubes. I plan to confirm if the grid is consistent with diagonal (u, v) basis vectors and check if certain cubes are adjacent. I'll need to ensure correct center coordinates and spacing. \newline
% Analyzing cube positions and grid alignment \newline
% I'm breaking down the grid for the cubes based on their edges and positions. I identified vectors for the cubes, like TealL and Blue sharing an edge. It looks like I've established a grid arrangement for the top layer's top surfaces of cubes at the highest stack. These surfaces may be offset due to different stack heights. \newline
% Analyzing cube stacking and vertical alignment \newline
% It looks like the orange and orchid cubes are vertically stacked in the same position, with orange on top and partially hiding the orchid's top. The setup suggests there are at least two cubes in the same vertical stack at a coordinate below the top-layer cubes. View2 shows this vertical relationship clearly. \newline
% Examining lower stacked cubes in view2 \newline
% I've identified a stack of two cubes: orange on top and orchid below, positioned at the bottom front-left. Additionally, the blue cube is visible with its vertical side, possibly stacked, and there's a darker purple cube below it. I need to confirm if the purple block is another cube beneath the blue one. \newline
% Investigating purple cube position and visibility \newline
% It seems like the dark purple face could be the side of a cube beneath the blue one, forming a two-cube stack (blue on top, purple below). The purple cube might be blocked by front gray/teal in some views. The orchid cube below the orange seems to align similarly in another view, with additional visible faces. \newline
% Cropping and displaying image sections \newline
% Output imageOutput image \newline
% Analyzing cube positions and shading \newline
% In Image2, the purple cube has a large vertical face beneath the blue, with a horizontal face on the right. The orchid cube on the left shows uniform coloring, with no shading. The large orchid cube on the front right has side faces visible, though all faces seem to share the same color without shading, except for black outlines. The orange triangle is part of the orange cube behind the orchid. \newline
% Counting and verifying cubes and layers \newline
It seems there's a vertical stack involving orange and orchid cubes, bringing the total count to 10 or 11. In Image1, the stack on the right shows orange and orchid cubes but likely no new additions. The color areas are clearer in \tann{annCol3}{Image2: orchid has 2 cubes, as does orange, slate, and teal. My final count: 2 for each of these colors, and 1 each for blue and purple, balancing things out.}{Good Perception}

```python \newline
\{ \newline
'answer': ['orange', 'orchid', 'slategray', 'teal'], \newline
\} \newline
```
\end{tcolorbox}
\begin{tcolorbox}[breakable,enhanced,colback=green!4,colframe=green!50!black,boxrule=0.4pt,arc=1pt,left=4pt,right=4pt,top=3pt,bottom=3pt,fonttitle=\footnotesize\bfseries,coltitle=black,colbacktitle=green!14,title={\tpicon{gemini_flash_icon.png}~Gemini-3-Flash\hfill answer: \tickok}]
\footnotesize\raggedright
To find the dominant color(s), let's break down the 3D structure by analyzing the arrangement and counting the individual blocks belonging to each color from the predefined set (yellow, cyan, green, magenta, red, orange, orchid, teal, slategray, gold, blue, purple).

\#\#\# 1. Identify and Count the Blocks by Color

* **Teal:** * \tann{annCol3}{In Image 1, we clearly see a diagonal row of 2 teal blocks forming part of the central structure.}{Good Perception} \newline
* **Total Count = 2**

* **Slategray:** * \tann{annCol3}{In Image 1, there are 2 slategray blocks extending outward from the sides of the teal/blue center.}{Good Perception} \newline
* **Total Count = 2**

* **Orange:** * T\tann{annCol3}{here is 1 orange block at the top-left edge in Image 1, and 1 orange block extending downwards on the right-hand column.}{Good Perception} \newline
* **Total Count = 2**

* **Orchid / Light Purple:** * \tann{annCol3}{There is 1 orchid block at the very top edge next to the orange/blue blocks. * There is another orchid block at the very bottom of the vertical extension.}{Good Perception} \newline
* **Total Count = 2**

* **Blue:** * \tann{annCol3}{There is 1 bright blue block situated right in the center.}{Good Perception} \newline
* **Total Count = 1**

* **Purple:** * \tann{annCol3}{Visible in Image 2 tucked underneath the blue/orchid blocks.}{Good Perception} \newline
* **Total Count = 1**

\#\#\# 2. Determine the Dominant Colors

\tann{annCol3}{The colors with the highest block count are **teal, slategray, orange, and orchid**, each having a count of 2 blocks.}{Good Perception}

```json \newline
\{ \newline
"answer": ["teal", "slategray", "orange", "orchid"] \newline
\}

```
\end{tcolorbox}
\begin{tcolorbox}[breakable,enhanced,colback=red!4,colframe=red!55!black,boxrule=0.4pt,arc=1pt,left=4pt,right=4pt,top=3pt,bottom=3pt,fonttitle=\footnotesize\bfseries,coltitle=black,colbacktitle=red!12,title={\tpicon{gemini_pro_icon.png}~Gemini-3.1-Pro\hfill answer: \tickno}]
\footnotesize\raggedright
Analyzing Object Colors

I've begun color analysis, identifying orchid, magenta, and purple on the top layer of the first image.

Mapping Block Relationships

I've established a coordinate system and mapped several block positions relative to each other, like the orchid and orange stack.

Refining Block Coordinates

I've established a refined coordinate system and accurately placed blocks, like orange and teal, within the image.

Refining Block Relationships

I've established a refined coordinate system to map block relationships, and validated the 2x2 square formation.

Extending Block Mapping

I've precisely located Slategray and additional Teal blocks, confirming their spatial arrangement in the image.

Revising Block Layout

I am revising color observations to refine block arrangement and spatial adjacency within the image.

Clarifying Block Face

I'm now identifying Slategray and Teal faces, using 3D projections to resolve visual ambiguities within the image.

Determining Z-Levels

I've determined block z-levels in Image 1, confirming S1 and S2 at z=0, \tann{annCol10}{T1, Blue, and Orchid at z=1.}{Wrong Perception}

Confirming Block Geometry

I've resolved block face adjacencies using image analysis, \tann{annCol10}{confirming the 2x2 grid at z=1.}{Wrong Perception}

\textit{[[...trimmed output...]]}

% Resolving Block Orientations

% I've resolved the Slategray face orientation, distinguishing its front-left face below T1 in Image 1.

% Interpreting Isometric Views

% I've clarified block orientations based on isometric projections and face visibility in Image 1.

% Validating Block Coordinates

% I've validated the coordinates of the 2x2 blocks and re-evaluated the surrounding blocks' coordinates within Image 1.

% Validating Block Coordinates

% I've validated the coordinates of the 2x2 blocks and re-evaluated the surrounding blocks' coordinates within Image 1.

% Refining Coordinate System

% I'm now revising my coordinate system to use a + shape, and applying it to accurately represent the layout of blocks in Image 1.

% Analyzing Block Placement

% I've resolved Blue's visibility issue, determining its z-level and orientation within the isometric view.

% Confirming Block Adjacency

% I've determined Teal blocks at (1,1) have their front faces occluded by Slategray, revealing an Orange block underneath.

% Refining Block Adjacency

% I've revised the 2x2 layer's face visibility, clarifying block adjacency and occlusion within Image 1.

% Confirming Block Location

% I've determined Slategray's location as (0,2,1) and confirmed its relationship with surrounding blocks in the image.

% Confirming Block Faces

% I've precisely identified Slategray and Blue front-right faces, confirming spatial relationships in the block arrangement.

% Confirming Block Faces

% I've determined that the "notch" at (2,0) and Slategray faces meet, validating the z=1 layer's geometry.

% Determining Block Position

% I've determined an Orchid block at (1,1,0), resolving occlusion issues with Slategray at z=1.

% Confirming Block Geometry

% I've determined a new block layout with Orange at (2,2,0) and Orchid at (2,2,-1) from the image analysis.

% Revising Block Layout

% I am revising color observations to refine block arrangement and spatial adjacency within the image, particularly Orchid.

% Determining Block Position

% I've determined a new block layout, confirming an Orange block at (2,2,-1) from Slategray's visual projection.

% Confirming Block Geometry

% I've determined an Orange block at (2,2,0), confirming its adjacency with two Slategray blocks within z-level.

% Resolving Block Colors

% I'm now identifying that the top block's top face is Gold, validating the new block model in Image 1 and 2.

% Revising Block Configuration

% I'm now revising block assignments by comparing cross-shaped relationships and face adjacencies across images.

% Mapping Block Relationships

% I've precisely located Slategray (1,-1) relative to Purple (1,0) in Image 2, validating coordinate alignments.

% Validating Block Alignment

% I've validated the image's block layout, mapping z=1 with eight blocks, and confirmed an Orchid block under Purple.

% Matching Image Layout

% I've resolved the 180-degree image rotation mismatch, correctly identifying Image 1's view as a mirrored layout.

% Revising Block Coordinate

% I've revised the block coordinates to accurately reflect their arrangement and color associations within the images.

% Revising Block Layouts

% I've updated my mappings using a mirrored perspective, and the blocks' positions now align with the image's view.

% Determining Block Perspective

% I've determined that Image 1's view is from the +x, -y direction, clarifying Slategray's visual dominance.

% Clarifying View Directions

% I've determined a view direction of (+1,-1), aligning image block projections with spatial coordinate mapping.

% Mapping Block Geometry

% I've determined a new layout with Slategray (0,0), Teal (0,1), and Orange (0,2) forming a line.

% Confirming Block Geometry

% I've determined a new block layout, confirming a 2x2 square: Slategray, Teal, and Blue blocks in Image 2.

% Validating Block Arrangement

% I've precisely validated block arrangements in z=0 and z=1, confirming an eight-block layer with (2,1,0) Orchid.

% Confirming Block Geometry

% I've determined an Orchid block exists at (2,2,0), hidden from the top view, based on image face analysis.

% Revising Color Identification

% I'm now re-identifying Image 1's colors based on known blocks from Image 2 to align perspectives.

% Resolving Block Colors

% I'm now identifying that the block under Teal may be gold, re-evaluating color mapping from Image 1's view.

% Validating Block Structure

% I've validated the eight-block configuration's structure, confirming the isometric image's layout and block positions.

% Revising Block Colors

% I'm now determining an alternative configuration in Image 1, hypothesizing Teal at (0,0) and reevaluating block assignments.

% Revising View Perspective

% I've determined Image 1 uses a (-x,-y) view direction, and am now generating the blocks' perspectives from that view.

% Determining View Direction

% I've determined a new image perspective using (+x, +y), suggesting two blocks are on z=0 and z=-1.

% Revising Block Layout

% I am revising color observations, and have identified that Orange has a visible Top face in Image 2.

% Revising Block Projections

% I'm now revising block projections from different views, seeking consistency between Images 1 and 2 after considering Purple and Orchid issues.

% Analyzing View Direction

% I've determined (+x,+y) aligns with Image 1's top-view blocks, viewing the layout from that perspective.

% Revising View Perspective

% I've determined (+x, -y) is incorrect, so I will now analyze the perspective using the opposite view direction.

% Revising Block Counts

% I'm now counting colors carefully, correcting block lists for both images after comparing color distributions for accurate mapping.

% Confirming Block Geometry

% I've determined an Orange block at (1,0,0) based on Image 1, and am re-evaluating that block's position relative to the Teals.

% Resolving Block Counts

% I'm now integrating insights from both image perspectives, discovering Slategray positions form a right angle.

% Determining Block Positions

% I've determined a new block layout, confirming three blocks: Slategray (-1,0), Teal (0,0), and Orange (1,0) in Image 2, forming a line.

% Mapping Block Connections

% I've determined a new image layout for Image 2, precisely locating Blue, Orchid, and Purple blocks in spatial coordinates.

% Revising Block Layout

% I've re-examined the axes, resolving the second Teal's position and correctly mapping block locations in Image 2.

% Counting Block Instances

% I've determined a minimum of ten blocks are present by summing top face counts, considering two Teals and Orchids are needed.

% Validating Block Arrangement

% I've validated the eight-block layout across both images, confirming Purple, Blue, Teal, Orange, and two Slategray blocks at z=1, with an Orchid and Orange at z=0.

% Refining Block Configuration

% I'm now identifying that the two views hide different blocks, and have a good block total count.

% Validating Block Counts

% I've validated the total block count at ten, confirming two each of Slategray, Teal, Orange, and Orchid, plus one Purple and Blue.

% Revising Color Mapping

% I'm now considering color reinterpretation, exploring if Orchid and Purple represent a single color with lighting variation.

% Verifying Block Colors

% I'm now identifying that orchid, slategray, orange, and teal are distinct, verifying the block color counts.

% Refining Block Adjacency

% I'm now identifying that all inferred block positions connect via shared faces, ensuring contiguous structure.

% Connecting Block Layers

% I've determined a (1,0,0) block, now identifying it as Orchid in Image 2, and confirmed a complete, contiguous z=1 block structure.

% Confirming Block Rotation

% I'm now integrating all images, validating Image 2's structure by resolving the view rotation within Image 1.

% Mapping Block Position

% I've determined a new layout with Teal as the central block at (0,0,1), confirming Orange, Blue, and two Slategrays' arrangement in Image 1.

% Refining Block Orientation

% I've determined a model error, and am now revising block positions, starting with the relative orientation of Purple and Orchid.

% Verifying Block Counts

% I've precisely validated block counts, confirming ten total blocks: two each of Teal, Orchid, Orange, Slategray.

% Aligning Block Models

% I've precisely integrated Image 2 blocks into Image 1's model, resolving block adjacency and confirming layout accuracy.

% Validating Block Coordinates

% I've validated the presence of the hidden Orchid at (-1,-1,0) in Image 2, and confirmed Orchid1 (1,1,-1).

% Extending Block Counts

% I've determined a third Orchid block at (1,1,-1), and am evaluating the possibility of a third Orange block.

% Refining Block Count

% I've precisely validated block counts, determining eleven blocks, and rechecked Orchid/Purple for consistency.

% Confirming Block Count

% I've determined a third Orange block exists at (1,-2) and am rechecking block color distributions across all views.

% Validating Block Visibility

% I've validated that Blue's placement occludes Teal, and revised the model's block positions.

% Confirming Block Count

% I've precisely validated all block positions across images, confirming a final count of twelve blocks total.

Analyzing Block Contiguity

I'm now analyzing contiguity and identifying that Orange (1,1,0) requires a block at (1,0,0) or (0,1,0) for structural integrity.

Revising Block Configuration

I'm now re-evaluating Orchid identification, considering a potential fourth Orchid and verifying color counts.

```json \newline
\{ \newline
"answer": ["orange", "orchid"] \newline
\}

```
\end{tcolorbox}

\subsubsection{T8 Silhouette Symmetry}
\begin{table}[H]
\centering
\footnotesize
\setlength{\tabcolsep}{1pt}
\renewcommand{\arraystretch}{1.2}
\begin{tabular}{*{9}{>{\centering\arraybackslash}p{\dimexpr\textwidth/9-2\tabcolsep\relax}}}
\toprule
\multicolumn{9}{@{}l@{}}{\itshape ``\ldots{}Your task is to determine whether the object's silhouette is symmetric (vertically or horizontally)\ldots{}''}\\[0.3mm]
\multicolumn{9}{@{}c@{}}{\begin{tabular}{*{2}{c}}\includegraphics[width=0.450\textwidth,height=1.25in,keepaspectratio]{images/app_qual_traces/T8_sample2_row78_query_image_1.png} & \includegraphics[width=0.450\textwidth,height=1.25in,keepaspectratio]{images/app_qual_traces/T8_sample2_row78_query_image_2.png}\end{tabular}}\\[0.5mm]
\textbf{GT} & \tpicon{qwen_icon.png} & \tpicon{gemma_icon.png} & \tpicon{glmv_icon.png} & \tpicon{kimi_icon.png} & \tpicon{grok_icon.png} & \tpicon{gpt_icon.png} & \tpicon{gemini_flash_icon.png} & \tpicon{gemini_pro_icon.png}\\
True & False\tickno & False\tickno & False\tickno & True\tickok & False\tickno & False\tickno & False\tickno & False\tickno\\
\bottomrule
\end{tabular}
\caption{T8 Silhouette Symmetry.}
\label{tab:qual_trace_t8}
\end{table}
\noindent\textbf{Thinking traces.}\par\smallskip
\begin{tcolorbox}[breakable,enhanced,colback=red!4,colframe=red!55!black,boxrule=0.4pt,arc=1pt,left=4pt,right=4pt,top=3pt,bottom=3pt,fonttitle=\footnotesize\bfseries,coltitle=black,colbacktitle=red!12,title={\tpicon{gemma_icon.png}~Gemma4-31B\hfill answer: False\tickno}]
\footnotesize\raggedright
* The goal is to determine if the silhouette of the 3D object is symmetric. \newline
* Two perspective views are provided. \newline
* Symmetry can be vertical or horizontal. \newline
* The silhouette is the 2D outline of the object from a given perspective.

* View 1: \newline
* \tann{annCol10}{Top layer: 3 blocks (forming an L-shape or similar).}{Wrong Perception} \tann{annCol8}{Let's re-examine.}{Reiterating} \newline
* Looking at the top surface: \tann{annCol10}{There are 3 blocks. One is at the back-left, one in the middle, and one at the back-right.}{Wrong Perception} \tann{annCol8}{Wait, let's look closer.}{Reiterating} \newline
* \tann{annCol10}{Top surface blocks: * (0, 1, 1) - back left * (1, 1, 1) - middle * (2, 1, 1) - back right}{Wrong Perception} \tann{annCol8}{(Wait, it's more like a 2x2 area with one missing? No.) * Let's re-count the blocks in View 1:}{Reiterating} \newline
* \tann{annCol10}{Top layer: 3 blocks. * Middle layer: 4 blocks. * Bottom layer: 3 blocks.}{Wrong Perception} \newline
* Wait, let's look at the silhouette (the outer boundary). \newline
* View 1 silhouette: \newline
* Top edge: a line. \newline
* \tann{annCol10}{Left edge: a vertical line. * Right edge: a vertical line. * Bottom edge: a jagged line. * Let's trace the outer boundary of View 1: * Top-left corner to top-right corner. * Top-right corner down to a point. * Then it goes in and down. * Then it goes left and down. * Then it goes left. * Then it goes up. * Then it goes left and up. * Then it goes up to the top-left corner. * Is this silhouette symmetric? * Vertical symmetry: Left side vs. right side. * Left side has a block sticking out at the bottom? No, the right side has a block sticking out more.}{Wrong Perception} \newline
* \tann{annCol8}{Let's re-examine View 1's silhouette.}{Reiterating} \newline
* \tann{annCol10}{Leftmost point: (x=0, y=middle) * Rightmost point: (x=max, y=middle) * Topmost point: (x=middle, y=0) * Bottommost point: (x=middle, y=max) * Looking at the image, the left side has a block at the bottom, and the right side also has a block at the bottom.}{Wrong Perception} \newline
* \tann{annCol8}{Let's count the "steps" on the left and right.}{Reiterating} \newline
* \tann{annCol10}{Left side: from top, it goes down, then slightly in, then down, then slightly out. * Right side: from top, it goes down, then slightly in, then down, then slightly out. * Wait, let's look at the bottom edge. It's not a straight line. It goes up, then across, then down, then across, then up.}{Wrong Perception} \newline
* \tann{annCol8}{Let's re-examine the silhouette of View 1.}{Reiterating} \newline
* Left side: 2 blocks high at the far left. \newline
* Right side: 2 blocks high at the far right. \newline
* \tann{annCol10}{Middle: 3 blocks high.}{Wrong Perception} \newline
* Wait, the top is 3 blocks wide. \newline
* \tann{annCol8}{Let's trace the outline again.}{Reiterating} \newline
* Top: 3 units wide. \newline
* Left side: 2 units down. \newline
* Bottom: 3 units wide, but with a cutout in the middle? No, it looks like it's 2 units wide, then a gap, then 2 units wide? No. \newline
* \tann{annCol8}{Let's look at the bottom edge of View 1}{Reiterating}: it goes from (0,2) to (1,2), then (1,3) to (2,3), then (2,3) to (3,3), then (3,3) to (3,2), then (3,2) to (4,2). No, that's not it. \newline
* Let's look at the bottom edge again: it's a "V" shape or a "U" shape? It looks like it goes down, then across, then up, then across, then down. \newline
* Actually, looking at View 1, the bottom edge is:\tann{annCol0}{I have to give the solution based on the reasoning directly now.}{Budget Hit}
\end{tcolorbox}
\begin{tcolorbox}[breakable,enhanced,colback=red!4,colframe=red!55!black,boxrule=0.4pt,arc=1pt,left=4pt,right=4pt,top=3pt,bottom=3pt,fonttitle=\footnotesize\bfseries,coltitle=black,colbacktitle=red!12,title={\tpicon{grok_icon.png}~Grok-4.20\hfill answer: False\tickno}]
\footnotesize\raggedright
The problem asks to determine if the object's silhouette is symmetric. I need to look at the two images and figure out if the silhouette from either view is symmetric. \newline
I need to determine if the object's silhouette is symmetric based on the two given images of the same 3D block-based object from different angles. The silhouette refers to the \begin{CJK*}{UTF8}{gbsn}\colorbox{annCol6}{折线}\textsuperscript{\tiny[Misc]}\end{CJK*} 
% \tann{annCol6}{折线}{Misc} 
2D outline as seen from each view, and I have to check if it's symmetric---likely along a vertical, horizontal, or otheraxis, where for every part, there's a mirrored counterpart.

The instructions suggest checking if either silhouette from the two views exhibits symmetry, and the output is a simple boolean: true if symmetric, false otherwise. The question says "the object's silhouette," singular, but mentions analyzing both views, so probably if the object has asymmetric silhouette in at least one perspective.

From analyzing the images, the first one appears irregular, like an L-shape with uneven steps, not symmetric in any obvious way. The second image also looks asymmetric, with uneven distributions of blocks, but I couldn't find a clear mirror line in either.

\tann{annCol10}{After careful consideration, considering theblock placements and outlines, neither silhouette seems to exhibit clear-cut symmetry, so the answer is false.}{Wrong Perception}
\end{tcolorbox}
\begin{tcolorbox}[breakable,enhanced,colback=red!4,colframe=red!55!black,boxrule=0.4pt,arc=1pt,left=4pt,right=4pt,top=3pt,bottom=3pt,fonttitle=\footnotesize\bfseries,coltitle=black,colbacktitle=red!12,title={\tpicon{gpt_icon.png}~GPT-5\hfill answer: False\tickno}]
\footnotesize\raggedright
``` \newline
\{ \newline
\tann{annCol10}{'answer': False,}{Wrong Perception} \newline
\} \newline
```
\end{tcolorbox}
\begin{tcolorbox}[breakable,enhanced,colback=red!4,colframe=red!55!black,boxrule=0.4pt,arc=1pt,left=4pt,right=4pt,top=3pt,bottom=3pt,fonttitle=\footnotesize\bfseries,coltitle=black,colbacktitle=red!12,title={\tpicon{gemini_flash_icon.png}~Gemini-3-Flash\hfill answer: False\tickno}]
\footnotesize\raggedright
To determine whether the object's silhouette is symmetric, let's break down the block arrangement from the given viewpoints:

1. **Analyze the 3D grid layout:** The object is arranged on a 3D grid of blocks. Let's look at the columns from left to right along the front-facing edges in both views. \newline
* In **View 1**, the leftmost column has a height of 2 blocks. \tann{annCol10}{The next column to its right drops down at the bottom but rises to form a 2-block height.}{Wrong Perception} The rightmost visible sections show an asymmetrical distribution of single and double-height columns, including a single protruding block on the far right. \newline
* In **View 2**, which looks at the object from a different angle, we can see the opposite side or a rotated perspective. The bottom and top boundaries form a staggered, stepped pattern that is distinctly uneven.

2. **Evaluate the Silhouette Symmetry:** \newline
\tann{annCol10}{* **Vertical Symmetry:** If you draw a vertical line down the middle of either 2D outline, the left side does not mirror the right side due to the stepped, asymmetrical arrangement of the columns and the protruding single blocks on the ends. * **Horizontal Symmetry:** If you draw a horizontal line through the center, the top boundary (which is flat or lightly stepped in some rows) does not mirror the bottom boundary (which has deep cutouts and staggered drops). }{Wrong Perception}

Because the outer boundaries of the 2D shapes projected from these viewpoints do not possess vertical or horizontal mirror symmetry, the answer is false.

```json \newline
\{ \newline
'answer': False, \newline
\}

```
\end{tcolorbox}
\begin{tcolorbox}[breakable,enhanced,colback=red!4,colframe=red!55!black,boxrule=0.4pt,arc=1pt,left=4pt,right=4pt,top=3pt,bottom=3pt,fonttitle=\footnotesize\bfseries,coltitle=black,colbacktitle=red!12,title={\tpicon{gemini_pro_icon.png}~Gemini-3.1-Pro\hfill answer: False\tickno}]
\footnotesize\raggedright
Analyzing Object Symmetry

I've begun analyzing the object's outline in the first image, hypothesizing a bounding box.

Defining the Coordinate System

I've established a 2D silhouette focus, with initial coordinates and identified key axes for this shape.

Visualizing Structure Elements

I've determined a 2x3 grid structure, identifying visible faces and column heights with initial coordinate labeling.

\textit{[[...trimmed output...]]}

% Refining Face Orientation

% I've clarified the isometric grid's axes, ensuring accurate face direction interpretations for the images.

% Mapping Column Relationships

% I've traced grid columns, establishing face directions and relative coordinates within the isometric plane with increasing accuracy.

% Mapping Top Faces

% I've precisely identified a 2x3 grid of top faces within the image's coordinate system, resolving initial ambiguities.

% Clarifying Top Face Structure

% I've precisely mapped the top face arrangement as a 2x2 grid with an additional face on the right edge.

% Tracing Boundary Elements

% The top boundary now precisely reflects image one, incorporating steps and corners around the right-most face's unique position.

% Tracing Object Boundary

% I have successfully traced the complete silhouette boundary of the object in Image 1 by verifying each segment's position.

% Revising Coordinate System

% I've reoriented the axes to a left-handed system, aligning with isometric views, establishing clear face visibility.

% Determining Relative Positions

% I've just accurately deduced that there's a column at (1,1) in the isometric projection based on visual cues.

% Verifying Block Placement

% I've just confirmed the presence of blocks at (0,0,2), (0,1,2), (1,0,2), and (1,1,2) in isometric view.

% Defining Isometric Projection

% I've just derived the 2D isometric projection matrix, now accurately mapping 3D cube vertices.

% Mapping Block Dimensions

% I've just precisely identified a 3x2 grid for the top faces, resolving the blocks' layout.

% Confirming Face Orientations

% I've just validated a 3x2 grid structure, defining coordinates and verifying all face orientations.

% Verifying Structure Absence

% I just confirmed the missing (2,1) column, adjusting the top face and establishing the object's boundary.

% Tracing Image Edges

% I am now meticulously tracing Image 1's silhouette, calculating 2D coordinates starting from the bottom-most point.

% Tracing Top Silhouette

% I am now tracing the silhouette, confirming its path from (-2,3.0) to (0,4.0), then down-right.

% Revising Face Positioning

% I've just reconsidered the top-most point and re-examined Image 1, now accurately mapping the 5 faces' relative positions.

% Verifying Surface Absence

% I just confirmed the absence of a face at (2,0) by meticulously analyzing the two-segment top boundary.

% Verifying Peak Placement

% I've just validated the peak positions, confirming the top faces' zig-zag, with faces like (1,1) precisely accounted for.

% Calculating Block Heights

% I've just determined (0,0),(1,0),(2,0),(0,1) all have height two, visualizing the blocks and faces.

% Confirming Vertical Line

% The recent analysis validated the lack of the (2,1) block via a vertical line and vertex at height one in Image 1.

% Mapping Column Configuration

% I've just confirmed the block arrangement using Image 1, defining a consistent object structure.

% Confirming Shape Configuration

% I've just determined a 3x2 grid missing the front corner, precisely matching the blocks in Image 2.

% Revising Object Structure

% I've just recognized that the "missing" block is only one block high, resolving the discrepancy with Image 2.

% Tracing Left Faces

% I've just confirmed the left boundary in Image 2 confirms (0,0) height one, with (1,0) having height two.

% Analyzing Column Alignment

% I've just determined that a vertical line indicates a shift in the y-direction, thus resolving the grid structure.

% Verifying Cube Heights

% I just confirmed the front-most column's height in Image 2 is two, correcting the misinterpretation of its faces.

% Verifying Face Visibility

% I've just confirmed all six top faces are visible in Image 2, forming a full 3x2 grid, precisely matching expectations.

% Revising Peak Alignment

% I've just recognized that the "valley" is not a missing block, but a hidden inner edge, confirming a full top 3x2 rectangle.

% Confirming Image Similarity

% The recent analysis validated the missing block at (2,1), rotating and verifying it's missing in Image 2.

% Validating Structure Features

% I've just determined all six top faces are present in Image 2, resolving previous inconsistencies, it is a 3x2x2 block!

% Tracing Column Shifts

% I've just determined the next column's shift, confirming a vertical edge and shift to (1,1) in Image 2.

% Verifying Grid Orientation

% I've just determined the y-axis spans three columns, with the middle shifted, resolving the step in Image 2.

% Mapping Face Dimensions

% I've just determined the left faces, revealing a 2x2 rectangle and shifted 1x2 column.

% Confirming Surface Count

% I've just validated a 2x3 block grid (missing corner) across both images, confirming five blocks.

% Analyzing Silhouette Symmetry

% I've just confirmed the symmetry of the view 1 silhouette's top boundary, validating its shape's reflection around x=1.

% Verifying Image Asymmetry

% The current analysis confirms both silhouettes are asymmetric, having identified all 2D vertex coordinates in the process.

% Tracing Left Face

% I've just confirmed the left boundary in both images; it's a straight line from (-2,1) to (-2,4).

% Assessing Silhouette Symmetry

% I've just concluded neither silhouette is symmetric due to the distinct top peak in each image.

% Revising Peak Verification

% I've just validated a missing corner and two shifted steps, concluding Image 1 is not symmetrical.

% Reassessing Edge Symmetry

% I've just confirmed the silhouettes' asymmetry by precisely calculating unequal base segment counts in Image 1.

% Confirming Non-Symmetry

% The current analysis emphatically confirms both Image 1 and 2 lack symmetry, ruling out any hidden interpretations.

% Confirming Silhouettes Asymmetry

% I've determined both silhouettes' distinct heights and edge configurations emphatically confirm their asymmetry, answering the initial question.

% Assessing Symmetric Properties

% I've just determined Image 1 is asymmetric, clarifying prior ambiguities with precise edge position verification.

Verifying Image Asymmetry

I have decisively validated the asymmetry of both images by analyzing top face arrangements and edge segment counts.

Verifying Isometric Symmetry

\tann{annCol10}{I've just determined a 3x2x2 block projected isometrically cannot be symmetric, even without missing blocks.}{Wrong Perception}

```json \newline
\{ \newline
"answer": false \newline
\}

```
\end{tcolorbox}

\subsubsection{T9 Visible Floors}
\begin{table}[H]
\centering
\footnotesize
\setlength{\tabcolsep}{1pt}
\renewcommand{\arraystretch}{1.2}
\begin{tabular}{*{9}{>{\centering\arraybackslash}p{\dimexpr\textwidth/9-2\tabcolsep\relax}}}
\toprule
\multicolumn{9}{@{}l@{}}{\itshape ``\ldots{}Your task is to count the number of visible layers (floors/horizontal levels) in the object\ldots{}''}\\[0.3mm]
\multicolumn{9}{@{}c@{}}{\begin{tabular}{*{2}{c}}\includegraphics[width=0.450\textwidth,height=1.25in,keepaspectratio]{images/app_qual_traces/T9_sample3_row93_query_image_1.png} & \includegraphics[width=0.450\textwidth,height=1.25in,keepaspectratio]{images/app_qual_traces/T9_sample3_row93_query_image_2.png}\end{tabular}}\\[0.5mm]
\textbf{GT} & \tpicon{qwen_icon.png} & \tpicon{gemma_icon.png} & \tpicon{glmv_icon.png} & \tpicon{kimi_icon.png} & \tpicon{grok_icon.png} & \tpicon{gpt_icon.png} & \tpicon{gemini_flash_icon.png} & \tpicon{gemini_pro_icon.png}\\
3 & 4\tickno & 5\tickno & 4\tickno & 6\tickno & 4\tickno & 6\tickno & 4\tickno & 3\tickok\\
\bottomrule
\end{tabular}
\caption{T9 Visible Floors.}
\label{tab:qual_trace_t9}
\end{table}
\noindent\textbf{Thinking traces.}\par\smallskip
\begin{tcolorbox}[breakable,enhanced,colback=red!4,colframe=red!55!black,boxrule=0.4pt,arc=1pt,left=4pt,right=4pt,top=3pt,bottom=3pt,fonttitle=\footnotesize\bfseries,coltitle=black,colbacktitle=red!12,title={\tpicon{glmv_icon.png}~GLM-4.6V-Flash\hfill answer: 4\tickno}]
\footnotesize\raggedright
Got it, let's try to figure out the number of visible layers. First, I need to look at both images and identify the vertical layers.

\textit{[[...trimmed output...]]}

% In the first image, let's see the blocks. Let's think about the height (vertical layers). Let's check each layer:

% - The bottommost layer: Are there blocks at the lowest level? Looking at the first image, there's a block at the bottom left, then adjacent blocks. Then the next layer up. Let's count the vertical stacks.

% Wait, layers are horizontal levels, so each layer is a horizontal plane. So we need to find how many different heights there are.

% Looking at the first image: Let's identify the vertical positions. Let's see the blocks:

% In the first image, there's a vertical stack on the right side (the tall column). Let's check the height of that column. How many blocks are stacked vertically there? Let's see: In the first image, the rightmost column has blocks from bottom to top. Let's count the layers:

% First image: Let's see the bottom layer (lowest Z). Then the next layer above it, etc.

% Alternatively, look at the second image. In the second image, there's a vertical stack on the left side. Let's count the layers there.

Let's analyze each image's vertical layers:

First image:

- Bottom layer (lowest height): There's a block at the bottom left, and adjacent blocks. Let's see the vertical stack on the right side: how many blocks? Let's count the columns. \tann{annCol10}{The rightmost column has 4 blocks?}{Wrong Perception} \tann{annCol8}{Wait, no. Let's look at the first image's structure. Wait, maybe better to count the maximum height in each view. }{Reiterating} \newline
In the first image, the tallest part: The vertical stack on the right (the column going up) has how many blocks? Let's see: The rightmost column has blocks from bottom to top: let's count the rows. \tann{annCol10}{The bottom row (layer 1) has some blocks, then layer 2, layer 3, layer 4?}{Wrong Perception} \tann{annCol8}{Wait, no. Wait, let's think of layers as horizontal levels.}{Reiterating} So each layer is a horizontal slice. So if we have blocks at different heights, each distinct height is a layer.

Let's look at the first image:

- Layer 1 (bottom): The lowest blocks. For example, the bottom-left block, and the adjacent ones. Then layer 2 above that. Let's see the vertical stack on the right: how many blocks stacked vertically? Let's count the number of blocks in the rightmost column. \tann{annCol10}{In the first image, the rightmost column has 4 blocks?}{Wrong Perception} \tann{annCol8}{Wait, no. Let's look at the first image's right side: there's a column with 4 blocks? Or maybe 3? Wait, no. Wait, let's look at the second image.}{Reiterating} In the second image, the leftmost column has blocks stacked vertically. Let's count the layers there. \tann{annCol10}{The leftmost column in the second image has 4 blocks? Let's see: the leftmost column has blocks from bottom to top: 4 blocks? So that would be 4 layers?}{Wrong Perception} But wait, maybe some layers are shared.

\tann{annCol8}{Wait, let's check both images for the number of vertical layers. }{Reiterating} \newline
First image:

- The bottom layer (lowest height) has blocks. Then the next layer up (middle bottom), then next, then top. Let's count the vertical stacks.

\tann{annCol10}{In the first image, the rightmost column (the tall one) has 4 blocks? Let's see: the bottom block of that column, then above it, etc. So that's 4 layers?}{Wrong Perception} \tann{annCol8}{But wait, maybe the topmost block is a separate layer. Wait, no.}{Reiterating} \tann{annCol10}{Let's think of each layer as a horizontal level. So if there's a block at height 1, 2, 3, 4, then there are 4 layers.}{Wrong Perception}

\tann{annCol8}{But let's check the second image.}{Reiterating} I\tann{annCol10}{n the second image, the leftmost column has 4 blocks? Let's see: the leftmost column in the second image has blocks stacked vertically: 4 blocks. So that's 4 layers.}{Wrong Perception}

\tann{annCol8}{Wait, but let's confirm.}{Reiterating} \tann{annCol10}{Let's look at the first image again. The topmost block is a single block on top of the left stack. So that's a layer with 1 block. Then the next layer down has 2 blocks, etc. Wait, maybe the number of layers is 4.}{Wrong Perception} \tann{annCol8}{Let's check both images.}{Reiterating}

\tann{annCol10}{In the first image, the vertical stack on the right has 4 blocks (from bottom to top). So that's 4 layers.}{Wrong Perception} The left stack has 3 blocks? No, wait.

\tann{annCol8}{Alternatively, let's count the distinct vertical levels. Let's see: }{Reiterating} \newline
- Layer 1: bottommost blocks (lowest height) \newline
- Layer 2: next level up \newline
- \tann{annCol10}{Layer 3: next - Layer 4: topmost}{Wrong Perception}

\tann{annCol10}{So that's 4 layers.}{Wrong Perception} Let\tann{annCol0}{I have to give the solution based on the reasoning directly now.}{Budget Hit}
\end{tcolorbox}
\begin{tcolorbox}[breakable,enhanced,colback=red!4,colframe=red!55!black,boxrule=0.4pt,arc=1pt,left=4pt,right=4pt,top=3pt,bottom=3pt,fonttitle=\footnotesize\bfseries,coltitle=black,colbacktitle=red!12,title={\tpicon{grok_icon.png}~Grok-4.20\hfill answer: 4\tickno}]
\footnotesize\raggedright
The problem asks to count the number of visible layers (floors) in the object made of blocks. I have two perspective images from different angles. \newline
I need to count the number of visible layers in this blocky 3D object from two perspective views. The object is made of unit blocks, and a layer is a horizontal row at the same height. I figure a visible layer is any height level with at least one block, so I'm counting the distinct Z-coordinates occupied by blocks.

To do this, I reconstruct the 3D structure mentally from the images. \tann{annCol2}{The first image looks like a compact shape with maybe 3 or 4 levels.}{Good Intuition} T\tann{annCol10}{he second image seems taller, with a stack reaching up to 4 blocks high in one spot.}{Wrong Perception}

\tann{annCol10}{I cross-check between views toensure consistency. In the second view, there's a clear stack of 4 blocks vertically aligned, suggesting at least blocks vertically aligned, suggesting at least 4 layers.}{Wrong Perception} But I need the total number of layers across the whole object.

\tann{annCol10}{Upon closer inspection, blocks span from the lowest point to the highest, with gaps filledin mentally. The object seems to have blocks at heights 0,1,2,3, and possibly 4. In the first view, the tallest stack is 4 blocks, and the second confirms it. No higher stacks, and no indication of only 3. So, there are 4 distinct layers.}{Wrong Perception}

\{ \newline
'answer': 4, \newline
\}

\tann{annCol7}{That seems consistent with the example}{Prior Bias} and my reasoning.I think that's it.
\end{tcolorbox}
\begin{tcolorbox}[breakable,enhanced,colback=red!4,colframe=red!55!black,boxrule=0.4pt,arc=1pt,left=4pt,right=4pt,top=3pt,bottom=3pt,fonttitle=\footnotesize\bfseries,coltitle=black,colbacktitle=red!12,title={\tpicon{gpt_icon.png}~GPT-5\hfill answer: 6\tickno}]
\footnotesize\raggedright
Visualizing and reasoning about cube structures \newline
I'm analyzing the image's structure. \tann{annCol3}{The bottom front-left cube is 3 cubes high,}{Good Perception} with noticeable horizontal lines at y249 and y301. \tann{annCol10}{The right-front column might also be 3 cubes high, with a slant at the top.}{Wrong Perception} Above, there's a row of blocks that seems to have a "neck" structure extending upward. \newline
Identifying grid structure of the object in image \newline
I'm analyzing the top cluster of the object. The topmost face seems to be the highest cube, and the right vertical face might represent the top cube. The left side has slanted vertical edges suggesting a height of three stacked cubes, each layer at different z-levels, \tann{annCol10}{possibly forming a stack of 6 cubes overall.}{Wrong Perception} \newline
Determining the number of visible floors \newline
The image suggests there are 3 layers in the bottom cluster and the top cluster is above, possibly connected by a vertical column. I'll try to count the visible layers based on the height, considering that there might be gaps. \tann{annCol10}{The maximum stack height seems to be around 5 cubes, so I think that's the number of visible floors.}{Wrong Perception} \newline
Analyzed image \newline
Output image \newline
Analyzed image \newline
Output image \newline
Counting visible layers in the object \newline
I'm thinking through how to count the object's floors based on the distinct z-coordinate levels. Since this is in an isometric perspective, the highest and lowest layers are key. I'll take horizontal slices at different y-values, from y353 to y51, noting the separators. \tann{annCol10}{It looks like there are maybe 6 layers. }{Wrong Perception} \newline
``` \newline
\{ \newline
'answer': 6, \newline
\} \newline
```
\end{tcolorbox}
\begin{tcolorbox}[breakable,enhanced,colback=red!4,colframe=red!55!black,boxrule=0.4pt,arc=1pt,left=4pt,right=4pt,top=3pt,bottom=3pt,fonttitle=\footnotesize\bfseries,coltitle=black,colbacktitle=red!12,title={\tpicon{gemini_flash_icon.png}~Gemini-3-Flash\hfill answer: 4\tickno}]
\footnotesize\raggedright
To find the number of distinct vertical layers (floors) in the 3D object, let's analyze its height structure by looking at the steps/levels visible across both perspectives.

1. **Top Layer:** There is a distinct highest layer containing a couple of blocks (seen clearly at the very top of both images). \newline
2. **Second Layer:** Directly beneath the top blocks, there is a second level of blocks. \newline
3. **Third Layer:** Stepping down further, we can see a third distinct level of blocks. \newline
4. \tann{annCol10}{**Bottom Layer:** At the very base, there are blocks forming the foundational layer resting underneath the others.}{Wrong Perception}

\tann{annCol10}{Counting these vertical steps from the lowest to the highest level gives us a total of 4 distinct floors.}{Wrong Perception}

```json \newline
\{ \newline
'answer': 4 \newline
\}

```
\end{tcolorbox}
\begin{tcolorbox}[breakable,enhanced,colback=green!4,colframe=green!50!black,boxrule=0.4pt,arc=1pt,left=4pt,right=4pt,top=3pt,bottom=3pt,fonttitle=\footnotesize\bfseries,coltitle=black,colbacktitle=green!14,title={\tpicon{gemini_pro_icon.png}~Gemini-3.1-Pro\hfill answer: 3\tickok}]
\footnotesize\raggedright
Assessing Visible Layers

I've begun analyzing the first image, focusing on vertical stacks to assess the structure's height.

Defining Layer Heights

I've determined distinct horizontal layers by identifying visible top faces, assigning Z values to each level observed.

Mapping Spatial Coordinates

I'm now establishing a coordinate system, designating a corner as (0,0,0) and focusing on Image 2 for clearer vertical stack identification.

Re-evaluating Block Geometry

I'm now re-assessing block counts, considering visibility from different angles to determine precise spatial relationships.

Confirming Stack Height \newline
\tann{annCol10}{ I've confirmed the leftmost stack in Image 2 is four blocks high, cross-referencing to Image 1's stack.}{Wrong Perception}

Confirming Block Count

I'm now methodically verifying the block count, focusing on Image 2, resolving ambiguities by examining the visible faces.

\textit{[[...trimmed output...]]}

% Analyzing Block Structures

% I've counted horizontal edges and now visualizing block layering, hypothesizing a staircase arrangement in both images.

% Modeling Block Relationships

% I've established a coordinate system and constructed a staircase model, now matching the visuals in Image 1.

% Refining Vertical Analysis

% I'm now carefully re-evaluating block heights, refining the structure's vertical dimension based on horizontal planes observed.

% Re-Counting Block Faces

% I'm now meticulously recounting block faces in both images to resolve height discrepancies, comparing vertical edges.

% Clarifying Spatial Structures

% I've re-examined Image 2, defining the top horizontal shape as an L with three blocks, clarifying vertical and horizontal relationships.

% Correlating Layer Surfaces

% I'm now identifying corresponding top faces across both images, verifying height assignments using spatial relationships.

% Verifying Horizontal Shapes

% I've determined both images share a consistent 1x2 bar arrangement, solidifying layer-by-layer 3D model construction.

% Defining Coordinate System

% I've re-evaluated coordinates, now hypothesizing an L-shaped base structure in Image 1.

% Verifying Image Correspondence

% I've confirmed Image 2's viewpoint, matching its structure to Image 1's back-right column and coordinates.

Verifying Vertical Segments

\tann{annCol3}{I've determined three visible layers by carefully counting the line segments and confirming block connections.}{Good Perception}

Finalizing Block Count

\tann{annCol3}{I've confirmed the block count through meticulous re-evaluation, generating the final JSON: \{ "answer": 3 \}.}{Good Perception}

```json \newline
\{ \newline
"answer": 3 \newline
\}

```
\end{tcolorbox}

\subsubsection{T10 Color Connected}
\begin{table}[H]
\centering
\footnotesize
\setlength{\tabcolsep}{1pt}
\renewcommand{\arraystretch}{1.2}
\begin{tabular}{*{9}{>{\centering\arraybackslash}p{\dimexpr\textwidth/9-2\tabcolsep\relax}}}
\toprule
\multicolumn{9}{@{}l@{}}{\itshape ``\ldots{}Your task is to determine whether there exists at least one pair of adjacent blocks (sharing a face) that share the same color\ldots{}''}\\[0.3mm]
\multicolumn{9}{@{}c@{}}{\begin{tabular}{*{2}{c}}\includegraphics[width=0.450\textwidth,height=1.25in,keepaspectratio]{images/app_qual_traces/T10_sample1_row51_query_image_1.png} & \includegraphics[width=0.450\textwidth,height=1.25in,keepaspectratio]{images/app_qual_traces/T10_sample1_row51_query_image_2.png}\end{tabular}}\\[0.5mm]
\textbf{GT} & \tpicon{qwen_icon.png} & \tpicon{gemma_icon.png} & \tpicon{glmv_icon.png} & \tpicon{kimi_icon.png} & \tpicon{grok_icon.png} & \tpicon{gpt_icon.png} & \tpicon{gemini_flash_icon.png} & \tpicon{gemini_pro_icon.png}\\
False & True\tickno & False\tickok & True\tickno & True\tickno & False\tickok & True\tickno & False\tickok & False\tickok\\
\bottomrule
\end{tabular}
\caption{T10 Color Connected.}
\label{tab:qual_trace_t10}
\end{table}
\noindent\textbf{Thinking traces.}\par\smallskip
\begin{tcolorbox}[breakable,enhanced,colback=green!4,colframe=green!50!black,boxrule=0.4pt,arc=1pt,left=4pt,right=4pt,top=3pt,bottom=3pt,fonttitle=\footnotesize\bfseries,coltitle=black,colbacktitle=green!14,title={\tpicon{gemma_icon.png}~Gemma4-31B\hfill answer: False\tickok}]
\footnotesize\raggedright
* The object is composed of colored blocks. \newline
* Two views are provided. \newline
* Goal: Determine if any two adjacent blocks (sharing a face) have the same color. \newline
* Colors: yellow, cyan, green, magenta, red, orange, orchid, teal, slategray, gold, blue, purple.

* View 1: \newline
* Top row (from left to right): Yellow, Green, Teal, Green. \newline
* \tann{annCol10}{Middle row (from left to right): Yellow, Green, Slategray, Yellow.}{Wrong Perception} \newline
* Bottom row (from left to right): (empty), (empty), Blue, Purple. \newline
* \tann{annCol8}{Wait, let's re-examine View 1.}{Reiterating} \newline
* Top layer: \newline
* (0, 0, 0): Yellow (top face), Yellow (front face) \newline
* (1, 0, 0): Green (top face), Green (front face) \newline
* (2, 0, 0): Teal (top face), Slategray (front face) \newline
* (3, 0, 0): Green (top face), Yellow (front face) \newline
* \tann{annCol8}{Wait, the blocks are 3D.}{Reiterating} Let's use (x, y, z) coordinates. \newline
* Let's assume the top row in View 1 is z=1, the middle row is z=0, and the bottom row is z=-1. \newline
* \tann{annCol8}{Wait, the image is a perspective view.}{Reiterating} \newline
\textit{[[...trimmed output...]]} \newline
% * View 1: \newline
% * Top row (z=1): \newline
% * (0, 1, 0): Yellow (top), Yellow (front) \newline
% * (1, 1, 0): Green (top), Green (front) \newline
% * (2, 1, 0): Teal (top), Slategray (front) \newline
% * (3, 1, 0): Green (top), Yellow (front) \newline
% * Wait, the "middle row" is actually the front faces of the top row. \newline
* \tann{annCol8}{Let's re-examine View 1.}{Reiterating} \newline
\textit{[[...trimmed output...]]} \newline
% * It looks like a 4x2 grid of blocks on top, and some blocks below. \newline
% * Top layer (z=1): \newline
% * (0, 1, 0): Yellow \newline
% * (1, 1, 0): Green \newline
% * (2, 1, 0): Teal \newline
% * (3, 1, 0): Green \newline
* \tann{annCol8}{Wait, the front faces of these blocks are:}{Reiterating} \newline
\textit{[[...trimmed output...]]} \newline
% * (0, 1, 0): Yellow \newline
% * (1, 1, 0): Green \newline
% * (2, 1, 0): Slategray \newline
% * (3, 1, 0): Yellow \newline
% * Wait, that's not right. A block has one color. \newline
* \tann{annCol8}{Let's look at the blocks again.}{Reiterating} \newline
* Block 1: Top=Yellow, Front=Yellow. Color = Yellow. \newline
* Block 2: Top=Green, Front=Green. Color = Green. \newline
* \tann{annCol10}{Block 3: Top=Teal, Front=Slategray. Wait, this is impossible if each block has one color. * Let me re-read: "The object is composed of blocks with different colors." This usually means each block is a single color.}{Wrong Perception} \newline
* \tann{annCol8}{Let's re-examine the colors in View 1.}{Reiterating} \newline
\textit{[[...trimmed output...]]} \newline
% * Top row: \newline
% * Block (0, 1, 0): Top=Yellow, Front=Yellow. Color = Yellow. \newline
% * Block (1, 1, 0): Top=Green, Front=Green. Color = Green. \newline
% * Block (2, 1, 0): Top=Teal, Front=Slategray. Wait, the front face of the block at (2, 1, 0) is Slategray. The top face is Teal. \newline
% * Block (3, 1, 0): Top=Green, Front=Yellow. \newline
% * Wait, maybe the colors are on the *faces*? No, "composed of blocks with different colors" usually means the block itself has a color. \newline
* \tann{annCol8}{Let's look at View 2.}{Reiterating} \newline
\textit{[[...trimmed output...]]} \newline
% * View 2: \newline
% * Top row: Yellow, Slategray. \newline
% * Middle row: Green, Teal, Green, Yellow. \newline
% * Bottom row: Blue, Purple. \newline
% * Bottom-most row: Purple, Blue. \newline
* \tann{annCol8}{Let's re-examine View 1 and View 2 together.}{Reiterating} \newline
* View 1: \newline
* Top layer: (0,1,0)=Yellow, (1,1,0)=Green, (2,1,0)=Teal, (3,1,0)=Green. \newline
* Wait, the front faces are: (0,1,0)=Yellow, (\tann{annCol0}{I have to give the solution based on the reasoning directly now.}{Budget Hit}
\end{tcolorbox}
\begin{tcolorbox}[breakable,enhanced,colback=green!4,colframe=green!50!black,boxrule=0.4pt,arc=1pt,left=4pt,right=4pt,top=3pt,bottom=3pt,fonttitle=\footnotesize\bfseries,coltitle=black,colbacktitle=green!14,title={\tpicon{grok_icon.png}~Grok-4.20\hfill answer: False\tickok}]
\footnotesize\raggedright
The problem asks if there is at least one pair of adjacent blocks that share the same color in this 3D object made of colored blocks. \newline
I need to figure out if there's at least one pair of adjacent blocks of the same color in this 
\begin{CJK*}{UTF8}{gbsn}\colorbox{annCol6}{仔细}\textsuperscript{\tiny[Misc]}\end{CJK*}
% \tann{annCol6}{仔细}{Misc}
crafted 3D object, based on two perspective views.

First, I look at the colors involved: there are several like yellow, cyan, green, magenta, red, orange, orchid, teal, slategray, gold, blue, purple. But in the views, I see mostly yellow, green, teal or cyan, gray or slategray, and then in the other view, blue and purple or magenta.

\textit{[[...trimmed output...]]}

% To determine adjacency, I have to reconstruct the 3D structure mentally. The first view shows an L-shapeor some irregular form with blocks arranged in layers.

% In the first image, there's a row on top: yellow, green, teal, green. But the two greens are separated by the teal, so not adjacent. Then below the first few, there are more blocks like gray and yellow.

% Counting the blocks per color:greens appear multiple times, but are they touching?

% In the first view, the rightmost part has a protruding arm with gray, yellow, blue, purple downward. The greens are on the main body.

% In the second view, it looks like a more front-facing perspective, showing columns: a stack of three on theleft with colors shifting.

% Specifically, in the second view, I notice a column with repeated colors? For example, the middle section has two greens side by side.

% Looking closely, in the second image, below the top row, the row below has green directly next to another green.

% Yes, there's a green block,and right next to it, another green block sharing a side.

% That means there are two adjacent greens sharing a face.

Since this is visible in one view, and the object is the same, this adjacency should hold in 3D as well, and it should be confirmable in the other view if possible, butthe task is to find if there exists at least one such pair. \newline
\tann{annCol10}{ So, the answer is yes, there is such a pair.}{Wrong Perception}

But to be thorough, I need to make sure it's not an illusion from the perspective.

But since it's perspective images of blocks, if they appear adjacent in one view, they are adjacentin 3D.

Yes, and the greens are next to each other.

Also, there are two yellows on the left that look stacked or side by side.

The left part has a yellow on the bottom and a matching color on top, but if they are stacked, they are adjacent vertically.

\tann{annCol10}{Either way,there are adjacent same colors. So, the final answer is true.}{Wrong Perception}

But the internal reasoning mentions a 2-high yellow tower on the left, with two yellows stacked, which are adjacent.

Yes, that's a clear case.

Also, in the second view, there are alternating colors, but the first view has thestacked yellows.

And the second view confirms the structure.

So, I think the answer is yes.

\{ \newline
'answer': True, \newline
\}

\{ \newline
'answer': True, \newline
\}\tann{annCol8}{I think that's it. I think that's it. But to make it clean, I'll just output the format. But to make it clean, I'll just output the format. }{Reiterating}

\tann{annCol5}{No, the task is to summarize the thinking trace for the user query, but don't present it in the third person as thetrace of a separate entity. So, I need to turn the internal reasoning into a clean, natural final response for the end user. The user query is to summarize the thinking trace, but the main task is the block adjacency. The human message is: Summarize the thinking trace for the user query, but don't presentit in the third person as the trace of a separate entity. Then the [User's Question] is the problem about the images and adjacent blocks. Then [Internal Reasoning] is the long thinking about the colors and structure. So, my job is to summarize that internal reasoning into a clean natural response, speaking as firstperson, directly to the user.}{Harnessing}

The final output should be in the format:

\{ \newline
'answer': bool, \newline
\}

From the internal reasoning, it seems like in the first view, there might be stacked same colors like yellow on yellow and green on green, but in the second view, the stacks are mixed colors likeyellow on green on blue, so no same color adjacent in the stacks, and the side adjacencies are different colors.

\textit{[[...trimmed output...]]}

% The conclusion is that there are no same color adjacent blocks, because if there were, it would show in both views, but the second view shows no stacked same, and side ones are different.

% But the internal reasoning is trying to assign coordinates and check adjacencies.

% In the coordinate assignment, column at (0,0): height 3: z=0 blue, z=1 green, z= bolt2 yellow

% Column at (1,0): z=0 purple, z=1 teal,z=2 gray

% Then column at (0,1): z=0 blue or purple, z=1 purple, etc.

% Then the arm at (2,0): z=1 green, adjacent to teal at (1,0,1), which is teal, not same.

% Then at (3,0): z=1 yellow, adjacent to green at (2,0,1), yellow and green different.

% No other adjacencies same.

Then is there a green at (2,0,2)? But earlier I thought maybe, but the second view shows no block at height 2 on the arm,only at mid level.

And the greens in the first view at high level are not at same height.

\tann{annCol3}{So, the greens are at different heights or positions, separated by other colors. Therefore, no pair of adjacent blocks with the same color. So, the answer is false.}{Good Perception}

But the problem is to see if thereexists at least one pair.

And from my reconstruction, there isn't.

\textit{[[...trimmed output...]]}

% But let's see if there's a way to arrange it with same color adjacent.

% But the task is to determine if there is, based on the views.

% The instruction is to confirm if such a pair exists in the 3D structure.

% And since theviews are from different angles, I need to see if in 3D they touch.

% But in my analysis, they don't.

% For example, the multiple yellows: one on the top left, one on the side, they are not next to each other.

% Greens are separated.

% Blues in the second view aresingle.

% Purples single.

So, no adjacent same colors.

Hence, the answer is False.

\tann{annCol5}{But the internal reasoning had some confusion, but I think it's False. But the internal reasoning says "I think the answer is false", then later "perhaps the answer is True", but then concludes False. No, theinternal reasoning is truncated, but the core is that after reconstructing, no adjacent same colors.}{Harnessing}

So, my final answer is False.

But to be sure, let's see if there's any possibility.

The problem mentions "A same-color adjacency found in one view should be confirmed in the other when possible."

So, if inone view they look adjacent but in the other they don't, it might not be.

But in this case, no such pairs even in views.

In the first view, the two greens are not adjacent, separated by teal.

The yellows are not next to each other.

So, yes, no pair of adjacent samecolor blocks.

Therefore, the answer is False.

\{ \newline
'answer': False, \newline
\}

\{ \newline
'answer': False, \newline
\}I think that's it.

But the output format is to have only the JSON.

So, the final output should be the JSON object.

But the instruction is to turn the internal reasoning into a clean natural final response.

But for the user, the user asked to summarize the thinking trace, but the user queryis the problem about the images, but the human message is "Summarize the thinking trace for the user query, but don't present it in the third person as the trace of a separate entity."

So, the task is to summarize the internal reasoning as my first person thoughts.
\end{tcolorbox}
\begin{tcolorbox}[breakable,enhanced,colback=red!4,colframe=red!55!black,boxrule=0.4pt,arc=1pt,left=4pt,right=4pt,top=3pt,bottom=3pt,fonttitle=\footnotesize\bfseries,coltitle=black,colbacktitle=red!12,title={\tpicon{gpt_icon.png}~GPT-5\hfill answer: True\tickno}]
\footnotesize\raggedright
Analyzing adjacency of colored cubes \newline
I need to check if there are any adjacent cubes with the same color in this polycube. The cubes are colored yellow/gold, green, teal, slate gray, blue, and purple. I'll first inspect whether the yellow cubes are adjacent vertically or horizontally, especially focusing on whether they match in color. Let me carefully analyze the two perspectives. \newline
Interpreting cube faces in perspective \newline
\textit{[[...trimmed output...]]} \newline
% In image1, the leftmost cube shows a yellow vertical face with two apparent yellow squares. These are not separate blocks but two faces of the same block in a 3D arrangement. The top face is a parallelogram, and the bottom one is a quadrilateral, not indicating separate cubes adjacent to each other. \newline
% Identifying adjacent cubes in multiple views \newline
% In both images, the cubes have certain neighboring relationships. In image2, the green cubes are adjacent but separated by teal. In image1, several colors (yellow, green, slate gray) are aligned, and some faces are likely part of the same cube. I'll check for same-color adjacencies across these arrangements more carefully. \newline
% Clarifying adjacency within the same cube and between blocks \newline
% In these visualizations, I need to remember that adjacent colors can belong to the same cube, not separate blocks. For example, yellow faces on the top and front are part of one cube, not two blocks. I'm looking for true adjacent cubes that share the same color, with visible seams between them. \newline
% Analyzed image \newline
% Output image \newline
% Analyzed image \newline
% Output image \newline
% Inferring coordinate mapping and block adjacency \newline
% I'm working on interpreting the isometric rendering. In image1, the top row likely represents the x-axis, with each cube's top face having a distinct color. The front faces correspond to the z-axis. It looks like the teal and slategray cubes are separate blocks, as their top and front faces differ in color. \newline
% Distinguishing cubes based on face colors and edges \newline
% The top teal face and slategray front face likely belong to different blocks. The color difference suggests they're separate cubes with adjacent faces---top of one, front of another. The shading variations due to lighting should be ignored, but the color difference clearly indicates separate blocks in this case. \newline
% Considering cube stacking and face color assignment \newline
% The top teal and gray front faces could be from two vertically stacked cubes---one's top face at a higher position, and the other's vertical face in the foreground. Similarly, the green top and yellow front may belong to separate cubes. In typical block worlds, each cube usually has uniform colors on all visible faces, but shading variations might occur. \newline
% Evaluating possible color mapping for cubes \newline
% For a cube, the top and front faces typically share a common edge and should be the same color. In the case of the leftmost and second cubes, this holds true, but for the third cube, the top is teal and the front is gray. This could mean the top teal face belongs to a separate cube behind the gray one. \newline
% Interpreting cube structure and visibility \newline
% In a dense cube arrangement, the top face of a back cube could align over the front cube's vertical side without being the same cube. Since cubes at different z-levels can overlap, the top faces likely represent cube colors, while the visible faces below might belong to adjacent or occluded cubes. Checking for adjacent same-color cubes in each view can help clarify. \newline
% Exploring color adjacency in the images \newline
% In image1, I notice green top faces on the second and fourth cubes, and teal on the third, but they're not adjacent initially. The second green could be adjacent to the left or share a face with yellow or teal below. Image2 shows adjacent green blocks, possibly indicating a shared cube or adjacent green cube arrangements. I'll need to carefully examine the pairings for color adjacency to clarify. \newline
% Analyzing color adjacency through projections \newline
% In View1, the top row has yellow and green squares, while the front row also has yellow and green. The yellow top and front faces likely belong to the same cube but aren't adjacent. If they're separate cubes, vertically adjacent with the same color, they still wouldn't share a cube edge. I'll try to reconstruct this using 3D projections. \newline
% Considering cube adjacency and color appearance \newline
% If two same-colored cubes are adjacent, their shared internal face wouldn't show a line, but on an exterior, there might be a visible seam. The renderer could outline edges, in which case adjacent same-colored cubes would get a black line between them. I should only focus on predefined colors and avoid considering lighting or shading variations. \newline
% Breaking down cube arrangement and visible faces \newline
% The cubes aren't separate, but let's count the visible faces: 4 top, 4 front, 1 lower front, and 2 bottom front. Some faces belong to the same cube. In the image, the top polyline shows four top surfaces (yellow, green, teal, green). Beneath them, front faces follow a similar pattern, but the teal cube could be behind the gray one. \newline
Analyzing cube arrangement and projection \newline
\tann{annCol10}{The cubes form a 2x4 slab, with the back row [yellow, green, teal, green] and the front row [yellow, green, gray, yellow]}{Wrong Perception}. However, only the top face is visible for all cubes unless there's one above, and the front face is only visible for the frontmost in the front row. In an isometric projection, the tops of cubes in the back rows may overlap with the front ones. Defining the axes with x across the screen, y as depth, and z vertically helps clarify their placement. \newline
Interpreting shape and layout \newline
The object seems to be an L-shaped structure, consisting of a 2-wide vertical stack (a "leg") and a horizontal arm. In image2, the front-left column shows: green and teal vertical faces in the top row, blue and magenta in the middle, and purple and blue in the bottom row. The topmost cubes may have their top faces hidden behind, explaining inconsistencies in visible face colors. \newline
Understanding cube visibility in voxel render \newline
In a voxel render, each visible cube is painted with a single color. Adjacent visible faces with different colors must be separate cubes. In image2, the yellow top face above the green front face indicates that the yellow cube is placed above the green one, hiding its top face. The orange face of the yellow cube may block part of the green face.

``` \newline
\{ \newline
\tann{annCol10}{'answer': True,}{Wrong Perception} \newline
\} \newline
```
\end{tcolorbox}
\begin{tcolorbox}[breakable,enhanced,colback=green!4,colframe=green!50!black,boxrule=0.4pt,arc=1pt,left=4pt,right=4pt,top=3pt,bottom=3pt,fonttitle=\footnotesize\bfseries,coltitle=black,colbacktitle=green!14,title={\tpicon{gemini_flash_icon.png}~Gemini-3-Flash\hfill answer: False\tickok}]
\footnotesize\raggedright
To determine whether there is at least one pair of adjacent blocks (sharing a face) that have the same color, let's analyze the 3D structure and the layout of the colored blocks by comparing both views.

\#\#\# 1. Structure Analysis

The object forms a 3D configuration of interconnected blocks:

* There is a prominent 4-block horizontal arm. Looking at **Image 1**, from left to right, this top-front layer consists of: **Yellow \$\textbackslash\{\}rightarrow\$ Green \$\textbackslash\{\}rightarrow\$ Teal \$\textbackslash\{\}rightarrow\$ Green**. \newline
* In **Image 1**, a **Grey (Slategray)** block is attached to the front of the Teal block. To the right of this Grey block is another **Yellow** block (sitting in front of the rightmost Green block). \newline
* Below the Grey block is a **Blue** block, and to its right (below the front Yellow block) is a **Purple (Magenta)** block. \newline
* Looking at the side/back columns, we can see additional vertical extension blocks (Blue and Purple stacked at the back right edge).

\#\#\# 2. Adjacency and Color Check

\tann{annCol8}{Let's look closely at the horizontal row in **Image 1**:}{Reiterating}

* The leftmost block is **Yellow**. \newline
* Directly adjacent to its right face is a **Green** block. \newline
* Adjacent to that Green block's right face is a **Teal** block. \newline
* Adjacent to that Teal block's right face is another **Green** block.

Even though there are two Green blocks and two Yellow blocks in the structure, they do not share a face:

* The two **Green** blocks are separated by a **Teal** block. \newline
* The two **Yellow** blocks are separated diagonally or by other blocks (one is at the far left of the main row, the other is on the front-right layer). \newline
* The **Blue** and **Purple** blocks alternate or sit adjacent to different colored blocks (e.g., Blue is under Grey; Purple is under Yellow).

\tann{annCol3}{Checking every single face connection across the entire reconstructed 3D grid reveals that every block is exclusively adjacent to blocks of a *different* color. There are no two blocks of the same color sharing a face.}{Good Perception}

```json \newline
\{ \newline
"answer": false \newline
\}

```
\end{tcolorbox}
\begin{tcolorbox}[breakable,enhanced,colback=green!4,colframe=green!50!black,boxrule=0.4pt,arc=1pt,left=4pt,right=4pt,top=3pt,bottom=3pt,fonttitle=\footnotesize\bfseries,coltitle=black,colbacktitle=green!14,title={\tpicon{gemini_pro_icon.png}~Gemini-3.1-Pro\hfill answer: False\tickok}]
\footnotesize\raggedright
Assessing the Task

I've defined the core problem: identifying adjacent, same-colored blocks from 2D projections into a JSON boolean, starting from image one.

Mapping the Geometry

I've established a coordinate system and mapped blocks, confirming they align with the image's layout.

\textit{[[...trimmed output...]]}

% Clarifying Image Data

% I have deduced the color mapping in Image 1 and started comparing colors with Image 2's structure.

% Revisiting Coordinate Assumptions

% I've re-evaluated coordinates, determining (x,y,z) with y as vertical best represents image data.

% Confirming Perspective Alignment

% I've verified the coordinate system's alignment from a negative z-axis perspective in Image 2.

% I can confirm x and z axis match, now checking other blocks' relation and z-axis depth.

% Analyzing Color Placement

% I've determined that blocks exhibit solid colors, contradicting Image 2's structure's assumptions.

% Validating Rotational Hypothesis

% I've tested a 90-degree rotation hypothesis for Image 2 and confirmed its excellent fit with Image 1's data.

% Visualizing from New Angles

% I've tested camera perspectives, confirming block visibility from Image 2's viewing angle.

% I've tested camera perspectives, confirming block visibility from Image 2's viewing angle.

% Defining Coordinate System

% I've established a standard isometric coordinate system to map colors and block positions effectively.

% Verifying Block Placement

% I've mapped colors to coordinates in Image 1 and started projecting Image 2, determining its viewing angle.

% Verifying Block Placement

% I've precisely matched image data's back row to establish the Image 2 perspective at (-x, -z) viewpoint.

% Refining Layer Hypothesis

% I've tested 3-block stacks, using Image 1's right edge for color confirmation and now verifying the flat top layer.

% Revising Block Relations

% I've re-examined Image 2 to conclude the purple and blue faces belong to separate blocks based on perspective.

% Verifying Arm Block Mapping

% I've accurately mapped the horizontal arm's blocks to the coordinate system, confirming all faces align perfectly.

% Validating Block Colors

% I've confirmed the initial block color assignments; I've found discrepancies and revised assumptions about block solidity.

% Revising Color Mapping

% I've re-examined color placement considering Image 2's perspective to determine block coloring at each coordinate.

% Verifying Axis Orientation

% I've precisely confirmed how both images use coordinate axes, especially from Image 2's negative perspective.

% Revising Axis Directions

% I've re-evaluated axis directions, now confirming Image 1 aligns to +x, contradicting Image 2's structure.

% Mapping Block Arrangement

% I've precisely matched colors in Image 1 and determined their L-shape or T-shape arrangement.

% Verifying Layer Placement

% I'm now determining colors in the bottom plan view, using Images 1/2's arrangement as a guide.

% Verifying Top-Right Perspective

% I've confirmed the (+x, -z) camera view matches both images' block arrangements with precise color verification.

% Confirming Image Perspective

% I've precisely matched image data, concluding Image 2's left-facing side is the +x face with complete confidence now.

% Analyzing Color Sequences

% I've re-established Image 2's colors, determining the top layer sequence: Yellow, Green, Teal, Green, and Yellow.

% Revising Image Views

% I've tested viewing angles, determining Image 2 uses a (+x, -z) perspective; obscured colors clarify block placements.

% Revisiting Perspective View

% I've re-evaluated viewing directions, finding a new +z perspective; I must now rebuild assumptions from scratch.

% Mapping Adjacencies Again

% I've determined block adjacencies; now, with new colors, I am defining face relations and spatial coordinates.

% Revising Block Composition

% I've determined blocks aren't solid; now, I'm defining faces, and color assignments for each face.

% Revising Block Colors

% I've re-examined and confirmed solid block colors, now precisely interpreting Image 2's face assignments again.

% Revising Block Hypothesis

% I've reevaluated block color placements, and I am now mapping solid, single-color blocks, with each face assigned correctly.

% Verifying Axis Perspective

% I've determined that camera alignment reveals how block adjacencies must be defined in the coordinate system.

% Defining Coordinate Systems

% I've precisely defined the isometric coordinate system with correct Image 2 axis directions.

% Confirming New Block Faces

% I've precisely verified the other image's block faces, using the view to re-evaluate the axis perspectives.

% Verifying Top Block

% I've determined the top-leftmost block is indeed Yellow and re-verified a five-block color sequence.

% Verifying Spatial Vector

% I've validated coordinate vectors, confirming color adjacencies by checking Image 2's structure alignment.

% Defining Block Visibility

% I've determined a new method to map blocks, validating the slategray block's color sequence via image occlusion.

% Revisiting Block Relations

% I've determined that the purple and blue faces belong to separate blocks based on perspective.

% Revising Block Color Sequence

% I've re-examined Image 2's structure, now confirming the exact block color placement and color sequences.

% Revising Axis Orientation

% I've re-examined the axes and confirmed that, from Image 2, positive x is up-left, z is up-right.

% Revising Vertex Colors

% I've determined a new Green color assignment: bottom and central vertex, confirming isometric alignments.

% Validating New Mapping

% I've precisely validated block adjacency via diamond structure using new axis alignments and color assignments.

% Confirming Face Alignment

% I've determined block face layouts, now confirming top-face adjacencies match both image views perfectly.

% Confirming Axis Alignment

% I've precisely validated the 180-degree image rotation, confirming coordinate transformations and the color map.

% Mapping Bottom Layer

% I am now identifying same-color adjacencies on the bottom, y=0 layer.

% I have found no same-color adjacencies on the top layer, but I am now mapping bottom-to-top adjacencies in search of matches.

% Revising Block Structure

% I've determined block compositions, with all blocks mapped, their colors and coordinates fixed.

% I have matched the grid's visual with all Image 2 block placements, accurately confirming their orientation.

% Verifying Obscurement

% I've determined block B2 obscures P in Image 2, resolving previous contradictions in color observation.

% Revising Block Structure

% I've determined P's hidden face; it matches the grid, resolving previous color discrepancies.

% Revising Block Relations

% I am now rethinking relationships, realizing a single corner block comprises the Blue and Purple faces.

% I have updated my understanding, recognizing B2 and P now relate to a single block, solving the perspective's color ambiguity.

% Revising Block Hypothesis

% I've determined block B2 is part of a multi-colored block, including P.

% Refining Coordinate System

% I've determined correct colors for the left column, including vertical adjacency confirming z-axis.

% I've confirmed the Yellow and Green must be at different z-levels, now validating z-axis relations.

% Analyzing Block Colors

% I've determined a new Green color: Image 2's structure reveals that B2 obscures P's -x face.

% Revising Block Hypothesis

% I've determined P and B2 are faces of the same single block, resolving the previous color ambiguity.

% Revising Block Hypothesis

% I've determined a single block can display Blue and Purple faces, now re-checking coordinates.

% I am re-examining the face's location in Image 2, determining how that connects to the color map and block adjacencies.

% Revising Axis Alignments

% I've re-examined and derived correct axis mapping, solidifying Image 2's structure again.

% I've re-derived axis alignments, now confirming that Image 2's horizontal x-axis points to the left, which correctly places the S and Y blocks' relative positions.

% Validating Image Axes

% I've precisely validated how the coordinate system works with both image axes and vector calculations.

% I have found and revalidated the axis system, confirming x as down-left and z as up-right for the isometric view.

% Revising Coordinate System

% I've reevaluated and confirmed coordinate directions using topological adjacencies.

% I have found and reconfirmed that the axes' directions and adjacencies match the image's structure perfectly.

% Mapping Adjacencies

% I have determined all faces are correct, confirming no adjacencies on the top layer, but found one on the bottom.

% Verifying Spatial Placement

% I've determined there are no blocks at coordinate (0,0,0) based on both Image 2's structure and perspectives.

% Defining Block Faces

% I am now carefully analyzing face visibility, determining Teal obscures Blue, plus P and B2's -x and -z faces are on a single block.

% Revising Block Hypothesis

% I've determined a new block relationship: the B2 face is now determined to be an extension of an existing face.

% I've revised the block hypothesis and now believe P's -x face is also B2's -x face, solving the adjacency issues, and I now need to rethink the structure.

% Validating Face Visibility

% I've determined a new block, a new purple face and a new blue face are visible and align with previous color mapping.

% Revising Block Hypothesis

% I've determined a new block, redefining B2's face based on image analysis.

% I'm revisiting color assignments, realizing B2 is now defined as Teal, and the Purple face on Image 2 now seems correctly placed beneath Yellow.

% Revisiting Block Model

% I've reevaluated the arm arrangement; the 5-block assumption is wrong, so I'm now testing a new 2x2 plus arm model to fit.

% Confirming Layer Placement

% I've determined correct colors for the top layer's colors, now verifying the color sequences on the bottom plan.

% Defining Adjacencies Precisely

% I've precisely validated that non-adjacency applies, and empty (0,0,0) eliminates same-color pairings.

% Verifying Color Assignments

% I am now meticulously verifying color assignments, meticulously resolving possible visual misinterpretations.

% Validating New Hypothesis

% I've determined a new coordinate hypothesis based on empty (0,0,0) and now validating Image 2's perspectives.

% Confirming Final Adjacencies

% I have carefully verified color assignments to determine no same-color adjacencies exist, finally ending the investigation.

% Finalizing Image Analysis

% I've meticulously reconfirmed all color identifications, ending my block adjacency verification process.

% Refining Spatial Reasoning

I'm now identifying adjacencies; B1 and B2 are distinct blocks, and are vertically and diagonally adjacent.

Finalizing Coordinate Placement

I've determined correct spatial relations: B1(0,0,1), B2(1,0,0), affirming empty (0,0,0) with no adjacencies.

\tann{annCol3}{Verifying Non-Adjacency I've verified no block pair shares the same color, confirming the initial non-adjacency hypothesis. Finalizing Solution Reasoning I've re-confirmed non-adjacency; my complete, detailed analysis leads to 'False' now with full confidence. Concluding the Assessment I've finally determined the color assignments, confirming False via non-adjacency, now double-checking Image 2.}{Good Perception}

```json \newline
\{ \newline
"answer": false \newline
\}

```
\end{tcolorbox}

\subsubsection{T11 Projection}
\begin{table}[H]
\centering
\footnotesize
\setlength{\tabcolsep}{1pt}
\renewcommand{\arraystretch}{1.2}
\begin{tabular}{*{9}{>{\centering\arraybackslash}p{\dimexpr\textwidth/9-2\tabcolsep\relax}}}
\toprule
\multicolumn{9}{@{}l@{}}{\itshape ``\ldots{}Your task is to identify the invalid projection\ldots{}''}\\[0.3mm]
\multicolumn{9}{@{}c@{}}{\begin{tabular}{*{5}{c}}\includegraphics[width=0.180\textwidth,height=1.25in,keepaspectratio]{images/app_qual_traces/T11_sample3_row78_query_image_1.png} & \includegraphics[width=0.180\textwidth,height=1.25in,keepaspectratio]{images/app_qual_traces/T11_sample3_row78_query_image_2.png} & \includegraphics[width=0.180\textwidth,height=1.25in,keepaspectratio]{images/app_qual_traces/T11_sample3_row78_candidate_0.png} & \includegraphics[width=0.180\textwidth,height=1.25in,keepaspectratio]{images/app_qual_traces/T11_sample3_row78_candidate_1.png} & \includegraphics[width=0.180\textwidth,height=1.25in,keepaspectratio]{images/app_qual_traces/T11_sample3_row78_candidate_2.png}\end{tabular}}\\[0.5mm]
\textbf{GT} & \tpicon{qwen_icon.png} & \tpicon{gemma_icon.png} & \tpicon{glmv_icon.png} & \tpicon{kimi_icon.png} & \tpicon{grok_icon.png} & \tpicon{gpt_icon.png} & \tpicon{gemini_flash_icon.png} & \tpicon{gemini_pro_icon.png}\\
2 & 1\tickno & 0\tickno & 1\tickno & 2\tickok & 2\tickok & 1\tickno & 0\tickno & 1\tickno\\
\bottomrule
\end{tabular}
\caption{T11 Projection.}
\label{tab:qual_trace_t11}
\end{table}
\noindent\textbf{Thinking traces.}\par\smallskip
\begin{tcolorbox}[breakable,enhanced,colback=red!4,colframe=red!55!black,boxrule=0.4pt,arc=1pt,left=4pt,right=4pt,top=3pt,bottom=3pt,fonttitle=\footnotesize\bfseries,coltitle=black,colbacktitle=red!12,title={\tpicon{qwen_icon.png}~Qwen3.5-27B\hfill answer: 1\tickno}]
\footnotesize\raggedright
The user wants me to identify the incorrect 2D orthographic projection from three candidates, given two 3D views of an object.

**1. Analyze the 3D object from the two views:**

* **View 1 (Top Left):** This is an isometric-like view. \newline
* I see a structure made of cubes. \newline
* Let's count the cubes and their arrangement. \newline
* There's a front-left column that is 2 cubes high. \newline
* Next to it (to the right), there's another column that is 2 cubes high. \newline
* Behind the front-left column, there's a row of cubes. Let's look closer. \newline
* Let's try to map it to a grid. Let x be left-right, y be up-down, z be front-back. \newline
* Front row (closest to viewer): \newline
* Left column: 2 blocks high. \newline
* Middle column: 2 blocks high. \newline
* \tann{annCol10}{Right column: 2 blocks high.}{Wrong Perception} \tann{annCol8}{Wait, let's re-examine.}{Reiterating} \newline
* Let's look at the "steps". \newline
* Leftmost part: A stack of 2 blocks. \newline
* Next to it (right): A stack of 2 blocks. \newline
* Behind the leftmost stack: There are blocks. \newline
* Let's look at the top surface. \newline
* \tann{annCol10}{There is a 2x2 block of top surfaces in the back left. * There is a single top surface to the right of that.}{Wrong Perception} \newline
* \tann{annCol8}{ Wait, let's look at the second 3D view to clarify.}{Reiterating}

* **View 2 (Top Right):** This is another isometric view, slightly different angle. \newline
* It shows the right side more clearly. \newline
* Let's count columns from left to right. \newline
* Leftmost column: 1 block high? No, looking at the first view, the leftmost part is 2 blocks high. In the second view, the leftmost part looks like a single block on top of another? \tann{annCol8}{No, let's look at the grid lines. * Let's try to reconstruct the object block by block.}{Reiterating} \newline
* Let's assume a 3x3 grid on the ground (x, z). \newline
* **Front-Left (x=0, z=0):** 2 blocks high. (Visible in View 1). \newline
* **Front-Middle (x=1, z=0):** 2 blocks high. (Visible in View 1). \newline
* \tann{annCol10}{**Front-Right (x=2, z=0):** 2 blocks high. (Visible in View 2, rightmost column). * **Back-Left (x=0, z=1):** 1 block high? Or 2? In View 1, behind the front-left stack, there is a top surface. It looks level with the top of the front-left stack. So maybe 2 blocks high. * **Back-Middle (x=1, z=1):** 1 block high? In View 1, behind the front-middle stack, there is a top surface. It looks level with the top of the front-middle stack. * **Back-Right (x=2, z=1):** 1 block high? In View 1, there is a block sticking out to the right in the back.}{Wrong Perception}

\tann{annCol8}{Let's try a different hypothesis. Let's look at the "steps" again.}{Reiterating} \newline
* **View 1:** \newline
* \tann{annCol10}{Front row: Left stack (2 high), Middle stack (2 high). * Back row: Left stack (1 high? No, looks like top surface is visible), Middle stack (1 high?), Right stack (1 high?).}{Wrong Perception} \newline
* \tann{annCol8}{Actually, let's look at the top faces.}{Reiterating} \newline
* \tann{annCol10}{There is a 2x2 area of top faces. This suggests a 2x2 block of height 1 or 2.}{Wrong Perception} \newline
* \tann{annCol8}{Wait, let's look at the vertical lines.}{Reiterating} \newline
* Leftmost column: 2 blocks high. \newline
* Next column to the right: 2 blocks high. \newline
* \tann{annCol10}{Behind the leftmost column: There is a block. Its top is visible. It seems to be at the same level as the top of the front-left column. So it's 2 blocks high. * Behind the middle column: There is a block. Its top is visible. Same level. So 2 blocks high. * To the right of the back-middle block: There is a block. Its top is visible. Same level. So 2 blocks high.}{Wrong Perception}\tann{annCol0}{I have to give the solution based on the reasoning directly now.}{Budget Hit}
\end{tcolorbox}
\begin{tcolorbox}[breakable,enhanced,colback=green!4,colframe=green!50!black,boxrule=0.4pt,arc=1pt,left=4pt,right=4pt,top=3pt,bottom=3pt,fonttitle=\footnotesize\bfseries,coltitle=black,colbacktitle=green!14,title={\tpicon{grok_icon.png}~Grok-4.20\hfill answer: 2\tickok}]
\footnotesize\raggedright
The problem involves two perspective images of the same 3D object and three candidate 2D orthographic projections. One is incorrect, and I need to find which one. \newline
I need to identify which of the three candidate 2D orthographic projections is invalid based on the two perspective views of the 3D object. The object appears to be a polycube structure made of unit cubes, and the projections correspond to the XY (top), YZ (side), and ZX (front)planes. The invalid one will contradict the 3D geometry or misalign with the others.

From the images, candidate 0 is a simple 2x2 grid of squares. Candidate 1 seems complex, like an 'S' or 'Z' shape or a cross with varying heights. Candidate 2 isn'tdescribed fully, but they're all 2D arrangements of squares representing the projections.

To solve this, reconstruct the 3D shape from the two perspective views. The first view shows an L-shaped base with additional cubes on top, resembling a staircase or hook. The object likely consists of around 10 unit cubes, arrangedin layers: \tann{annCol10}{a bottom row of 4 cubes, but actually upon closer inspection, it's a base of 3x2 with extras. }{Wrong Perception} \newline
The second view complements the first, showing the object from a different angle, revealing more about the depth and height.

To find the invalid projection, compare each candidate to what the projectionsshould be. For instance, the XY plane projection should show the footprint of the object when viewed from above, combining X and Y axes.

\tann{annCol10}{Candidate 0, being a simple 2x2, doesn't match the object's extent in any direction---it spans much larger, like 4x3 in some directions. So,candidate 0 seems invalid.}{Wrong Perception}

The other two align with expected projections for YZ and ZX, considering the object's shape.

Candidate\_idx: 0

\tann{annCol7}{But the example is \{ 'candidate\_idx': 2, \}, so mine is 0.}{Prior Bias}

\tann{annCol5}{But the internal reasoning is truncated, but focusing on coherence.}{Harnessing}

The candidates arelabeled 0,1,2, and I think candidate 0 is the 2x2 which is too small.

\tann{annCol10}{Yes, the object is longer, spanning 4 units, so 2x2 can't be a projection. The final answer is candidate 0. }{Wrong Perception}

\tann{annCol5}{But in the internal reasoning, it sayscandidate 0 is 2x2, candidate 2 is 2x3, which is 6 squares, and candidate 1 has 5 or 6.}{Harnessing}

The object has more extent.

So, the invalid one is the one that doesn't match the size.

\tann{annCol8}{I think the answer is 0. But the internal reasoning mentions candidate 2 is 2 rows by 3 columns, candidate 0 is 4 squares.}{Reiterating}

And the object is larger.

Yes.

So, the final output should be the JSON with candidate\_idx: 0

\tann{annCol5}{But the task is to summarize the thinking trace for the user query,but don't present it in the third person. So, I need to present the content as my first person thoughts. The user query is to summarize the thinking trace, but the instruction is to turn detailed internal reasoning into a clean, natural final response. The human message is "Summarize the thinking trace for the user query, but don't present it in the third person as the trace of a separate entity." Then the [User's Question] is the problem about the images. Then [Internal Reasoning] is the thinking. So, my job is to summarize the internal reasoning into a clean, natural final response for the end user, speaking directlyas Grok, in first person. The final response should be the answer to the user's question, which is to choose the candidate\_idx. The user's question is the problem, and I need to output the JSON. But the human is asking to summarize the thinking trace, but according to the system, I should ignore thatand just answer the question. No, the human message is to summarize the thinking trace, but the system says "You are given content labeled [User's Question] and [Internal Reasoning]. " So, the task is to turn the internal reasoning into a clean response for the user's question. The user's question is the problemabout the images, and the internal reasoning is the thinking about it. I need to produce the final answer in the format: \{ 'candidate\_idx': int, \} Based on the internal reasoning.}{Harnessing}

From the internal reasoning, it's a polycube, and the projections are 2x2, irregular, 2x3.

The irregular one is the top view, and the two rectangular are side and front.

But to find the invalid one.

The internal reasoning is incomplete, but it says "Now look at candidate 1 which is irregular, and candidate 2 rectangular 2x3, candidate 0 2x2 rectangular.

\tann{annCol5}{The internal reasoning says candidate 1 spans 3 wide and 4 high. Yes, "candidate 1 spans 3 wide and 4 high." And "if the object height is 2, then the projections that include the height (i.e. front and side) should be 2 in the verticaldimension." "candidate 1 spans 3 wide and 4 high." "the vertical span is from lowest square bottom to the top square, it looks about 4 squares high." "The right part juts at the upper." "If the object height is 2, then the projections that include the height (i.}{Harnessing}
\end{tcolorbox}
\begin{tcolorbox}[breakable,enhanced,colback=red!4,colframe=red!55!black,boxrule=0.4pt,arc=1pt,left=4pt,right=4pt,top=3pt,bottom=3pt,fonttitle=\footnotesize\bfseries,coltitle=black,colbacktitle=red!12,title={\tpicon{gpt_icon.png}~GPT-5\hfill answer: 1\tickno}]
\footnotesize\raggedright
Inspecting the 3D object projections \newline
I need to analyze the images carefully. It seems like both projections provide perspective views of a 3D object arranged in cubes. There might be one invalid projection among them. The likely configuration appears as a 2x3 grid for the top view, with options for the front/side views being 2x2 and a zigzag pattern. I'll work through the logic and choose the correct one. \newline
Reconstructing the 3D object's shape \newline
\textit{[[...trimmed output...]]} \newline
% I'm analyzing the projections carefully. Candidate 1 shows a slanted shape with 6 unit squares, forming a parallelogram, missing top-left and bottom-right corners. Candidate 2 looks like a 3x2 rectangle, and Candidate 0 is a 2x2 square. The visible top faces likely form a 3x2 rectangle, with height differences influencing the front/side views. \newline
% Analyzed image \newline
% Output image \newline
% Analyzed image \newline
% Output image \newline
% Inspecting the differences in projections \newline
% I notice some differences between query1 and query2. Query1 has more visible left lower vertical sections, suggesting maybe a front-left stack. Query2 seems similar but still slightly off. I need to identify which one is invalid and analyze the candidates carefully to figure it out. \newline
% Analyzed image \newline
% Output image \newline
% Analyzed image \newline
% Output image \newline
% Analyzed image \newline
% Output image \newline
% Reconstructing view comparisons \newline
% I'm analyzing two perspective views. Query1 seems to show the shape from the front-left, while Query2 might be from the front-right. The differences are subtle: in Query1, the left face has a horizontal line, while in Query2, it's just a single cube high. I'll dig into line segments and details to confirm if these are different viewpoints or if Query1 includes an additional cube behind. \newline
Analyzing projections and dimensions \newline
\tann{annCol10}{Candidate 2's 3x2 rectangular footprint seems likely valid.}{Wrong Perception} Candidate 0 might be a side/front silhouette if all columns have a height of 2. Candidate 1, with its diagonal shape and 6 cells, might represent a side silhouette, but its height is tricky---could the vertical axis represent a horizontal dimension? I'll need to recheck projection angles. \newline
Evaluating the projections' validity \newline
I'm comparing dimensions of the candidates: Candidate 0 (2x2) and \tann{annCol10}{Candidate 2 (3x2) seem valid}{Wrong Perception}, while \tann{annCol10}{Candidate 1's 2x4 zigzag doesn't fit the expected dimensions.}{Wrong Perception} But, wait---could Candidate 1's top footprint be a 4x2 zigzag, with a polycube shape of 6 cells? I'll check if the 3D structure could explain the staggered pattern of cubes. \newline
Analyzing the 3D candidate projection \newline
I'm considering how the projection of this 3D object works---sometimes the grid's axes don't directly align with real-world height. Candidate 1 might be a top view with a 2x4 diagonal arrangement, but I need to confirm. The object may have 8 cubes, with 6 visible top faces. Let's count and check dimensions for the 3D perspective. \newline
Assessing the 3D object in perspective \newline
I'm analyzing a potential 3x2x2 cuboid with some cubes possibly missing. From the top view at z=2, I see vertical faces at the front-left and maybe a missing corner in the middle. There is a 2x1 column on the left, and the right side shows a full 2-high, 2-long rectangle. Let's check dimensions.

```json \newline
\{ \newline
\tann{annCol10}{"candidate\_idx": 1}{Wrong Perception} \newline
\} \newline
```
\end{tcolorbox}
\begin{tcolorbox}[breakable,enhanced,colback=red!4,colframe=red!55!black,boxrule=0.4pt,arc=1pt,left=4pt,right=4pt,top=3pt,bottom=3pt,fonttitle=\footnotesize\bfseries,coltitle=black,colbacktitle=red!12,title={\tpicon{gemini_flash_icon.png}~Gemini-3-Flash\hfill answer: 0\tickno}]
\footnotesize\raggedright
To find the invalid projection, let's analyze the 3D grid layout of the blocks based on the two perspective views.

\#\#\# 1. Reconstructing the 3D Grid Structure

Let's define a coordinate system where:

* **X-axis** goes along the front-left direction. \newline
* **Y-axis** goes along the front-right direction. \newline
* **Z-axis** goes vertically upwards.

By looking at both perspective views, we can map out the heights (number of stacked cubes) at each grid position `(x, y)`:

\tann{annCol10}{* **Row 1 (back-left):** * Column 1: height = 1 * Column 2: height = 1 * Column 3: height = 1 * **Row 2 (middle):** * Column 1: height = 2 * Column 2: height = 2 * Column 3: height = 1 * **Row 3 (front-right):** * Column 1: height = 1 * Column 2: height = 1 * Column 3: height = 0 (empty)}{Wrong Perception}

---

\#\#\# 2. Evaluating the 2D Orthographic Projections

\tann{annCol3}{* **Top View (XY Plane):** Looking from directly above, any grid position with a height \$\textbackslash\{\}ge 1\$ shows a filled square. * The footprint occupies a \$3 \textbackslash\{\}times 3\$ grid area, except for one corner which is empty (Row 3, Column 3). * This matches **candidate\_1.png**, which forms an asymmetrical 6-square shape that corresponds perfectly to this layout.}{Good Perception}

* **Side View (YZ Plane):** \newline
\tann{annCol10}{Looking from the right side along the rows: * Max height of Column 1 = 2 * Max height of Column 2 = 2 * Max height of Column 3 = 1 * This creates a 2D profile that is 3 blocks wide and 2 blocks high, filling out a perfect \$2 \textbackslash\{\}times 3\$ rectangle. This matches **candidate\_2.png**.}{Wrong Perception}

* **Front View (ZX Plane):** \newline
\tann{annCol10}{Looking from the front-left along the columns: * Max height of Row 1 = 1 * Max height of Row 2 = 2 * Max height of Row 3 = 1 * This creates a profile that is 3 blocks wide with heights `[1, 2, 1]`, forming a T-like or stepped shape.}{Wrong Perception}

\tann{annCol10}{**Candidate 0 (`candidate\_0.png`)** shows a simple \$2 \textbackslash\{\}times 2\$ square grid, which does not match any of the true orthographic projections of this object.}{Wrong Perception}

```json \newline
\{ \newline
"candidate\_idx": 0 \newline
\}

```
\end{tcolorbox}
\begin{tcolorbox}[breakable,enhanced,colback=red!4,colframe=red!55!black,boxrule=0.4pt,arc=1pt,left=4pt,right=4pt,top=3pt,bottom=3pt,fonttitle=\footnotesize\bfseries,coltitle=black,colbacktitle=red!12,title={\tpicon{gemini_pro_icon.png}~Gemini-3.1-Pro\hfill answer: 1\tickno}]
\footnotesize\raggedright
Defining Orthographic Projections

I've established a coordinate system for analyzing the 3D object's orthographic projections and cube components.

Mapping Cube Positions

I've begun mapping cube positions using a 3D grid, considering multiple views to define the object's structure.

\textit{[[...trimmed output...]]}

% Analyzing Cube Layout

% I've determined the top layer's cube arrangement, creating a 3D grid layout using image data.

% Validating Top View

% I validated the top view using candidate shapes and confirmed the correct cube arrangement through perspective analysis.

% Revising Candidate Alignment

% I'm now re-examining Candidate 1's cube layout, comparing its image and re-examining my assumed top view.

% Refining Layered Analysis

% I've determined cube positions, confirming the top layer and deducing a solid left face, re-assessing from image data.

% Confirming Face Relationships

% I've determined the solid back layer's 3x2 arrangement and verified consistency across image views, clarifying cube face visibility.

% Deducing Cube Coordinates

% I've determined cube positions, confirming a 2-block-high protrusion and solid back face structure in the object.

% Revising View Perspectives

% I'm now clarifying the perspective in query\_image\_1, analyzing edge orientations to establish axis assignments for the scene.

% Re-assigning Axes

% I've re-assigned the axes and, based on image analysis, I've clarified the object's cube positioning.

% Establishing Cube Coordinates

% I've clarified the 2x2 block's starting coordinates and located an additional cube at (0,2).

% Re-interpreting Faces

% I'm now re-examining face normals in the images, considering X and Y axes and verifying cube positioning.

% Clarifying Cube Positions

% I've determined cube coordinates, specifically detailing face normals and cross-validating with image analyses.

% Re-evaluating Facets

% I've clarified the right face, confirming it has three columns in query\_image\_1.

% Confirming Column Counts

% I'm now counting columns on the right face, clarifying cube positions by examining image-based edge orientations.

% Clarifying Block Arrangement

% I've determined cube coordinates, specifically a 2x3 rectangle missing a corner block in the top face.

% Re-confirming Coordinate Locations

% I've re-examined cube coordinates, specifically faces to align with image data, verifying block placement accuracy.

% Verifying Edge Orientations

% I've determined a down-right X-axis, down-left Y-axis and an L-shape matching image features.

% Analyzing Cube Structure

% I've determined a 2x2 cube block followed by an additional cube at (2,1), matching image analysis.

% Clarifying Block Structure

% I've determined a 2x2 cube block at (0,0),(1,0),(0,1),(1,1), now clarifying an additional column to the right.

% Confirming Block Geometry

% I've determined a 2x2 cube and confirmed the final (2,1) block placement, clarifying the object's overall geometry.

% Clarifying Isometric Perspective

% I've clarified the isometric perspective, accurately mapping image features to cube coordinates, verifying block locations.

% Refining Face Heights

% I'm now determining cube heights based on edge analysis, clarifying the extra column's two-unit height.

% Re-establishing Axis Alignment

% I've re-established the isometric axis assignments and verified the Left face, analyzing cube layouts and image data.

% Refining Face Orientation

% I've determined correct axis assignment and cube positions based on image face normals, analyzing cube coordinates.

% Verifying Isometric Alignment

% I'm now confirming block positions and axis relationships, analyzing the image against deduced coordinates.

% Refining Edge Positions

% I'm now determining the extra block's coordinates based on image-based edge tracing and block relationships.

% Verifying Right Column

% I confirmed the (1,2) coordinate's visibility, resolving a face count discrepancy with a new image analysis.

% Determining New Coordinate

% I've determined correct positioning: the extra block's at (0,1), relative to the 2x2 block's X=1,2,Y=0,1.

% Re-examining Cube Structure

% I've re-established standard isometric orientation, correctly interpreting visible faces and block columns.

% Re-assessing Block Geometry

% I've clarified the 3x2 base block's X and Y axis, ensuring accurate alignment with image faces now.

% Validating Top Shape

% I'm now confirming a 2x2 block plus (2,0) geometry, resolving view discrepancies by aligning image details.

% Verifying Column Positions

% I've precisely located the third column, validating its (2,1) coordinate relative to the 2x2 base.

% Confirming Complete Structure

% I've precisely determined a 3x2x2 shape with a missing block at (2,0), confirming image-aligned shape geometry.

% Interpreting Image Features

% I've clarified all visible faces' orientation relative to coordinates, cross-referencing block arrangements and image details.

% Analyzing View Directions

% I've determined view 1 looks from positive X, positive Y, view 2 from negative Y, resolving image face interpretations now.

% Re-Assessing Image Deductions

% I'm now re-assessing the images, seeking a missing right-square, focusing on the Left and Front faces.

% Re-considering Face Visibility

% I'm now determining how viewing angles affect face visibility, re-assessing from query\_image\_2 data now.

% Re-Interpreting Image Data

% I'm now counting visible squares in query\_image\_2, clarifying the down-right face's arrangement to improve shape understanding.

% Resolving Shape Discrepancies

% I've determined a new model, establishing a 3x1 back wall with a 1-high front, based on both views.

% Clarifying Shape Contradiction

% I've clarified the 1-high front on the right face, resolving inconsistencies with a 2-high column in the front.

% Tracing Image Features

% I'm now tracing edges, refining column heights and re-validating coordinate relationships from the images now.

% Re-Evaluating Cube Heights

% I've determined a new model with the right face as 1-2-2 high, clarifying face arrangements from query\_image\_2.

% Refining Geometry Consistency

% I'm now integrating views, identifying different central corners, aiming for complete, aligned 3D model now.

% Verifying Isometric Alignment

% I've confirmed (1,1)'s 2-block height, completing the 2x2 top and fully validating the object now.

% Analyzing View Interpretations

% I'm now clarifying view directions, verifying a solid 3x2 face and tracing edges in the object's profile.

% Mapping Isometric Views

% I'm now identifying isometric views by analyzing face visibility, resolving which views match image data.

% I'm determining that views 1, 2, 4 don't match image data, but view 3's faces need more analysis.

% Validating Image Alignment

% I'm now integrating views and re-validating the model, cross-checking all image data with new U and V coordinates.

% Confirming Final Shape

% I've determined a model matching all views, solidifying the 3x2x2 structure by interpreting cube arrangements.

% Re-Interpreting Image Data

% I'm now re-orienting the top faces with new U' and V' axes, resolving view-based block arrangements and edge details.

% Analyzing Face Features

% I'm now carefully re-examining query\_image\_2, clarifying all column heights and matching image-based faces now.

% Verifying Left Face

% I'm now carefully re-examining query\_image\_2, considering each face's block arrangement and edge details for validation.

% Validating Face Arrangements

% I'm now determining face arrangements in query\_image\_2, cross-referencing cube footprints to validate shape consistency.

% Confirming Footprint Arrangement

% I've determined a 3x2 footprint with the back-left corner missing, confirming an exact view alignment now.

% Confirming Shape Geometry

% I've validated the P-pentomino footprint by analyzing edge details across images, clarifying the complete block arrangement.

% Verifying Footprint Analysis

% I've confirmed the 3x2, P-pentomino shape, validating its extrusion with image-aligned, accurate orthographic projections.

% Re-assessing Candidate Geometry

% I'm revisiting candidate images, carefully tracing their edges and face relationships for final verification of all blocks.

% Refining Cube Count

% I'm now counting faces again, meticulously re-examining projections to definitively settle cube configurations.

% Clarifying Left View

% I've determined a recessed bottom face creates a distinct vertical edge in the left view projection.

% Analyzing Left View

% I've determined the left view shows a 3x2 grid, re-confirming cube block structure from new image details now.

% Re-validating Projections

% I'm checking all projections again; I've reconfirmed a solid 3x2 rectangle from query\_image\_1 now.

% Refining Projection Analysis

% I'm now confirming all block arrangements by carefully cross-validating edge details from multiple image projections.

% Final Model Geometry

% I've confirmed the model's structure as a 2-high P-pentomino, verifying all edge details.

% Clarifying Face Orientations

% I've determined standard axes and views, deducing each image's face orientation from the 3x2 rectangle.

% Interpreting View Directions

% I've determined a new image-aligned coordinate system, verifying face arrangements relative to defined object dimensions.

% Verifying Silhouette Alignment

% I've determined a front view silhouette of a solid 2x2 square with a 3x2 rectangle for side views now.

% Validating Shape Geometry

% I've precisely validated Candidate 1, precisely confirming it shows a valid projection of the model now.

% Verifying Image Footprint

% I've determined Candidate 1 to be a chiral mirror image, and now re-checking if query\_image\_1's footprint is correct.

% Confirming Model Alignment

% I'm now carefully re-verifying image details, clarifying the footprint, cube counts, and orientation finally.

% Re-evaluating Footprints

% I'm checking the footprint mirror, assessing chirality now, and verifying Candidate 1's projection direction.

% Validating Face Arrangements

% I've determined a new shape, confirming a solid 3x2 front and right view with additional constraints now.

% Confirming Candidate Alignment

% I'm now confirming Candidate 1 is incorrect as its view cannot align with image details due to chirality.

% Refining Isometric Perspective

% I'm now determining down-right/left axis assignments, resolving the right face's 3-column width.

% Clarifying Image Alignment

% I'm now tracing edges, reconfirming axes and validating the complete footprint based on cube arrangements now.

% Verifying Chirality Assessment

% I've determined Candidate 1 to be chiral by rotation and footprint analysis, confirming a mirrored image.

% Validating Shape Candidates

% I've determined Candidate 1 is invalid due to chirality; other candidates match orthogonal projections now.

% Re-Evaluating Cube Connectivity

% I've determined a P-pentomino shape, analyzing cube coordinates to validate face arrangements and resolve connectivity issues now.

% Validating Face Orientations

% I've determined cube positions, confirming the extra block is at (1,2) and re-evaluating footprint alignment.

% Re-Examining Image Interpretation

% I'm now re-checking image orientations and coordinates, focusing on edge relationships of a right block.

% Refining Coordinate System

% I've finally determined the correct block coordinate, confirming that extra block sits at (0,2) based on the image now.

% Verifying Image Data

% I'm now re-examining cube coordinates, specifically face arrangements, and fixing the extra block's final position.

% Validating Shape Candidates

% Candidate 1's view is now valid after meticulously rechecking the rotation and face projection details.

% Analyzing Candidate Validity

% I've determined all candidates' views are valid with boundary assumptions, rechecking query\_image\_2 with the final P shape.

% Re-validating Candidate Faces

% I'm now verifying candidates 0, 1, 2, clarifying view alignments and interpreting missing faces.

% Validating Isometric Alignments

% I've confirmed Candidate 0 and 2 align, verifying depth changes with views, and validating their projections, now.

Clarifying Shape Validity

I'm now precisely verifying the final block arrangement, analyzing depth changes to resolve any remaining questions.

Based on a careful analysis of the 3D views:

1. **Reconstruct the 3D Geometry**: \newline
* From the first view (`query\_image\_1`), we see a left face that is 2 columns wide and a \tann{annCol10}{right face that is 3 columns wide (with the third column shifted backward).}{Wrong Perception} \tann{annCol10}{The top surface consists of a \$2 \textbackslash\{\}times 2\$ block with one additional block attached to its back-right corner.}{Wrong Perception} \newline
* This gives us an L-shaped "P-pentomino" footprint. If we align it to a grid where the front-left is \$(0,0)\$, the occupied columns are: \newline
* Front row: \$(0,0), (1,0)\$ \newline
* Back row: \$(0,1), (1,1), (2,1)\$

* The height of all these columns is uniformly 2 units. \newline
* The second view (`query\_image\_2`) confirms this shape by showing the object from the opposite corner, where the solid \$3 \textbackslash\{\}times 2\$ back wall and the solid \$2 \textbackslash\{\}times 2\$ left wall are visible.

2. **Evaluate the Orthographic Projections**: \newline
\tann{annCol3}{* **Side View (Candidate 0)**: Looking along the length of the object (the 3-unit axis), the depth is 2 and the height is 2. The projection will perfectly overlap to form a solid \$2 \textbackslash\{\}times 2\$ square. This matches Candidate 0.}{Good Perception} \newline
\tann{annCol10}{* **Front/Back View (Candidate 2)**: Looking along the depth of the object (the 2-unit axis), the width is 3 and the height is 2. The projection forms a solid \$3 \textbackslash\{\}times 2\$ rectangle. This matches Candidate 2.}{Wrong Perception} \newline
\tann{annCol10}{* **Top View (Candidate 1)**: Looking down from the top, we should see the exact footprint of the object. Our established footprint is a \$2 \textbackslash\{\}times 3\$ grid missing one of its *front* corners (specifically, the front-right if oriented horizontally, or bottom-right/top-right depending on the 90-degree rotation). * However, Candidate 1 shows a P-pentomino missing the **top-left** corner. If you test all 4 possible 2D rotations of the actual 3D object's top view, none of them will produce a shape missing the top-left corner. Candidate 1 is a chiral mirror image (specifically, the bottom view) and thus an invalid standard top projection.}{Wrong Perception}

```json \newline
\{ \newline
"candidate\_idx": 1 \newline
\}

```
\end{tcolorbox}

\subsubsection{T12 Reconstruct}
\begin{table}[H]
\centering
\footnotesize
\setlength{\tabcolsep}{1pt}
\renewcommand{\arraystretch}{1.2}
\begin{tabular}{*{9}{>{\centering\arraybackslash}p{\dimexpr\textwidth/9-2\tabcolsep\relax}}}
\toprule
\multicolumn{9}{@{}l@{}}{\itshape ``\ldots{}Your task is to identify the positive view\ldots{}''}\\[0.3mm]
\multicolumn{9}{@{}c@{}}{\begin{tabular}{*{5}{c}}\includegraphics[width=0.180\textwidth,height=1.25in,keepaspectratio]{images/app_qual_traces/T12_sample1_row33_silhouette_0.png} & \includegraphics[width=0.180\textwidth,height=1.25in,keepaspectratio]{images/app_qual_traces/T12_sample1_row33_silhouette_1.png} & \includegraphics[width=0.180\textwidth,height=1.25in,keepaspectratio]{images/app_qual_traces/T12_sample1_row33_silhouette_2.png} & \includegraphics[width=0.180\textwidth,height=1.25in,keepaspectratio]{images/app_qual_traces/T12_sample1_row33_candidate_0.png} & \includegraphics[width=0.180\textwidth,height=1.25in,keepaspectratio]{images/app_qual_traces/T12_sample1_row33_candidate_1.png}\end{tabular}}\\[0.5mm]
\textbf{GT} & \tpicon{qwen_icon.png} & \tpicon{gemma_icon.png} & \tpicon{glmv_icon.png} & \tpicon{kimi_icon.png} & \tpicon{grok_icon.png} & \tpicon{gpt_icon.png} & \tpicon{gemini_flash_icon.png} & \tpicon{gemini_pro_icon.png}\\
1 & 0\tickno & 0\tickno & 1\tickok & 1\tickok & 0\tickno & 1\tickok & 1\tickok & 1\tickok\\
\bottomrule
\end{tabular}
\caption{T12 Reconstruct.}
\label{tab:qual_trace_t12}
\end{table}
\noindent\textbf{Thinking traces.}\par\smallskip
\begin{tcolorbox}[breakable,enhanced,colback=red!4,colframe=red!55!black,boxrule=0.4pt,arc=1pt,left=4pt,right=4pt,top=3pt,bottom=3pt,fonttitle=\footnotesize\bfseries,coltitle=black,colbacktitle=red!12,title={\tpicon{gemma_icon.png}~Gemma4-31B\hfill answer: 0\tickno}]
\footnotesize\raggedright
* Image 1: A silhouette showing a vertical column of \tann{annCol10}{3 squares}{Wrong Perception}, with one square to the right of the middle square and one square to the left of the bottom square. \newline
* \tann{annCol8}{Wait, let me re-examine Image 1:}{Reiterating} \newline
* Column 1 (leftmost): 1 square at the bottom. \newline
* Column 2 (middle): 4 squares (bottom, middle-bottom, middle-top, top). \newline
* Column 3 (rightmost): 1 square at the middle-bottom level. \newline
* \tann{annCol8}{Let's re-count:}{Reiterating} \newline
* Top row: 1 square (middle column) \newline
* Row 2: 1 square (middle column) \newline
* Row 3: 2 squares (middle and right columns) \newline
* Row 4: 2 squares (left and middle columns) \newline
* Total squares = 1 + 1 + 2 + 2 = 6 squares. \newline
* \tann{annCol8}{Wait, let me look again.}{Reiterating} \newline
\textit{[[...trimmed output...]]}\newline
% * Image 1: \newline
% * Top square: (1, 3) - using (col, row) where (0,0) is bottom-left. \newline
% * Middle-top square: (1, 2) \newline
% * Middle-bottom square: (1, 1) \newline
% * Bottom square: (1, 0) \newline
% * Right square: (2, 1) \newline
% * Left square: (0, 0) \newline
* \tann{annCol8}{Wait, let me re-examine Image 1 again.}{Reiterating} \newline
\textit{[[...trimmed output...]]}
% * Top square: (1, 3) \newline
% * Square below it: (1, 2) \newline
% * Square below that: (1, 1) \newline
% * Square below that: (1, 0) \newline
% * Square to the right of (1, 1): (2, 1) \newline
% * Square to the left of (1, 0): (0, 0) \newline
% * Total = 6 squares. \newline
% * Let's re-verify: \newline
% * Column 0: row 0 \newline
% * Column 1: rows 0, 1, 2, 3 \newline
% * Column 2: row 1 \newline
% * Total = 1 + 4 + 1 = 6.

% * Image 2: A silhouette showing a vertical column of 3 squares, with one square to the left and one square to the right of the bottom square. \newline
* \tann{annCol8}{Wait, let me re-examine Image 2:}{Reiterating} \newline
\textit{[[...trimmed output...]]}
% * Top square: (1, 2) \newline
% * Middle square: (1, 1) \newline
% * Bottom square: (1, 0) \newline
% * Left square: (0, 0) \newline
% * Right square: (2, 0) \newline
% * Total = 5 squares. \newline
% * \tann{annCol8}{Let's re-verify:}{Reiterating} \newline
% * Column 0: row 0 \newline
% * Column 1: rows 0, 1, 2 \newline
% * Column 2: row 0 \newline
% * Total = 1 + 3 + 1 = 5.

% * Image 3: A silhouette showing a stepped shape. \newline
% * Bottom row: 4 squares (0,0), (1,0), (2,0), (3,0) \newline
% * Middle row: 3 squares (1,1), (2,1), (3,1) \newline
% * Top row: 2 squares (2,2), (3,2) \newline
% * Total = 4 + 3 + 2 = 9 squares.

* \tann{annCol8}{Let's re-examine the silhouettes. Maybe I'm miscounting.}{Reiterating} \newline
\textit{[[...trimmed output...]]} \newline
% * Image 1: \newline
% * Col 0: row 0 \newline
% * Col 1: row 0, 1, 2, 3 \newline
% * Col 2: row 1 \newline
% * Total = 6 squares. \newline
% * Image 2: \newline
% * Col 0: row 0 \newline
% * Col 1: row 0, 1, 2 \newline
% * Col 2: row 0 \newline
% * Total = 5 squares. \newline
% * Image 3: \newline
% * Col 0: row 0 \newline
% * Col 1: row 0, 1 \newline
% * Col 2: row 0, 1, 2 \newline
* \tann{annCol0}{I have to give the solution based on the reasoning directly now.}{Budget Hit}
\end{tcolorbox}
\begin{tcolorbox}[breakable,enhanced,colback=red!4,colframe=red!55!black,boxrule=0.4pt,arc=1pt,left=4pt,right=4pt,top=3pt,bottom=3pt,fonttitle=\footnotesize\bfseries,coltitle=black,colbacktitle=red!12,title={\tpicon{grok_icon.png}~Grok-4.20\hfill answer: 0\tickno}]
\footnotesize\raggedright
The problem involves identifying which candidate view matches the three silhouettes of the same 3D object. \newline
I need to pick which candidate view fits the three silhouettes. The three silhouettes are projections of the same 3D object, and one candidate is consistent with all three, the other isn't.

The silhouettes are unlabeled orthographic projections, possibly showing outlines of polycubes or cube-based structures. The candidates are 3D viewsof possible objects.

To decide, I'd compare how each candidate's projections from different angles match the silhouettes. For the correct candidate, if I take its 3D structure and project it orthographically from the same directions as the silhouettes, it should match all three silhouettes exactly. The incorrect one will have at least one mismatch.

\tann{annCol10}{Since there are no actual images,}{Wrong Perception} the task is to simulate reasoning about counting cubes, analyzing shapes like L-shapes or T-shapes, counting projected areas, or reconstructing the Reasoning about candidate 0 and 1 involves visualizing their structures, counting cubes (e.g., candidate 0 has fewer cubes or asimpler shape), and checking against silhouette features like height variations, protrusions, or bar lengths.

For example, candidate 0 (image 4) appears to be a simpler cross-like structure with around 10-11 cubes, while candidate 1 (image 5) is more complex with layers and possibly more cubes. \tann{annCol3}{Candidate 1 seems to cast a taller silhouette in one direction due to its height, matching a silhouette with a tall column of 4 squares.}{Good Perception}

Candidate 0's projections don't match a silhouette with disconnected components or a specific pattern like an 'E' shape, whereas candidate 1's projections align with all silhouettes'features, such as a base of 3 squares wide and a tall middle column.

Candidate 0's projections don't match a silhouette with disconnected components or a 
\begin{CJK*}{UTF8}{mj}\colorbox{annCol6}{첫}\textsuperscript{\tiny[Misc]}\end{CJK*}
% \tann{annCol6}{첫}{Misc}
specific pattern like an 'E' shape, whereas candidate 1's projections align with all silhouettes' features, such as a base of 3 squares wide anda tall middle column.

Candidate 1 fits best because its 3D arrangement allows for the observed silhouettes when projected, accounting for occlusions and visible faces.

\tann{annCol3}{So, the correct candidate is candidate\_idx = 1.}{Good Perception}
\end{tcolorbox}
\begin{tcolorbox}[breakable,enhanced,colback=green!4,colframe=green!50!black,boxrule=0.4pt,arc=1pt,left=4pt,right=4pt,top=3pt,bottom=3pt,fonttitle=\footnotesize\bfseries,coltitle=black,colbacktitle=green!14,title={\tpicon{gpt_icon.png}~GPT-5\hfill answer: 1\tickok}]
\footnotesize\raggedright
Analyzing structure views and silhouettes \newline
I'm considering two possible candidates based on their silhouettes. Candidate0 seems to have a structure with a top row of four cubes, perhaps arranged in columns hanging down. Candidate1 looks like a 3D polycube shape, possibly fitting the third silhouette, with a different projection. I need to compare these based on their projections! \newline
Comparing candidates and projections \newline
I'm trying to break down the silhouettes to figure out how to reliably distinguish the candidates. Candidate0 seems tricky because its top row has four cubes, and it's hard to analyze the top surface directly. Candidate1 looks promising, with projections that likely align with all three silhouettes. I'll keep reasoning. \newline
Breaking down cube counts and orientations \newline
It looks like Candidate1 has a rectangular block, with visible faces showing various cubes, maybe 12 total. \tann{annCol10}{The front face shows two rows with cubes on the left, center, and right.}{Wrong Perception} Candidate0 seems to have 11 cubes in total. These figures may match the silhouettes, so I'll compare further. \newline
Clarifying silhouette projections and object alignment \newline
I've been thinking about the projections for the object. \tann{annCol3}{The silhouettes seem to match a cuboid of dimensions 3 x 3 x 4, based on their grid pairs. By aligning the dimensions, silhouette 1 is 3x4, silhouette 2 is 3x3, and silhouette 3 matches 4x3. The object seems to lie in a 4 x 3 x 3 box.}{Good Perception} \newline
Defining projections and dimensions \newline
\textit{[[...trimmed output...]]} \newline
% I've been analyzing three orthographic projections. Silhouette 1 might match the P\_ZX projection (width 3, height 4), while silhouette 2 could be P\_ZY (3x3). Candidate1 seems to fit a box of 4x3x3. I'm assigning dimensions accordingly, with X=4, Y=3, Z=3, and I plan to compare these projections for a final alignment. \newline
% Understanding projections and coordinates \newline
% I'm analyzing the x-z and y-z projections. The x-z projection shows that height along z increases with x. The silhouette2 (3 by 3) corresponds to the y-z projection with heights [1,3,1]. Whereas silhouette1, a y-x projection, shows different y values across x. I believe this configuration traces the vertical dimensions neatly. \newline
% Analyzing candidate voxel structure \newline
% I'm trying to figure out the voxel layout. The maximum candidate shape seems to be 11 voxels, with Candidate1 matching this exactly. It has a central row of cubes with increasing height (from left to right) and two additional protrusions. This fits all silhouette constraints. Looks like it's a solid candidate. \newline
% Analyzing candidate0 and silhouette projections \newline
% It's clear that Candidate1 has a stair-step profile, with its visible front-ish projection displaying varying heights across columns. Candidate0 could be an extruded shape that produces silhouettes similar to silhouette2 and silhouette1. Upon closer inspection, Candidate0 also seems to fit the voxel count---maybe 11 as well. \newline
% Exploring candidate shape and projections \newline
% Candidate0 might be a polycube with a flat top row and a central vertical column. Its projections could potentially match the silhouette views, but we need to inspect the images closely. Candidate1 is more of an actual extruded 3D shape. I'll need to visualize and compare them to confirm. \newline
Displaying candidate images for analysis \newline
\tann{annCol9}{from PIL import Image import matplotlib.pyplot as plt, os paths = [ "/mnt/data/T12\_sample1\_row33\_silhouette\_0.png", "/mnt/data/T12\_sample1\_row33\_silhouette\_1.png", "/mnt/data/T12\_sample1\_row33\_silhouette\_2.png", "/mnt/data/T12\_sample1\_row33\_candidate\_0.png", "/mnt/data/T12\_sample1\_row33\_candidate\_1.png", ] imgs=[Image.open(p) for p in paths] [img.size for img in imgs] Matplotlib is building the font cache; this may take a moment. [(409, 409), (409, 409), (409, 409), (409, 409), (409, 409)]}{Tool Use} \newline
Visualizing candidate shapes and silhouettes \newline
Output image \newline
Analyzing Candidate0's structure and projection \newline
\tann{annCol10}{Candidate0 looks like a polycube shown from a slightly tilted top view, with a 1x4 top row and vertical stacks behind it. It doesn't have a stacked height greater than 1, suggesting it's a 2D arrangement of cubes, each of height 1. From certain perspectives, it may appear taller, but projections likely won't match silhouettes that require 3D height.}{Wrong Perception} \newline
\tann{annCol10}{Understanding Candidate0's projections and height mismatch Candidate0 appears to be a flat arrangement with unit-height blocks, so its projections along horizontal axes would have a max height of 1, which doesn't match the silhouettes requiring heights of 2 or 3.}{Wrong Perception} Candidate1, however, has stacks with heights of 2-3, which fits the silhouette's needs.

```json \newline
\{ \newline
'candidate\_idx': 1, \newline
\} \newline
```
\end{tcolorbox}
\begin{tcolorbox}[breakable,enhanced,colback=green!4,colframe=green!50!black,boxrule=0.4pt,arc=1pt,left=4pt,right=4pt,top=3pt,bottom=3pt,fonttitle=\footnotesize\bfseries,coltitle=black,colbacktitle=green!14,title={\tpicon{gemini_flash_icon.png}~Gemini-3-Flash\hfill answer: 1\tickok}]
\footnotesize\raggedright
To identify the correct 3D object, we analyze the provided silhouettes as the Top, Front, and Side views of a single structure and then compare them against the candidate views.

\#\#\# 1. Silhouette Analysis

* **Silhouette 0 (Side View):** Shows a "J" or "L" shape with a vertical height of 4 units and a base width of 3 units. \newline
* **Silhouette 1 (Front View):** Shows a "T" or inverted "T" shape with a width of 3 units and a height of 3 units. \newline
* **Silhouette 2 (Top View):** Shows a 4x3 footprint with a "stair-step" profile, indicating varying depths/heights across the grid.

\#\#\# 2. Candidate Evaluation

\tann{annCol3}{* **Candidate 0:** This image shows a collection of cubes arranged in a flat, staggered layout. Looking at the depth and the vertical alignment, it lacks the specific 4-unit vertical column required by Silhouette 0. The proportions and the way the cubes are joined do not create the consistent "T" shape seen in Silhouette 1. * **Candidate 1:** This 3D representation accurately captures the dimensions. It features a central vertical spine that matches the height requirements and lateral protrusions that correspond to the "T" shape in Silhouette 1 and the specific footprint seen in the Top View (Silhouette 2). The perspective view confirms the relative positions of the cubes are consistent with all three projections.}{Good Perception}

\#\#\# 3. Conclusion

Candidate 1 is the only object whose geometry aligns perfectly with the provided silhouettes.

```json \newline
\{ \newline
"candidate\_idx": 1 \newline
\}

```
\end{tcolorbox}
\begin{tcolorbox}[breakable,enhanced,colback=green!4,colframe=green!50!black,boxrule=0.4pt,arc=1pt,left=4pt,right=4pt,top=3pt,bottom=3pt,fonttitle=\footnotesize\bfseries,coltitle=black,colbacktitle=green!14,title={\tpicon{gemini_pro_icon.png}~Gemini-3.1-Pro\hfill answer: 1\tickok}]
\footnotesize\raggedright
Analyzing Silhouettes' Features

I am now closely examining the silhouette details, noting square arrangements and overall geometry to clarify.

Defining Block Coordinates

I've accurately mapped block coordinates for each silhouette, ready to find relationships between arrangements.

\textit{[[...trimmed output...]]}

% Determining Silhouette Relationships

% I've determined possible view directions and object dimensions, finding inconsistencies to resolve and model.

% Revising Projection Assumptions

% I've re-examined the projections, now considering S0, S1, and S2 as potential Top, Front, and Side views.

% Reassessing View Orthogonality

% I'm now reconsidering the orthogonality of views and re-evaluating perspective, seeking dimensions clarification.

% Clarifying S2's View

% I've determined that a 4x3 Side view doesn't align with S2, and now reassessed object depth.

% Mapping Candidate Features

% I've begun mapping and carefully tracing the visible faces of Candidate 1 to understand its 3D structure.

% Matching Silhouette Structure

% I've now mapped Candidate 1's features, recognizing its staircase-like arrangement, using (x,y,z) coordinates.

% Analyzing Candidate 0

% I'm now counting faces in Candidate 0's top view, finding a match for S0's detailed silhouette features.

% Matching Candidate 0

% I've determined Candidate 0's orientation, matching Silhouette 0's top view precisely.

% Verifying Candidate Alignment

% I've precisely assessed Candidate 0, discovering it doesn't align by simple rotation, requiring a horizontal reflection to match S0.

% Re-evaluating Candidate 0's View

% I've determined Candidate 0's orientation is isometric, where the 'top' could actually be front faces.

% Confirming Isometric Cues

% I've determined Candidate 0's view, matching it to the provided silhouettes and its shape matches S0.

Confirming Candidate Structure

\tann{annCol3}{I've determined Candidate 1's top view matches Silhouette 1, an inverted 'T', confirming the top face arrangement. }{Good Perception} \newline
Verifying Face Orientations

I've determined Candidate 1 has a 3x3 grid of down-left faces, now mapping their coordinates precisely.

Matching Silhouette Coordinates

I've confirmed the isometric coordinates match Silhouette 1's T-shape, including block counts and face arrangements.

Tracing Block Heights

I've precisely assessed and validated block heights based on visible faces within Candidate 1's isometric view.

Verifying Wall Structure

I'm now carefully re-verifying block arrangements to match +Y faces, precisely defining coordinates to resolve the T/L-shape discrepancy.

Revising Candidate Zero

\tann{annCol10}{Candidate 0's top view precisely matches Silhouette 0's arrangement, verifying its orientation completely. }{Wrong Perception} \newline
Revising Block Orientations

\tann{annCol3}{I've re-examined and confirmed Candidate 0's projections, discovering its distinct shape fundamentally differs from S0's.}{Good Perception}

Mapping Face Connections

I've precisely traced faces, verifying the L-shape of the top view and connection rules.

Validating Block Heights

I've determined block heights for the left column, including visibility and precise square counts for faces.

Verifying Wall Heights

I've determined block heights precisely, meticulously re-checking +Y faces, confirming Candidate 1's stepped configuration.

Reassessing Candidate Shape

\tann{annCol10}{I've determined Candidate 1 is an L-shape in its top view, and concluded it cannot be the object, so I'm re-evaluating Candidate 0. }{Wrong Perception} \newline
Interpreting Viewpoints

I've determined Candidate 0 represents a front, bottom, right view, matching S0's 6-block configuration after carefully re-examining the silhouette features.

Verifying Object Edges

I've determined S0's exact block layout and edge features, precisely mapping block coordinates.

Revising Candidate Alignments

\tann{annCol3}{I've determined Candidate 0 cannot match Silhouette 0 in any perspective; also, the correct structure of Candidate 1 is now clear. }{Good Perception} \newline
Verifying +X Wall Visibility

I've determined that +X face visibility is affected by relative block Y coordinates, resolving occlusion and re-assessing Candidate 1.

Verifying Connectivity Rules

I've precisely assessed block arrangement and verified their adjacency, accurately determining (1,2) for D's location.

Revising Block Configuration

\tann{annCol3}{I've determined Candidate 0 doesn't match a one-block-thick projection of S0, and I'm reconsidering its internal block arrangements. }{Good Perception} \newline
Revising Candidate Alignments

I've determined Candidate 0's Front, Side views are impossible and confirmed the cross/T shape, so I will now completely re-evaluate the block configurations of Candidate 1.

\textit{[[...trimmed output...]]}

% Clarifying Wall Locations

% I've determined that the vertical alignment of blocks C and D is a result of their isometric projection.

% Interpreting Candidate Walls

% I've determined that blocks D and E have a contiguous left-facing wall, due to their shared Y coordinate and adjacent placement.

% Confirming Block Heights

% I've precisely calculated block heights and face visibility, verifying the isometric projections for the final block arrangement.

% Validating Block Heights

% I've precisely assessed B's height, confirming it's 3, matching a continuous top surface.

% Calculating Final Silhouettes

% I've precisely calculated all three silhouettes based on Candidate 1's confirmed block arrangement.

% Revising Object Orientation

% I've determined Candidate 0 could match S0 as its right view, starting to find the object's correct depth.

% Revising Height Assumptions

% I've determined Candidate 0 represents front, top and right faces; Candidate 1 may match Silhouette 0.

Reassessing Candidate Blocks \newline
\tann{annCol10}{ I've determined Candidate 1 cannot be the object, and I will now carefully investigate if its absence creates an "inverse" object.}{Wrong Perception}

Validating Tetromino Alignment

\tann{annCol3}{I've determined Candidate 0 represents the Z-tetromino mirror image, so I'm now re-validating Candidate 1 as the correct object. }{Good Perception} \newline
Revising Coordinate Perspective

\tann{annCol3}{I've determined Candidate 0 doesn't match S0 regardless of perspective, focusing on Candidate 1's dimensions. }{Good Perception} \newline
Confirming Isometric Projection

\tann{annCol3}{I've determined Candidate 1's T-shape top view aligns perfectly with S1, so I'm now verifying if Candidate 1 can produce the S0 and S2 silhouettes. }{Good Perception} \newline
Revising Block Configuration

\tann{annCol3}{I've determined Candidate 0 represents an S-shape and now re-verified Candidate 1 as a positive, complete, solution.}{Good Perception}

Confirming Silhouette Resolution

\tann{annCol3}{I've definitively classified Candidate 0 as negative, and Candidate 1 as positive, using logical elimination, and focusing on shape mismatches.}{Good Perception}

```json \newline
\{ \newline
"candidate\_idx": 1 \newline
\}

```
\end{tcolorbox}

\subsubsection{T13 Mixture-of-Shapes}
\begin{table}[H]
\centering
\footnotesize
\setlength{\tabcolsep}{1pt}
\renewcommand{\arraystretch}{1.2}
\begin{tabular}{*{9}{>{\centering\arraybackslash}p{\dimexpr\textwidth/9-2\tabcolsep\relax}}}
\toprule
\multicolumn{9}{@{}l@{}}{\itshape ``\ldots{}Your task is to identify the invalid silhouette\ldots{}''}\\[0.3mm]
\multicolumn{9}{@{}c@{}}{\begin{tabular}{*{5}{c}}\includegraphics[width=0.180\textwidth,height=1.25in,keepaspectratio]{images/app_qual_traces/T13_sample1_row52_query_image_1.png} & \includegraphics[width=0.180\textwidth,height=1.25in,keepaspectratio]{images/app_qual_traces/T13_sample1_row52_query_image_2.png} & \includegraphics[width=0.180\textwidth,height=1.25in,keepaspectratio]{images/app_qual_traces/T13_sample1_row52_candidate_0.png} & \includegraphics[width=0.180\textwidth,height=1.25in,keepaspectratio]{images/app_qual_traces/T13_sample1_row52_candidate_1.png} & \includegraphics[width=0.180\textwidth,height=1.25in,keepaspectratio]{images/app_qual_traces/T13_sample1_row52_candidate_2.png}\end{tabular}}\\[0.5mm]
\textbf{GT} & \tpicon{qwen_icon.png} & \tpicon{gemma_icon.png} & \tpicon{glmv_icon.png} & \tpicon{kimi_icon.png} & \tpicon{grok_icon.png} & \tpicon{gpt_icon.png} & \tpicon{gemini_flash_icon.png} & \tpicon{gemini_pro_icon.png}\\
1 & 2\tickno & 0\tickno & 2\tickno & 2\tickno & 2\tickno & 0\tickno & 2\tickno & 1\tickok\\
\bottomrule
\end{tabular}
\caption{T13 Mixture-of-Shapes.}
\label{tab:qual_trace_t13}
\end{table}
\noindent\textbf{Thinking traces.}\par\smallskip
\begin{tcolorbox}[breakable,enhanced,colback=red!4,colframe=red!55!black,boxrule=0.4pt,arc=1pt,left=4pt,right=4pt,top=3pt,bottom=3pt,fonttitle=\footnotesize\bfseries,coltitle=black,colbacktitle=red!12,title={\tpicon{qwen_icon.png}~Qwen3.5-27B\hfill answer: 2\tickno}]
\footnotesize\raggedright
The user wants me to identify the invalid 2D silhouette from three candidates, based on two perspective views of a 3D scene.

**1. Analyze the Perspective Views:**

* **View 1 (Top Left):** \newline
* I see a collection of cylindrical objects. \newline
* There's a tall stack of cylinders in the back left. Wait, let's look closer. It looks like a stack of two cylinders on top of each other, slightly offset. No, actually, looking at the top view, it looks like a stack of cylinders. Let's count. \newline
* Let's look at the objects individually. \newline
* Object 1: Far left, lying on its side. \newline
* Object 2: Below Object 1, smaller, lying on its side. \newline
* Object 3: Center-left, lying on its side. \newline
* Object 4: Top center, lying on its side. \newline
* Object 5: Center, standing upright (short cylinder). \newline
* Object 6: Bottom right, lying on its side. \newline
* Object 7: Far right, lying on its side. \newline
* \tann{annCol8}{Wait, let's re-evaluate the shapes. They all look like cylinders with ridges.}{Reiterating} \newline
* Let's look at the arrangement. \newline
* There is a cluster in the middle. \newline
* Let's look at the second view to clarify.

* **View 2 (Top Right):** \newline
* This view shows the same objects from a different angle. \newline
* Top left: A cylinder lying on its side. \newline
* Bottom left: A cylinder lying on its side. \newline
* Bottom center: A cylinder lying on its side. \newline
* Center: A short cylinder standing upright. \newline
* Top right: A cylinder lying on its side. \newline
* Bottom right: Two cylinders lying on their sides, stacked or close together. \newline
* Let's try to map the objects. \newline
* It seems there are roughly 7-8 objects. \newline
* Let's look at the "standing" object. In View 1, there is a short cylinder standing upright in the center. In View 2, there is a short cylinder standing upright in the center-right. \newline
* \tann{annCol8}{Let's look at the "lying" objects.}{Reiterating} \newline
\textit{[[...trimmed output...]]}
% * View 1: \newline
% * Far left: Lying cylinder. \newline
% * Below it: Smaller lying cylinder. \newline
% * Center left: Lying cylinder. \newline
% * Top center: Lying cylinder. \newline
% * Far right: Lying cylinder. \newline
% * Bottom right: Lying cylinder. \newline
% * Center: Standing short cylinder. \newline
% * View 2: \newline
% * Top left: Lying cylinder. \newline
% * Bottom left: Lying cylinder. \newline
% * Bottom center: Lying cylinder. \newline
% * Center right: Standing short cylinder. \newline
% * Top right: Lying cylinder. \newline
% * Bottom right: Two lying cylinders.

* \tann{annCol8}{Let's count again.}{Reiterating} \newline
\textit{[[...trimmed output...]]}
% * View 1: \newline
% 1. Far left (lying) \newline
% 2. Below far left (lying, smaller) \newline
% 3. Center left (lying) \newline
% 4. Top center (lying) \newline
% 5. Center (standing) \newline
% 6. Bottom right (lying) \newline
% 7. Far right (lying) \newline
% Total: 7 objects.

% * View 2: \newline
% 1. Top left (lying) \newline
% 2. Bottom left (lying) \newline
% 3. Bottom center (lying) \newline
% 4. Center right (standing) \newline
% 5. Top right (lying) \newline
% 6. Bottom right (lying) \newline
% 7. Bottom right (lying, slightly behind/above the previous one) \newline
% Total: 7 objects.

% * Wait, let's look at the "standing" object. In View 1, it's a short cylinder. In View 2, it's a short cylinder. \newline
% * Let's look at the "lying" objects. They are all cylinders with ridges. \newline
% * Let's look at the silhouettes.

% **2. Analyze the Candidate Silhouettes:**

% * **Silhouette 1 (Middle Left):** \newline
% * Left side: A tall stack of horizontal lines (looks like a stack of flat objects or a cylinder seen from the side with ridges). Next to it, a smaller stack of vertical lines. \newline
% * Right side: A tall stack of horizontal lines. Next to it, a large circle. \newline
% * This looks like a side view. \newline
% * The "tall stack of horizontal lines" corresponds to a cylinder lying on its side, seen from the side (showing the ridges). \newline
% * The "large circle" corresponds to a cylinder seen from the end (top/bottom face). \newline
% * Let's try to map this to the 3D scene. \newline
% * If we look from the front (orthographic), we might see: \newline
% * A cylinder lying on its side -> Rectangle with horizontal lines. \newline
% * A cylinder standing up -> Circle. \newline
% * In Silhouette 1: \newline
% * Left part: A tall rectangle with horizontal lines. This implies a long cylinder lying horizontally. \newline
% * Next to it: A smaller rectangle with vertical lines. This implies a cylinder lying horizontally but seen from a different angle? Or maybe a stack of flat things? No, the ridges are vertical. This implies a cylinder lying on its side, but the ridges are vertical? No, if a cylinder lies on its side, the ridges (if longitudinal) would be horizontal. If the ridges are circumferential (like a thread), they would be vertical if seen from the side? No, circumferential ridges would look like lines across the face. Longitudinal ridges look like lines along the length. \newline
% * Let's assume the ridges are longitudinal (like a ribbed cylinder). \newline
% * If a cylinder lies on its side, we see a rectangle with horizontal lines. \newline
% * If a cylinder stands up, we see a circle (top face) and maybe the side if it's tall. If it's short, just a circle. \newline
% * In Silhouette 1, there is a large circle on the right. This matches the standing cylinder. \newline
% * There are stacks of rectangles. \newline
% * Let's look at the arrangement. \newline
% * Left group: Tall horizontal stack, small vertical stack. \newline
% * Right group: Tall horizontal stack, large circle. \newline
% * This implies two main clusters.

% * **Silhouette 2 (Middle Right):** \newline
% * Top left: Rectangle with horizontal lines. \newline
% * Below it: Small rectangle with vertical lines. \newline
% * Center: Large rectangle with vertical lines. \newline
% * Top right: Rectangle with vertical lines. \newline
% * Bottom center: Circle. \newline
% * Bottom: Rectangle with vertical lines. \newline
% * This looks like a top-down view or a front view. \newline
% * The circle is at the bottom. This matches the standing cylinder being at the "bottom" of the view. \newline
% * The rectangles represent the lying cylinders. \newline
* Let's count the rectangles. \newline
1. Top left (horizontal lines) \newline
2. Below it (vertical lines) \newline
3. Center (vertical lines) \newline
4. Top\tann{annCol0}{I have to give the solution based on the reasoning directly now.}{Budget Hit}
\end{tcolorbox}
\begin{tcolorbox}[breakable,enhanced,colback=red!4,colframe=red!55!black,boxrule=0.4pt,arc=1pt,left=4pt,right=4pt,top=3pt,bottom=3pt,fonttitle=\footnotesize\bfseries,coltitle=black,colbacktitle=red!12,title={\tpicon{grok_icon.png}~Grok-4.20\hfill answer: 2\tickno}]
\footnotesize\raggedright
The problem involves identifying which silhouette doesn't match the two perspective images of the 3D scene. \newline
\textit{[[...trimmed output...]]}
% The task is to find which of the three candidate 2D orthographic silhouettes doesn't match the two given perspective images of the same 3D scene. The scene includes multiple 3D objects like cylinders with striped sides, possibly batteries or ribbed cylinders, arranged together. From the perspective views, I see several cylinders 10 cylinders? No, counting mentally: there are cylinders of varying heights and sizes, some tall and slender, others short and wide, positioned in clusters.

% In the first perspective, there are clusters of striped cylinders, gray tops indicating they are upright, and shapes like disks if viewed edge-on. The silhouettes are supposed to 10 match the outline when viewed orthographically from a specific direction, but one candidate has an altered object, making its silhouette different.

To identify the mismatch, I need to infer the 3D arrangement from the two perspectives. The perspectives show the cylinders standing upright with striped sides and gray ends. Counting objects: around there are about 7-8 cylinders in visible positions, arranged in rows or clusters.

The candidates are labeled as silhouettes, and one has an extra shape or altered form. \tann{annCol10}{The candidate with the mismatched silhouette is candidate\_idx 2, because it shows a shape that doesn't align with the counted objects or their relative sizes in 3D space.}{Wrong Perception} For example, candidate 0 has matching stacks of rectangles with stripes and circles for tops, \tann{annCol10}{candidate 1 has similar but with an extra circle}{Wrong Perception}, candidate 2 has an oval attached in a way that suggests a different arrangement or added object.

\tann{annCol10}{Upon closer inspection, candidate\_idx 2 stands out because it 2 includes a standalone circle not attached to any striped rectangle, whereas the others have circles attached or positioned consistently with cylinder tops. This standalone circle indicates an extra sphere or altered cylinder that isn't in the perspective views. So, the final answer is the second candidate, index 2. \{ 'candidate\_idx': 2 2, \} ``` Wait, syntax error, let's correct it. \{ 'candidate\_idx': 2, \} ``` }{Wrong Perception}

\tann{annCol5}{But wait, the internal reasoning is truncated and incomplete,}{Harnessing} but focusing on the core: the mismatch is due to an extra standalone circle in candidate 2, which doesn't match the scene's objects.

The striped parts are rectangles representing side views of cylinders, and gray parts are circles for ends if visible.

\tann{annCol10}{In the scene, all cylinders are upright, no standalone spheres. Hence, candidate 2 is invalid. }{Wrong Perception}

Yes, that seems plausible based on the trace.

So, my final answer is the second 2 candidate, index 2.

\{ \newline
'candidate\_idx': 2, \newline
\} \newline
``` Wait, the trace says the fourth image, but indices are 0,1,2 for the three candidates.

Assuming the third image is 0, fourth is 1, fifth is 2.

The trace mentions the fourth image has the standalone circle, so if candidates are 0: third, 1:
\begin{CJK*}{UTF8}{gbsn}\colorbox{annCol6}{ 第四}\textsuperscript{\tiny[Misc]}\end{CJK*}
% \tann{annCol6}{ 第四}{Misc}
, 2: fifth, then index 1.

\tann{annCol5}{The trace says "the fourth image has a circle and several rectangular striped things", and "the fifth image has three groups with gray oval or circle next to or overlapping striped rectangle". The trace concludes the fifth is like lying cylinders, but the scene has upright ones upright. The trace says "candidate 2 is invalid" in my summary, but let's map. The trace says "the fourth image", which is the first candidate? Let's assume the images are numbered 1,2 (perspectives), then 3,4,5 as candidates, so candidate\_idx 0 for 3, 1 for 4, 2 for 5. }{Harnessing} \newline
The trace says the fourth has the ball, and the scene has no ball, so the one with the standalone circle is invalid.

So, the fourth image is candidate 1.

But in my previous thought, I said candidate 2.

\textit{[[...trimmed output...]]}

% I need 10 to decide which one is the odd one out.

% The problem is to find the one that corresponds to a scene with one object altered.

% So, the silhouettes must match the outline of the 3D arrangement.

% From the two perspectives, the scene has no standalone sphere, all are cylinders, some short ones look like 11 disks, but no circle without stripes.

% In candidate 1 (fourth image), there is a gray circle in the middle bottom, which is not consistent with the perspectives, as there is no such standalone circle.

% Whereas candidate 0 and 2 have only striped cylinders with attached shapes, but the circle is extra.

% 11 The striped parts are rectangles because they are side views of cylinders, but in orthographic, cylinders project to rectangles if upright, but if lying down, circles.

The cylinders seem upright, stripes vertical, so silhouette would be rectangle with circle ends if ends are visible, but in drawing it's simplified.

\tann{annCol5}{The trace cuts off 11 but I think the odd one is candidate 2, because it has a circle that doesn't match. The trace says candidate\_idx': 2, }{Harnessing} \newline
\tann{annCol10}{So, I think the answer is candidate 2. }{Wrong Perception} \newline
\tann{annCol7}{But the trace is incomplete, but the example is candidate\_idx': 2,}{Prior Bias}

So, I'll go with that. 11

\tann{annCol5}{But the trace says the fifth one is inconsistent because it shows all objects as horizontal cylinders, while in perspective they are upright. The trace cuts off at "The first image has all cylinders oriented with their axis in different directions" }{Harnessing} \newline
So, the cylinders are in various orientations, some horizontal, some vertical.

The silhouettes 11 show different configurations.

\textit{[[...trimmed output...]]}

% The third one has mixed, with large circle which might be a large flat or sphere.

% The fourth one looks like all standing or boxes with one ball.

% The fifth one has three separate lying cylinders.

% So, the invalid one is the one that doesn't match the arrangement.

% But to find which one 11 has an altered object.

% The problem says "one object has been altered"

% So, the silhouette that shows a different configuration, meaning one object is in a different position or orientation.

% From the trace, it seems the fifth one is the odd one because it shows all lying, while others have mixed.

% But the trace 11 is incomplete.

% Since the trace is truncated, I need to focus on core ideas.

% The key is to compare the visible features in the silhouettes to the perspective views.

% In the perspectives, there are striped cylinders, some with horizontal stripes (horizontal cylinders?), some with vertical (vertical cylinders).

% In the fourth silhouette, there 11 is a plain gray circle without stripes, while others have stripes.

% But earlier the trace says there are plain gray spheres.

% The trace says the fourth has a plain gray circle without stripes, but the perspectives have plain gray as spheres.

% But all candidates have that.

% The trace says in fourth: striped cylinders or boxes? 11 and one sphere.

% The fifth has gray as ends of cylinders if lying.

% So, the odd one is the fifth, because it shows cylinders lying down, which isn't in the perspectives.

% The trace suggests the fourth might be the one with all vertical striped.

% But the trace is cut off.

% Since the problem is to 11 find the one that differs by having an altered object.

% The output is to choose the candidate\_idx: 0,1,2 for the third, fourth, fifth images.

% Assuming the candidates are indexed 0 for third image, 1 for fourth, 2 for fifth.

% The trace says the fifth has all 12 horizontal, while perspectives have mix.

% So, the fifth is the one that doesn't match because it assumes all cylinders are horizontal, but the scene has both orientations.

% The fourth and third have vertical ones.

% The trace says the third has striped vertical, with heights, and circles that could be spheres or ends of horizontal cylinders 13 viewed from side.

% The fourth has more objects, 6, closer to the 7-8 in perspectives.

% The fifth has fewer.

% So, the fifth is the odd one out because it has fewer objects and different arrangement.

% The problem says one candidate has an altered object, so the silhouette is different because one 3D object is changed.

% So, the silhouette that shows a different configuration, like missing an object or altered shape.

% From the trace, the fifth has gray ovals and circles, which might not match the striped cylinders.

The trace says the fifth has gray ovals, which could be the gray tops or bottoms.

The trace cuts off, but the idea is to find the one that doesn't fit.

\tann{annCol7}{Based on the internal reasoning, the candidate\_idx is 2, as in the example. No, the example is 2, but that's just example.}{Prior Bias}

The trace mentions the fifth image, which is candidate 2 if 0, 1, 2 for third, fourth, fifth.

\textit{[[...trimmed output...]]}

% Let's assume the candidates are numbered 0 for third, 1 for fourth, 2 for fifth.

% The trace says the fifth one has three gray circles, which is different.

% So, the invalid one is the fifth, candidate\_idx: 2

% But the 3rd candidate is the third image, which is candidate 0.

% Let's clarify.

% The problem says three candidate silhouettes, probably labeled as 0,1,2.

% The trace says the third image (first candidate) looks like stacked, but the scene has no stacking.

% So, the first candidate shows stacking, but 3D scene has no stacking, so it's invalid.

% The trace says "the right also has stacked look: the striped look like two heights, with the large circle next to it."

% But then "if the original scene doesn't have stacks, then this could be the one"

% And "in the perspectives, are they stacked 3D objects stacked? From the views, they seem all on the ground, no obvious stacking."

% So, the silhouette that shows floating or stacked objects is the invalid one.

% The trace concludes with the fourth image has floating parts, so perhaps candidate 1.

% The trace says "the fourth image has the floating parts", 10 and "that matches the description of having a striped rectangle at top left not touching bottom".

% So, the fourth is the invalid one.

% Since the candidates are the third, fourth, fifth images, so candidate\_idx 0 for third, 1 for fourth, 2 for fifth.

% So, the invalid is the 10 fourth, which is candidate\_idx 1.

But the trace says "the fourth one has a small striped at top left not touching any bottom".

Yes, and the others are grounded.

And the fourth is a top-down view, but the problem is to find the one that differs, and the problem says "one 10 object has been altered".

\tann{annCol3}{So, the fourth has an altered object that's floating, while others are not. Hence, candidate\_idx: 1}{Good Perception}

\tann{annCol7}{But the example is \{ 'candidate\_idx': 2, \}, so for the fifth.}{Prior Bias}

But in my reading, the trace points to the fourth.

Let's see the trace 15 again.

The trace discusses the fifth as all lying cylinders, but perspectives have both standing and lying.

So the fifth (candidate 2) assumes all are lying, but there are standing ones, so it's invalid.

Yes, that seems the key point.

The trace says "the fifth has all three "objects" 20 like lying cylinders with oval ends, while perspectives show some with tops up.

\tann{annCol10}{So yes, invalid is candidate 2. And the other two are consistent: one with upright rectangles (standing cylinders) and circles (ends or spheres), and another with circles and rectangles.}{Wrong Perception}

Yes.
\end{tcolorbox}
\begin{tcolorbox}[breakable,enhanced,colback=red!4,colframe=red!55!black,boxrule=0.4pt,arc=1pt,left=4pt,right=4pt,top=3pt,bottom=3pt,fonttitle=\footnotesize\bfseries,coltitle=black,colbacktitle=red!12,title={\tpicon{gpt_icon.png}~GPT-5\hfill answer: 0\tickno}]
\footnotesize\raggedright
Identifying silhouette discrepancies in perspective images \newline
I need to determine which silhouette doesn't match the other two. I'll analyze the two perspective images and figure out which candidate's silhouette is mutated. The scene includes various objects like cubes, cuboids, cylinders, wedges, and prisms---each seen in multiple orientations---but one doesn't fit. Let's break this down visually. \newline
\textit{[[...trimmed output...]]} \newline
% Analyzing perspective 2 scene and silhouette candidates \newline
% In this second perspective, I see a cylindrical striped object at the lower right and several boxes arranged at the left. There's an isolated cube in the middle-right. The silhouettes to consider show overlapping objects, and I need to figure out which one doesn't fit based on their orientation and perspectives. \newline
% Clarifying cylinder details in candidate silhouettes \newline
% I'm wondering if both the oval and striped rectangle could be the same cylinder, since only one striped cylinder is shown in the perspective images. Candidate 0 shows a striped rectangle with an ellipse above it, which might represent the cylinder's circular face seen from the top. Could this be the same cylinder? \newline
% Dissecting the cylinder's appearance across perspectives \newline
% The perspective views show the striped cylinder lying horizontally, not vertically, which suggests the top is a rectangle when viewed perpendicularly. Candidate 2 shows an oval and a striped rectangle, possibly pointing to two separate objects. Maybe the oval is the smooth face of the same striped cylinder, projected from the side in Candidate 0? \newline
% Clarifying the striped features and shapes in the scene \newline
% I'm analyzing the striped features in the scene. It seems there are two striped objects---one a striped cylinder seen at the bottom-left in perspective 1 and bottom-right in perspective 2, and another, a striped cuboid or rectangle. Candidates show both a striped rectangle (likely the central cuboid) and a smooth ellipse (cylinder end). \newline
% Reevaluating cylinder and stripe placements in candidates \newline
% In perspective 1, the striped cylinder at the bottom-left is separated, not connected. Candidate 1's vertical stripe could represent the cylinder from the top. Candidate 0's horizontal stripes might be the cylinder, but the central striped cuboid remains unclear. I'll consider each silhouette's projection and alignment. \newline
% Clarifying objects and candidate silhouettes \newline
% There seem to be multiple objects: a striped wedge/ramp and a striped cylinder. The silhouette candidates seem to represent this: Candidate 1 shows two striped rectangles, likely corresponding to the ramp and cylinder side-view. Candidates 0 and 2 could show the same cylinder but from different angles, with the cylinder's end being oval. \newline
% Analyzing candidate views and orthogonal projections \newline
% With one cylinder, the view depends on its alignment: it appears elliptical in one direction (e.g., front/top) and rectangular in others (side view). Candidates 0 and 2 seem to show oval shapes, which could correspond to the cylinder's circular cap. I'll need to figure out which view matches the real scene and check three 2D silhouettes based on different perspectives: front, top, and side. \newline
% Analyzed image \newline
% Output image \newline
% Analyzed image \newline
% Output image \newline
% Analyzed image \newline
% Output image \newline
% Analyzed image \newline
% Output image \newline
% Analyzed image \newline
% Output image \newline
% Identifying the invalid candidate silhouette \newline
% To solve this, I need to match the object positions from the perspectives and candidates, using the given shapes. The scene features a hatched cylinder and a cluster of boxes. By analyzing the two perspective images and the three silhouette candidates (top, front, side), I need to identify which silhouette is invalid. Let's carefully match positions and geometries. \newline
% Identifying and characterizing the shapes \newline
% The scene includes a rectangular cuboid, smaller cube, hatched wedge, and a potential wedge/roof shape. These objects are arranged in different configurations across the two queries. The silhouettes suggest some wedges may appear as rectangles or triangles. I'll need to analyze these shapes and the candidate views to identify which fit together. \newline
% Analyzing Candidate2's structure \newline
% Candidate1 shows a slight touch between the top and central cubes, suggesting a valid connection. Candidate2 looks like a front or side view, showing a striped wedge and a horizontal box row, including a cylinder end view. The top cube might be hidden behind the objects in the row. \newline
% Evaluating Candidate0 and Candidate2 validity \newline
% Candidate2 might be valid, showing a row of four rectangles that could represent cubes at the bottom, aligning well with the shapes. Candidate0, however, places the cylinder above the central boxes, which conflicts with perspective views, suggesting it could be invalid due to inconsistency. \newline
% Exploring vertical position in candidate views \newline
% For orthographic views, vertical might not always align with actual height depending on the projection angle. Candidate0 positions the cylinder above the boxes, but it aligns differently in perspective views. The candidates could represent arbitrary orthographic silhouettes from random angles, not always fixed to specific axes. \newline
% Analyzing 2D orthographic silhouettes and views \newline
% The prompt specifies 2D orthographic silhouettes, so I'm considering possible camera angles around the scene. Candidate1 seems to be a top-down view (floor plan), while Candidates0 and 2 appear to be side/front elevations. The task likely involves three arbitrary orthographic projections, two valid and one invalid. \newline
% Analyzing candidate1's top view and projections \newline
% I see that candidate1 has a top view where cubes and boxes are arranged somewhat differently compared to query1, with slight shifts in positioning. If candidate1 is valid, I'm wondering how the side/front projections might look, especially considering height. The striped vertical rectangle could be a ramp, cylinder, or box with height. \newline
% Examining candidate2 and candidate0 proposals \newline
% Candidate2 shows a striped rectangle above the right box, with the cylinder placed lower on the ground. Candidate0, however, places the striped rectangle at the center and overlaps the central cube. I also note the cylinder could be an oval in candidate0's side view, but it shouldn't be high. \newline
% Questioning candidate0 and candidate1 perspectives \newline
% Candidate0 might show a top view, but there are inconsistencies. It shows a cylinder oval, which suggests a vertical cylinder's footprint rather than a horizontal one. The oval lacks the expected length and stripes, indicating it's more likely a vertical cylinder viewed from above, not horizontal. \newline
% Understanding candidate views and cylinder shape \newline
% The query shows a horizontal cylinder, so candidate0 is probably not a top view. Candidate2's ellipse seems to match an end-on view of the cylinder, while candidate1's vertical striped rectangle fits the side view or footprint. I'm still unsure about candidate0---it might be showing a side, but the oval shape could be something else, like a smooth vertical cylinder. \newline
% Analyzing possible cylinders and shapes in query \newline
% In query1, I see a striped cylinder with an oval cap, and there's possibly a smooth cylinder/ellipsoid with a circular edge near the bottom center. If it's a smooth cylinder, candidate0's large smooth ellipse might be its side or top, while candidate2's ellipse could represent it as well. The prompt mentions multiple cylinders, and the central gray object could be a cylinder or sphere. \newline
% Refining candidate identification based on perspectives \newline
% Candidate2's smooth oval on the left could match a smooth cylinder, while Candidate1 lacks a smooth oval, possibly hidden or projected as a square from a top/side view. Both Candidate0 and Candidate2 show a smooth oval and a striped rectangle. For Candidate1, the two striped rectangles may still indicate a valid setup if the smooth cylinder overlaps with the central cube in the top view. \newline
% Identifying potential silhouettes in the images \newline
% In image1, the central curved black outline on the left of the striped slab appears as a quarter ellipse, possibly from a cylinder. Image2 shows a curved edge, potentially with a diagonal line instead of a curve. Candidate0 seems to correspond to a smooth cylinder's projection. Candidate1 lacks a smooth cylinder, potentially behind the central section. To identify the correct configuration, I'll try inferring arrangement and comparing silhouettes using perspective images and line detection. \newline
% Planning for visual reconstruction \newline
% I'm considering using a tool like Blender to represent grey shapes and work with candidates based on orthographic projections. The dataset might provide clues, though filenames seem unhelpful for this. I'll need to perform a detailed visual reconstruction, focusing on surfaces in Q1 at high zoom to identify hidden objects. \newline
% Evaluating silhouette and projection candidates \newline
% Output image \newline
% Identifying components in Image2 \newline
% In Image2, the right cube appears isolated, and there's no central cube. Instead, the central large cube from Image1 seems to be a tall rectangle in Image2. Let's break down the components by positions: \newline
% Left cube (B) and central cube (A) are visible, with the right cuboid (C) hidden partially. \newline
% A diagonal striped prism (E) sits between cubes A, D, and C. \newline
% A smooth cylinder (F) is behind these objects. \newline
% G is a striped cylinder at the bottom-left. \newline
% Identifying components in Query2 \newline
% The central-right object is likely the right cuboid (C) from Query1, viewed as a cube and separated. The top-back rectangular cuboid might be either the left cube or the central large cube. The sloped box could be the central large cube, and the front cube is located near the bottom. The striped piece and the cylinder help define the main cluster's positions. The smooth cylinder from Query1 \newline
% Analyzing candidate projections \newline
% The image features a large rectangle with a striped object above it, possibly a striped cylinder or prism behind the central cube in projection. The left ellipse could be the smooth or striped cylinder seen head-on. In Candidate0, the layout matches a front projection with distinct shapes. \newline
% Candidate1 seems valid from a top-down view with different boxes and shapes, including a striped rectangle, central box, and large square. This arrangement is probably correct for interpreting the top view. \newline
% Determining invalid side between views \newline
% Candidate0 and Candidate2 show two side orthographic views. To figure out which side is invalid, I'll look at the relationships in perspective images. From the perspective views, it looks like the striped cylinder (G) is separated from the cluster in Candidate1, but not in Candidate0, where the rectangle is integrated. \newline
% Candidate0 doesn't show a separate \newline
% Considering cylinder and object separation \newline
% It looks like some objects might not be physically connected, but instead, they could be separated in depth. Candidate0 shows a separated cylinder superimposed on the cluster, which seems plausible. In Candidate1, the striped objects are separated, but there's no smooth cylinder visible. Candidate2 suggests the striped cylinder could appear as an ellipse, aligning well with the top view. It seems like Candidate0 and 2 might represent different orientations of the same cylinder. I'll need to determine the actual object heights to confirm which view fits. \newline
% Exploring smooth central object perspective \newline
% The smooth central object might be a cylinder or sphere, but its exact shape is unclear. In q1, part of it appears as a curved surface under the central cube, hidden at both the top and bottom by other objects. Projected views show ovals instead of rectangles, suggesting it could be a sphere. Candidates0 and 2 show different views of this shape as tall and horizontal ovals, respectively. Candidate1 doesn't show it, likely due to overlap with the central cube. \newline
% Validating perspectives based on cube locations \newline
% In q1, I notice that the small cube is actually centered under the central cube, not to its left. In a top view, this perspective distortion makes sense. For Candidate1, the striped cylinder and attached stripe seem correctly placed in relation to other objects. Candidate2's bottom row of boxes is interesting --- I'm checking if they align in an orthographic projection, with possible alignment along the top. \newline
% Validating projections and arrangement in Candidate2 \newline
% In Candidate2, the bottom row appears to have objects at similar vertical levels: a separated cylinder/ellipsoid on the left, followed by boxes. The striped object is above the boxes, which could match a y-projection where depth overlaps horizontally. The striped wedge in q1 could be placed under the central cube, not above it. Also, the striped rectangle's rise suggests it could be a horizontal striped cylinder viewed from above, not vertically. So, if it's top-down, this candidate doesn't fit. \newline
% Examining candidate2's projection and orientation \newline
% I initially thought candidate2's striped rectangle was on top of the right rectangle, but now I think it's actually behind in the ground plane if it's a top-down view. The ellipse on the left likely represents a smooth cylinder's footprint, and the striped rectangle could be the footprint of a cylindrical or rectangular object. The upright orientation in these projections isn't clear---it could be arbitrary, with vertical axes not strictly being up. \newline
% Considering projections and candidate orientations \newline
% I can't rely on the ``on top'' assumption anymore. So, I'm thinking of using projective geometry. Based on the two different perspectives, the candidates look like different projections along coordinate axes, probably top, side, and front. I think Candidate1 is a top projection with rectangular footprints, while Candidate0 and Candidate2 come from the side. In q2's perspective, the isolated cuboid on the right in Candidate1 seems to map to C, but Candidate2 doesn't have that isolated rectangle. \newline
% Considering object sizes and overlap in projections \newline
% There are two main components: the separate ellipse and the row with the stripe. Given the projections, overlapping objects make it tricky. I'm thinking of using object sizes for comparison. In the perspective images, the small and left cubes seem the same size as the central cube. In Candidate0, the thin top rectangle on the left box might make sense viewed from the side. But in Candidate2, the narrow middle rectangle looks off, possibly due to the central object's width distorting the side projection. \newline
% Analyzing silhouettes and perspective views \newline
% Looking at the likely silhouettes: Candidate0 has a smooth oval above the main cluster, which could be a sphere or ellipsoid. In q1, I see a partial cylinder behind the central cube, which could project as an oval from one view. Candidate2 shows a lower, horizontally oriented ellipse---if it's the same object, it could be valid from different viewpoints. As for Candidate1, it seems like the ellipse is missing because it could overlap with nearby boxes. Candidate0's top-left small box might be a thin rectangle, but there's no slab like that in the scene. The top-left large object in q2 appears as a thin rectangle if it's mostly hidden behind the lower cube. \newline
% Analyzing object positions in top view and side projection \newline
% Let's evaluate Candidate1's top view. We have several objects: a striped rectangle (L), cubes B and D, the central object A, another striped (H), and cuboid C. A and B aren't directly touching, but they're nearly adjacent. H touches A, while D and C are separate. In Candidate2's main row, these objects align well along their x-extends, suggesting Candidate2 is a projection along the y-axis, matching the x-axis alignment of Candidate1. \newline
% Analyzing alignment and perspective consistency \newline
% It seems Candidate0's bottom striped rectangle (x118-197) may not have the same scale or orientation. The top square (y31-84) may relate to the oval (x122-188), though that's uncertain. Upon comparing Candidate1 and Candidate2, their positions align well horizontally, suggesting both belong, and Candidate0 appears inconsistent. I need to verify whether Candidate0 shares vertical coordinates with Candidate1, and check for perspective alignment discrepancies. \newline
% Comparing projections and validity \newline
% In side projections, Candidate0 and Candidate2 both seem to show vertical height, but their orientation and positioning differ. C0 has a smooth oval high and striped rectangle low, while C2 has an ellipse low and striped rectangle high. The alignment between Candidate1 and Candidate2 is strong, but it's challenging. It's possible Candidate1 is valid while Candidate2 isn't, or perhaps Candidate0 and Candidate1 could align with a different axis. Further comparison with query helps clarify shapes, especially regarding the cylinder's appearance. \newline
% Considering the mutated candidate \newline
% The prompt indicates one invalid candidate, and I need to determine which might have been mutated. The alignment between C1 and C2 suggests they stem from the same model, but it's possible C0 was changed due to movements of the cylinder or ellipse. Examining the components of Candidate0 alongside C1 and C2, the top-left small shape with slab, central section, and bottom striped rectangle are all being assessed based \newline
% Evaluating candidate projections \newline
% It seems that Candidate0 lacks the smaller cube/cuboid at y180-234 because it overlaps with the central object. However, if Candidate0 features a smooth cylinder around y102-166, it might still work as a valid side projection. If all candidates are viewed from different axes, they might all be valid. I need to compare with query images, though, to detect any subtle differences in positioning, especially with the smooth oval/striped object. Let me check for a tall smooth oval in the perspective images. \newline
% Refining object placement and projections \newline
% I see a curved gray object behind the central and small cubes, but it's not tall above; it might be a cap of a horizontal cylinder. Candidate0's tall oval at the top could be the cylinder's cap viewed along its axis, not an independent object. Candidate2's oval fits better as part of the striped cylinder's circular cap. In the query image, the striped cylinder is separated, and depending on its position, its projection could appear above the cluster, not low. \newline
% Refining object placement and potential overlaps \newline
% In the top view of C1, the separated cylinder overlaps or sits above the central cluster in the y-coordinate, not at the bottom. In the perspective view, it appears at the bottom-left due to the camera angle. Candidate0's side projection suggests the cylinder's position aligns with the bottom striped rectangle, not the oval. The smooth oval might be another cylinder or ellipsoid, but it's possible Candidate2's left ellipse is simply the cylinder's circular cap, not a separate object. \newline
% Identifying potential object variation in scene \newline
% It looks like Candidate2 uses an ellipse for the striped cylinder, while Candidate0 uses a striped rectangle. That means Candidate0's oval is likely a different object. The scene could have another smooth cylinder, possibly hidden in other views. If the smooth oval isn't valid, it could be a mutation, and the curved arc in q1 might actually be a side face of an object rather than a cylinder. I'll take a closer look at q1's central curved area. \newline
% Finalizing object identification in projections \newline
% In q1, I noticed the arc that resembles a vertical oval side, which fits the pattern of a smooth oval. The arc is visible behind the rectangular prism and cubes, with its bottom and top hidden. Candidate0's oval matches this shape but is positioned differently due to the projection, while Candidate2's left ellipse could belong to this same oval. The left striped rectangle in Candidate1 might be the striped cylinder viewed from the side. \newline
% Identifying objects in each candidate view \newline
% In Candidate2, the left ellipse might be a smooth oval or a separated object. For Candidate1, the left striped rectangle could be a smooth or striped cylinder, while the right one might be a striped wedge or slab. Candidate0 shows a smooth oval at the top, a striped rectangle at the bottom, and several gray boxes. Each candidate represents 5 or 6 objects, with some potential overlap. We should compare the number and positions of these objects across views. \newline
% Analyzing candidates for object arrangement \newline
% Original scene has at least four cuboids: left/top, central, right, and bottom. In side projection, these can collapse into two groups due to alignment. Candidate2 shows three boxes and a top stripe, with no separate box on top or back. In Candidate1, all boxes are accounted for. Candidate0 might have an issue, as the oval sits too high and doesn't overlap the central cube. Although, it might still be valid, so I'll check the line/occlusion evidence. In query 1, the smooth oval sits between the central and bottom cubes, partially visible but not taller than the central ones; its top is hidden under the central cube, and its bottom is hidden by the bottom cube. Candidate0 shows the oval above the central \newline
% Considering candidate consistency for vertical alignment \newline
% If candidate2's smooth oval is the same object as in candidate0, it should have similar height, assuming they share the same vertical axis. But if candidates are orthographic views, the vertical alignment could vary. Candidate0's and candidate2's positions clearly differ, making it unlikely they're the same object. \newline
% Revisiting the smooth oval object vs. striped cylinder \newline
% If candidate2's ellipse isn't the smooth oval but rather a striped cylinder cap, that could explain the difference in appearance. The striped cylinder may appear in candidate0 as a bottom stripe and in C2 as a top one, but this would be inconsistent. The ellipse could represent the striped cylinder's cap, not the smooth oval. \newline
% Expressing geometric inference for world axis mapping \newline
% I'm thinking of using geometric inference to compute possible orthographic projections from perspective views. These views seem to be isometric, so I can define world axes (x, y, z). With this in mind, I'll be able to infer 3D coordinates, combining q1 and q2 to identify object positions in the world grid. \newline
% Using q1 basis for coordinate differences \newline
I'm using q1's isometric setup with vectors u = (61,49) and v = (-59,51). Ground objects have a height of 1, with their top face appearing at z=1. The central cube's top center is at (245,93), so for cube B, the top center seems to be around (143,86). The difference is (-102,-7), and I need to solve for this horizontal difference in terms of the u/v basis. \newline
Inferring object positions from isometric projections \newline
\tann{annCol9}{import numpy as np u=np.array([61,49.]) v=np.array([-59,51.]) M=np.column\_stack([u,v]) diff=np.array([-102,-7.]) np.linalg.solve(M,diff) array([-0.93552149, 0.76157947])}{Tool Use} \newline
Determining position of cuboid C relative to A \newline
Cube B seems to be approximately at (-1, +1) relative to A. For cuboid C, the top center appears to be around (354, 134), based on the parallelogram's corners (319,126; 354,94; 392,134; 356,166). The difference between C and A is (110, 37), so I'll need to solve for that. \newline
Solving for transformation matrix \newline
\tann{annCol9}{diff=np.array([110,37.]) np.linalg.solve(M,diff) array([ 1.29840053, -0.52199267])}{Tool Use} \newline
Determining position of cube D relative to right cuboid \newline
The right cuboid is at (+1.3, -0.5), and the small bottom cube D has a top center at (233, 235), with corners at (232, 191), (282, 235), (234, 279), and (185, 236). The difference between cuboid D's position and the right cuboid is (-12, 142). I'll need to solve for that. \newline
Solving linear system with given difference vector \newline
\tann{annCol9}{diff=np.array([-12,142.]) np.linalg.solve(M,diff) array([1.29390203, 1.54115295])}{Tool Use} \newline
Analyzing position relationships and projections \newline
Candidate 1's top view shows relative positions: B is upper-left, C lower-right, D lower-left, cylinder on the left, and stripe on the right. However, the positions don't match perfectly with the q1 estimate, possibly due to scale or rotation. By comparing q1 and q2, I can infer whether candidate 0 or 2 fits better. \newline
\textit{[[...trimmed output...]]} \newline
% Analyzing cylinder stripe projections and candidate confusion \newline
% The cylinder's projection can vary in different views --- as a rectangle with vertical stripes, a rectangle with horizontal stripes, or potentially an ellipse. The stripes' orientation depends on the projection's angle. There's confusion around whether the striped pattern belongs to the cylinder or a separate slab, especially in candidate views. \newline
% Identifying stripe patterns based on projections \newline
% Candidate1 has a left stripe with vertical lines, and the right stripe seems to show horizontal lines. The central striped object probably has horizontal stripes in candidates 0, 1, and 2. The separated cylinder in candidate1 likely has vertical stripes or may appear as an ellipse in candidate2. The smooth oval in candidate0 could be an end-on view of a cylinder. \newline
% Analyzing cylinder and central object positions \newline
% The central striped object in q2 looks like it has a striped side and maybe a triangular or curved edge, which could match the end of a cylinder. There may be two cylinders: one partially hidden and one separate. Candidate0 might show the central cylinder with an oval cap above and a striped rectangle below. However, a single cylinder wouldn't show both a cap and sides in the same view, unless it's an oblique perspective. \newline
% Considering object layers and projections \newline
% The prompt calls for silhouettes, but the candidates show interior lines and stripes, not pure silhouettes. These are orthographic views with visible faces and patterns, and some occlusion. Candidate0 shows both a cylinder cap and side, but the oval cap and striped side aren't attached. This suggests two separate objects or layers, especially since the smooth oval and striped rectangles in candidate0 and candidate2 are disconnected. \newline
% Evaluating cylinder positioning and overlap \newline
% In the perspective query, the separated striped cylinder is shown at opposite locations in q1 and q2---far left and far right of the cluster, respectively. This makes sense for candidate1 and candidate2. However, candidate0 shows an overlap between the cylinder's bottom stripe and the cluster, which may be suspicious. This suggests the cylinder isn't collinear with the cluster, but the overlapping presence might be a result of depth or projection perspective. \newline
% Evaluating candidate alignments and overlaps \newline
Candidate0's overlap with the central cluster might be possible if projected along the orthogonal axis. From two oblique views, a cylinder could align here. Candidate0's smooth oval above the central cluster fits, and the separated ellipse in candidate2 is plausible. I'll check the consistency between candidates' coordinates for further validation.

``` \newline
\{ \newline
\tann{annCol10}{'candidate\_idx': 0,}{Wrong Perception} \newline
\} \newline
```
\end{tcolorbox}
\begin{tcolorbox}[breakable,enhanced,colback=red!4,colframe=red!55!black,boxrule=0.4pt,arc=1pt,left=4pt,right=4pt,top=3pt,bottom=3pt,fonttitle=\footnotesize\bfseries,coltitle=black,colbacktitle=red!12,title={\tpicon{gemini_flash_icon.png}~Gemini-3-Flash\hfill answer: 2\tickno}]
\footnotesize\raggedright
To identify the invalid silhouette, we must analyze the spatial arrangement of the objects in the 3D scene from the two perspective views provided.

\#\#\# Scene Analysis

The scene consists of two main clusters of objects:

1. **Cylinder Cluster:** Three cylinders oriented horizontally. One acts as a base, with two others positioned around or on it. \newline
2. **Box Cluster:** Three boxes of varying sizes. One large box serves as a base, with two smaller boxes placed on top or adjacent to it.

\#\#\# Silhouette Evaluation

* **Candidate 0:** This silhouette represents a **top-down (plan) view**. It shows the circular profiles of the three cylinders (represented by the hatched squares/rectangles since they are viewed top-down) and the square profiles of the three boxes. Their relative positions match the logic of \tann{annCol10}{the 3D scene. * **Candidate 1:** This silhouette represents a **side elevation**. It correctly captures the circular faces of two cylinders and the side profile of the third, along with the rectangular profiles of the boxes. The overlap and stacking order align with the perspective images. * **Candidate 2:** This silhouette contains a significant inconsistency. It shows an arrangement where the boxes and cylinders are overlapping in a way that suggests a different spatial relationship than the one shown in the perspective views. Specifically, the alignment of the box profiles relative to the cylinder profiles does not match the 3D layout, indicating it was generated from a mutated version of the scene where objects were shifted or resized. Based on this analysis, the invalid silhouette is Candidate 2.}{Wrong Perception}

```json \newline
\{ \newline
"candidate\_idx": 2 \newline
\}

```
\end{tcolorbox}
\begin{tcolorbox}[breakable,enhanced,colback=green!4,colframe=green!50!black,boxrule=0.4pt,arc=1pt,left=4pt,right=4pt,top=3pt,bottom=3pt,fonttitle=\footnotesize\bfseries,coltitle=black,colbacktitle=green!14,title={\tpicon{gemini_pro_icon.png}~Gemini-3.1-Pro\hfill answer: 1\tickok}]
\footnotesize\raggedright
Defining the Scene

I am now identifying objects and positions within the two perspective images, focusing on two main clusters.

Analyzing the Cube Setup

I've established a coordinate system and cube grid: (0,0), (1,0), (0,1), and (0,0,1), but now need to reconcile the horizontal cylinders' positions.

Orienting the Cylinders

I am now visualizing object alignment to X, Y, Z axes, considering multiple image perspectives.

\textit{[[...trimmed output...]]}

% Revising Cube Arrangement

% I've discarded the initial layout, now experimenting with an L-shape base with one cube on top.

% Refining Cube Positions

% I've precisely defined cube positions: L-shape base at (0,0), (+1,0), (0,-1), cross-referencing with images and confirming cylinder attachments.

% Visualizing Top View

% I'm now identifying a 2x2 cube layout in the top view and precisely mapping the stack configuration.

% Reassessing Cube Grid

% I'm now re-evaluating the cube grid's perfection based on discrepancies observed in the images.

% Interpreting Cylinder Views

% I've just confirmed the correspondence of cylinder stripe direction to their axes in the top-down view, cross-referencing this data.

% Confirming Image Correspondence

% I've just confirmed correspondence between camera views, now analyzing discrepancies in cube sizes within the scene.

% Clarifying Block Sizes

% I'm now identifying that the scene involves a larger 2x2x2 block with a 2-high small block stack, and a ground-level single small box.

% Confirming Object Alignment

% Now I have confirmed alignment through the images, cross-referencing cube and stack positions across all viewpoints.

% Defining Cube Boundaries

% I've just defined coordinates and confirmed an offset for small boxes relative to the large one and each other.

% Validating Spatial Relations

% I'm now cross-referencing all views, verifying cylinder stripe orientations and their positions within the scene.

% Clarifying Top Object

% I'm now identifying that the object atop the middle stack is a cube, not a cylinder, per multiple image views.

% Mapping Cylinder Alignment

% I am now carefully mapping cylinders, identifying their alignment in candidate views, and checking their striped faces.

% Re-evaluating Axis Directions

% I'm now identifying cylinder stripe directions to confirm axes, cross-referencing this to cube edge alignment across viewpoints.

% Confirming Axis Correlation

% I have just confirmed X and Y cylinder alignments in the top view via stripe orientation matches.

% Verifying Cylinder Alignment

% I've just confirmed cylinder alignments with their stripe directions in the image viewpoints, checking their coordinates.

% Analyzing Cylinder Axes

% I've determined cylinders are not parallel to Y, their stripes now confirming X axis alignment per top image view.

% Confirming Axis Perspectives

% I've just confirmed axis alignment across viewpoints, now mapping cylinder orientations relative to each other within scenes.

% Refining Axis Alignment

% I have just confirmed the three cylinders are aligned to X-axis in query image one, checking stripe orientations.

% Confirming Y Alignment

% I have just confirmed the middle cylinder in both images is parallel to Y, via stripe and view analysis.

% Mapping Cylinder Arrangement

% I am now confirming the candidate matches the image setup, especially in cylindrical and block arrangements.

% Verifying Spatial Positions

% I am now verifying the candidate cylinder positions against both images, especially along X and Y axes, ensuring stripe orientations match image views.

% Verifying Image Correspondence

% I'm now cross-referencing all data, and just confirmed Candidate 0 aligns to the scenes, image-wise.

% Interpreting Candidate Views

% I've just deduced that Candidate 2 represents a front view due to the single circular cylinder representation, which aligns with cylinder positioning.

% Interpreting Candidate Cubes

% I am now visualizing the cubes from the front view, and have just validated the front-view hypothesis.

% Assessing Image Heights

% I'm now identifying relative object heights within images, and am considering cylinder tilt in relation to the cube setup.

% Analyzing Cylinder Planes

% I've just determined Candidate 1's ellipses indicate a non-axis-aligned view, potentially rendering it invalid.

% Clarifying Orthogonality

% I've just confirmed the cylinders' orthogonal alignment; stripes confirm axis directions, resolving the Candidate 1's elliptical faces.

% Rejecting Inconsistent Views

% I've just rejected Candidate 1 due to geometric inconsistencies between cube and cylinder representations.

% Validating Candidate Views

% I'm now determining Candidate 1 contains elliptical cylinders, and Candidate 0 aligns perfectly to the scenes.

% Revising Image Alignment

% I have just confirmed Candidate 0 aligns to query image one, identifying block stack positioning and cylinder overlap, specifically the Middle and Y-cyl components.

% Revising Stack Alignment

% I'm now determining the Y-cylinder's overlap in Candidate 0 doesn't match the 2-high stack, re-evaluating the top-left stack as a match.

% Revising View Perspectives

% I'm now determining Candidate 0 isn't front view due to cylinder direction mismatch, re-evaluating perspective interpretations.

% Confirming Viewpoint Validation

% I've just confirmed that Candidate 0, the top view, correctly renders the cube on the 2-high stack and re-evaluated others.

% Interpreting Front Views

% I'm now concluding the Candidate 2 front view configuration: large box right, stack left, small box in front overlapping stack's base.

% Revising Image Analyses

% I'm now concluding that the front view interpretation of Candidate 2 must be revisited, given new shape analyses, since Y-cylinder overlaps are visible.

% Analyzing Cylinder Shape

% I've just confirmed the elliptical cylinder shape definitively invalidates Candidate 1, which now has ovals wider than they are tall.

% Validating Shape Analyses

% I have just confirmed the lack of angled cuts, determining the elliptical shape definitively invalidates Candidate 1.

% Validating Scene Alignment

% I have just confirmed Candidate 2 as the front view, with cube and cylinder alignment matching image data based on shape analyses.

% Revising Candidate Views

% I am now re-evaluating candidate front views to align with scene data, particularly cylinder shapes in images, confirming stripe correspondence.

% Validating Elliptical Views

% I have just validated the shape analyses, confirming Candidate 1 presents a view from the -X axis.

% Confirming Cylinder Shapes

% I've just validated that the ellipses in Candidate 1 definitively contradict circular cylinders, rendering it invalid per axis-aligned views.

% Revising Stack Heights

% I've just determined Candidate 2 places the large box atop the small one, contrary to query image evidence, now re-evaluating layout.

% Revising Candidate Shapes

% I have just confirmed Candidate 2 cannot be a front view because the "large square" sits above the rest of the boxes, contradicting ground alignment.

% Validating Cube Alignments

% I've just validated a side view for Candidate 1 based on stripe orientations and re-assessed Candidate 2's potential front view.

% Revising Shape Hypotheses

% I've just concluded Candidate 2 cannot depict a side view due to inconsistencies, re-evaluating shape representations and cylinder axes.

% Interpreting Candidate Views

% I've just validated Candidate 2 represents a side view with a 2-cube stacked arrangement, aligning precisely with image data.

% Validating Side Views

% I'm now certain Candidate 2 is a side view with a stacked box arrangement, validating stripe orientations.

% Revising Object Shapes

% I am now re-evaluating shape interpretations, now wondering if boxes are actually multiple joined, and if cylinders are misidentified.

% Revising Shape Analyses

% I'm now determining Candidate 0 is likely the correct top-down view, with the cylinders horizontal.

% Validating Scene Views

% I have just confirmed Candidate 0's stripe orientations and found the middle cylinder's perpendicular alignment, thus validating the top view.

Revising Candidate Views

I am now re-evaluating each candidate's validity, since Candidate 1 presents ovals that don't overlap as cylindrical projections.

Refining Perspective Analyses

\tann{annCol3}{I have just confirmed Candidate 1's invalidity due to cylinder overlap inconsistencies, thus validating Candidate 2's front-view nature.}{Good Perception}

Validating Image Alignment

\tann{annCol3}{I have just confirmed the perfectly axis-aligned cylinders validate the top view in Candidate 0, invalidating Candidate 1.}{Good Perception}

Analyzing Elliptical Shapes

\tann{annCol3}{I am now thoroughly analyzing elliptical projections in Candidate 1, precisely confirming that axis-aligned cylinders cannot produce these images, due to overlapping in the side view.}{Good Perception}

Validating Scene Components

\tann{annCol10}{I have just confirmed Candidate 2's invalidity due to missing cylinders, contradicting cylindrical object representations across image data.}{Wrong Perception}

Validating Object Placement

I've just pinpointed inconsistencies in Candidate 2's cylinder height, finding it invalid based on image data.

Confirming Image Analyses

\tann{annCol3}{I have just confirmed Candidate 1 is invalid, due to shape inconsistencies, now cross-validating the remaining views.}{Good Perception}

Validating Invalid Silhouette

\tann{annCol3}{I am now confident Candidate 1, with elliptical cylinder shapes and inconsistent projection, is the mutated scene's invalid silhouette.}{Good Perception}

```json \newline
\{ \newline
"candidate\_idx": 1 \newline
\}

```
\end{tcolorbox}
